# Supplementary material for: Generators and relations for n-qubit Clifford operators
Source: arXiv:1310.6813 ancillary file (2017-03-29)

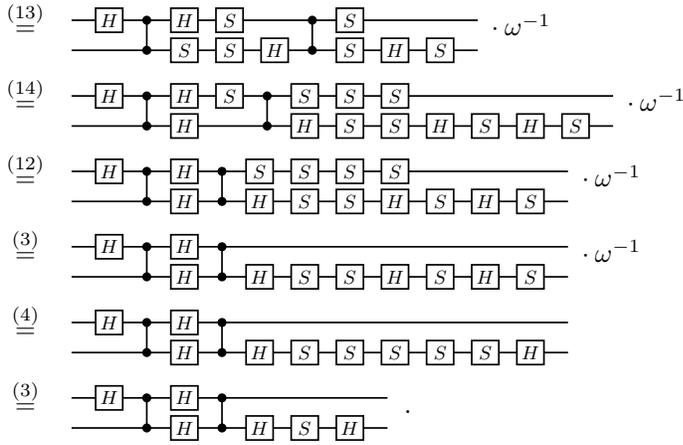

For (17), we have

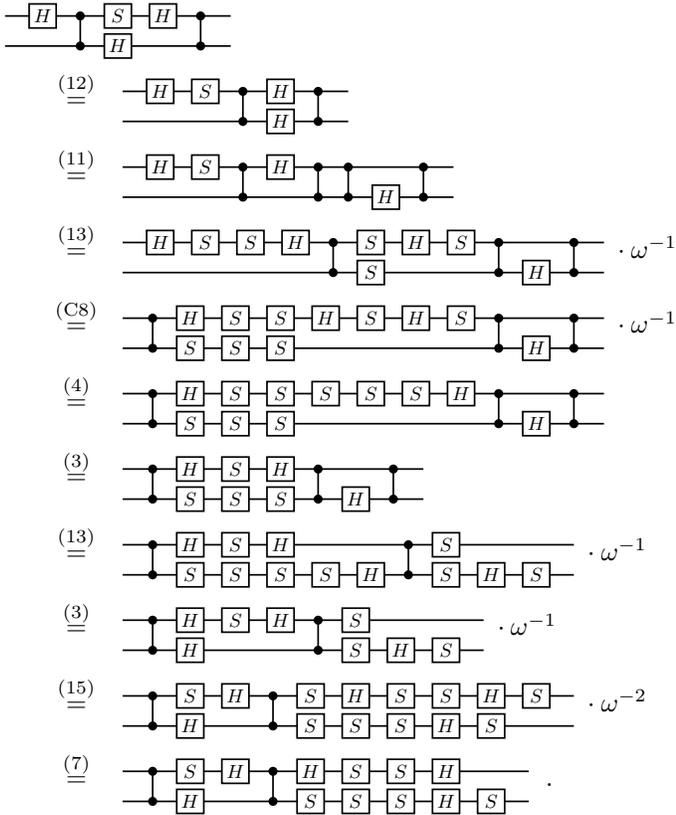

For (18), we have

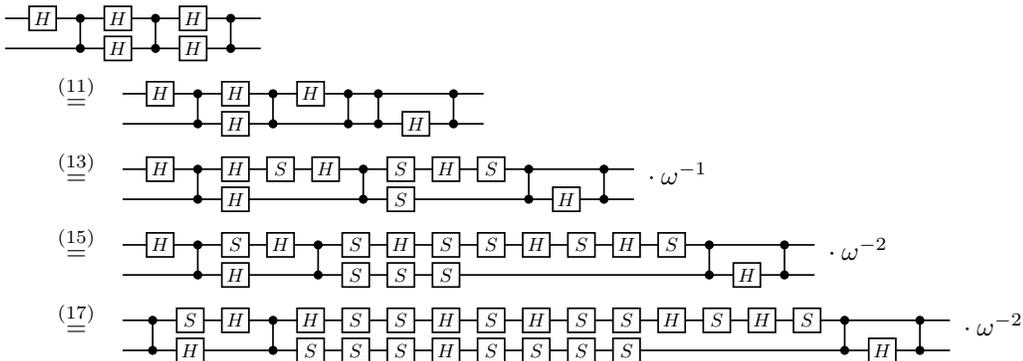



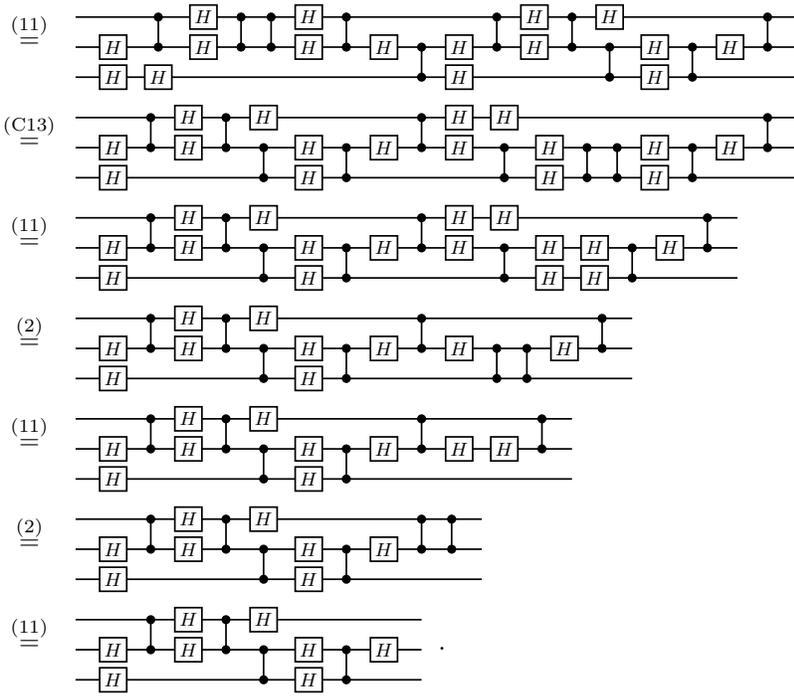

For (21), we have

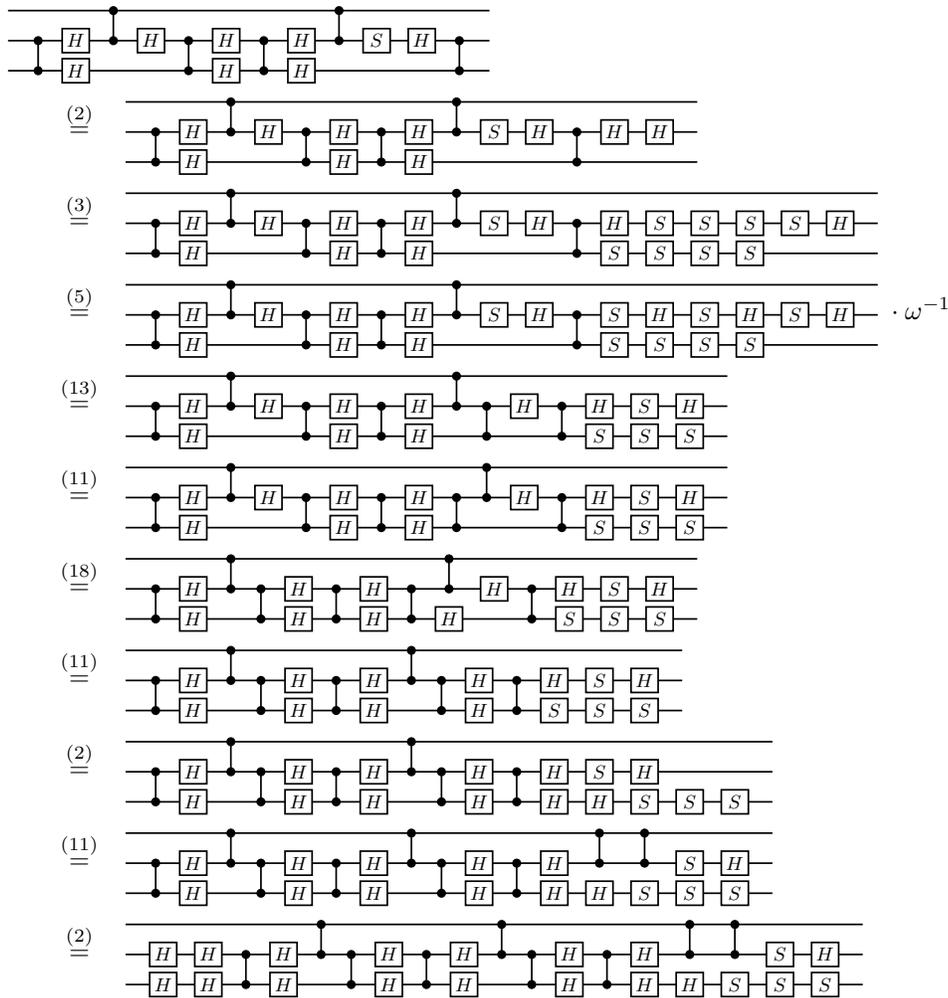

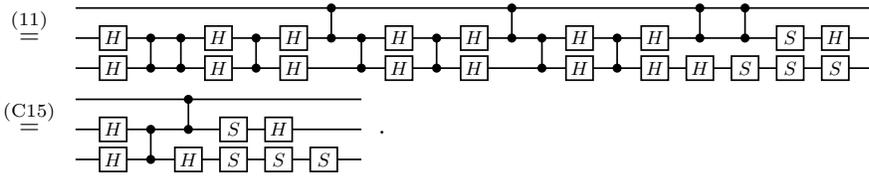

□

### 3 Proofs of the equations from Proposition 7.1

In the following proofs, we write (inv) to denote some number of application of the properties (2), (3), and (11), usually to insert or delete a circuit together with its own inverse inside a larger circuit. We write (def) to denote a definition from Figure 1.

#### 3.1 Equation

$$\text{---} = \text{---} \boxed{A_1} \boxed{C_1} \boxed{E_1} \text{---}$$

**Proof:**  $\text{---}$   
 $\stackrel{\text{(def)}}{=} \text{---}$   
 $\stackrel{\text{(def)}}{=} \text{---} \boxed{A_1} \boxed{C_1} \boxed{E_1} \text{---}$

#### 3.2 Equation

$$\text{---} \boxed{C_1} \text{---} = \text{---} \boxed{B_1} \boxed{C_1} \boxed{D_1} \text{---}$$

**Proof:**  $\text{---} \boxed{C_1} \text{---}$   
 $\stackrel{\text{(def)}}{=} \text{---}$   
 $\stackrel{\text{(2)}}{=} \text{---} \boxed{H} \boxed{H} \text{---}$   
 $\stackrel{\text{(11)}}{=} \text{---} \boxed{H} \boxed{H} \text{---}$   
 $\stackrel{\text{(2)}}{=} \text{---} \boxed{H} \boxed{H} \boxed{H} \boxed{H} \text{---}$   
 $\stackrel{\text{(2)}}{=} \text{---} \boxed{H} \boxed{H} \boxed{H} \boxed{H} \boxed{H} \boxed{H} \text{---}$   
 $\stackrel{\text{(11)}}{=} \text{---} \boxed{H} \boxed{H} \boxed{H} \boxed{H} \boxed{H} \boxed{H} \boxed{H} \boxed{H} \text{---}$   
 $\stackrel{\text{(2)}}{=} \text{---} \boxed{H} \boxed{H} \boxed{H} \boxed{H} \boxed{H} \boxed{H} \boxed{H} \boxed{H} \boxed{H} \boxed{H} \text{---}$   
 $\stackrel{\text{(2)}}{=} \text{---} \boxed{H} \boxed{H} \boxed{H} \boxed{H} \boxed{H} \boxed{H} \boxed{H} \boxed{H} \boxed{H} \boxed{H} \boxed{H} \text{---}$   
 $\stackrel{\text{(11)}}{=} \text{---} \boxed{H} \boxed{H} \boxed{H} \boxed{H} \boxed{H} \boxed{H} \boxed{H} \boxed{H} \boxed{H} \boxed{H} \boxed{H} \text{---}$   
 $\stackrel{\text{(def)}}{=} \text{---} \boxed{B_1} \boxed{C_1} \boxed{D_1} \text{---}$

#### 3.3 Equation

$$\text{---} \boxed{H} \boxed{A_1} \text{---} = \text{---} \boxed{A_2} \text{---}$$

**Proof:**  $\text{---} \boxed{H} \boxed{A_1} \text{---}$   
 $\stackrel{\text{(def)}}{=} \text{---} \boxed{H} \text{---}$   
 $\stackrel{\text{(def)}}{=} \text{---} \boxed{A_2} \text{---}$

#### 3.4 Equation

$$\text{---} \boxed{H} \boxed{A_2} \text{---} = \text{---} \boxed{A_1} \text{---}$$

**Proof:**  $\text{---} \boxed{H} \boxed{A_2} \text{---}$   
 $\stackrel{\text{(def)}}{=} \text{---} \boxed{H} \boxed{H} \text{---}$   
 $\stackrel{\text{(2)}}{=} \text{---}$   
 $\stackrel{\text{(def)}}{=} \text{---} \boxed{A_1} \text{---}$

### 3.5 Equation

$$\boxed{H} \boxed{A_3} = \boxed{A_3} \boxed{X} \boxed{S} \boxed{S} \boxed{S} \cdot \omega$$

**Proof:**

$$\begin{aligned} & \boxed{H} \boxed{A_3} \\ \stackrel{(\text{def})}{=} & \boxed{H} \boxed{H} \boxed{S} \boxed{H} \\ \stackrel{(2)}{=} & \boxed{S} \boxed{H} \\ \stackrel{(3)}{=} & \boxed{S} \boxed{H} \boxed{S} \boxed{S} \boxed{S} \boxed{S} \\ \stackrel{(6)}{=} & \boxed{H} \boxed{S} \boxed{S} \boxed{S} \boxed{H} \boxed{S} \boxed{S} \boxed{S} \cdot \omega \\ \stackrel{(2)}{=} & \boxed{H} \boxed{S} \boxed{H} \boxed{H} \boxed{S} \boxed{S} \boxed{H} \boxed{S} \boxed{S} \boxed{S} \cdot \omega \\ \stackrel{(\text{def})}{=} & \boxed{A_3} \boxed{X} \boxed{S} \boxed{S} \boxed{S} \cdot \omega \end{aligned}$$

### 3.6 Equation

$$\boxed{S} \boxed{A_1} = \boxed{A_1} \boxed{S}$$

**Proof:**

$$\begin{aligned} & \boxed{S} \boxed{A_1} \\ \stackrel{(\text{def})}{=} & \boxed{S} \\ \stackrel{(\text{def})}{=} & \boxed{A_1} \boxed{S} \end{aligned}$$

### 3.7 Equation

$$\boxed{S} \boxed{A_2} = \boxed{A_3} \boxed{X} \boxed{S} \boxed{S} \boxed{S} \cdot \omega$$

**Proof:**

$$\begin{aligned} & \boxed{S} \boxed{A_2} \\ \stackrel{(\text{def})}{=} & \boxed{S} \boxed{H} \\ \stackrel{(3)}{=} & \boxed{S} \boxed{H} \boxed{S} \boxed{S} \boxed{S} \boxed{S} \\ \stackrel{(6)}{=} & \boxed{H} \boxed{S} \boxed{S} \boxed{S} \boxed{H} \boxed{S} \boxed{S} \boxed{S} \cdot \omega \\ \stackrel{(2)}{=} & \boxed{H} \boxed{S} \boxed{H} \boxed{H} \boxed{S} \boxed{S} \boxed{H} \boxed{S} \boxed{S} \boxed{S} \cdot \omega \\ \stackrel{(\text{def})}{=} & \boxed{A_3} \boxed{X} \boxed{S} \boxed{S} \boxed{S} \cdot \omega \end{aligned}$$

### 3.8 Equation

$$\boxed{S} \boxed{A_3} = \boxed{A_2} \boxed{S} \boxed{S} \boxed{S} \cdot \omega$$

**Proof:**

$$\begin{aligned} & \boxed{S} \boxed{A_3} \\ \stackrel{(\text{def})}{=} & \boxed{S} \boxed{H} \boxed{S} \boxed{H} \\ \stackrel{(5)}{=} & \boxed{H} \boxed{S} \boxed{S} \boxed{S} \cdot \omega \\ \stackrel{(\text{def})}{=} & \boxed{A_2} \boxed{S} \boxed{S} \boxed{S} \cdot \omega \end{aligned}$$

### 3.9 Equation

$$\begin{array}{c} \bullet \\ | \\ \boxed{A_1} \\ | \\ \bullet \\ \hline \end{array} = \begin{array}{c} \hline \bullet \\ | \\ \boxed{A_1} \\ | \\ \bullet \\ \hline \end{array}$$

**Proof:**

$$\begin{aligned} & \begin{array}{c} \bullet \\ | \\ \boxed{A_1} \\ | \\ \bullet \\ \hline \end{array} \\ \stackrel{(\text{def})}{=} & \begin{array}{c} \bullet \\ | \\ \bullet \\ \hline \end{array} \\ \stackrel{(\text{def})}{=} & \begin{array}{c} \hline \bullet \\ | \\ \boxed{A_1} \\ | \\ \bullet \\ \hline \end{array} \end{aligned}$$



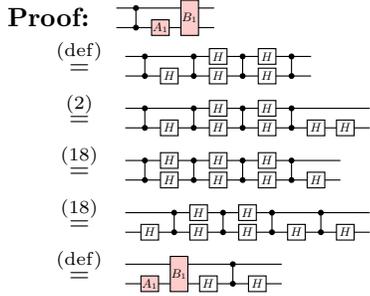

### 3.13 Equation

$$\text{Circuit with } A_1, B_2 = \text{Circuit with } A_2, H$$

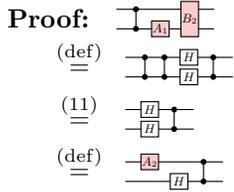

### 3.14 Equation

$$\text{Circuit with } A_1, B_3 = \text{Circuit with } A_3, H, S, H, S \cdot \omega^7$$

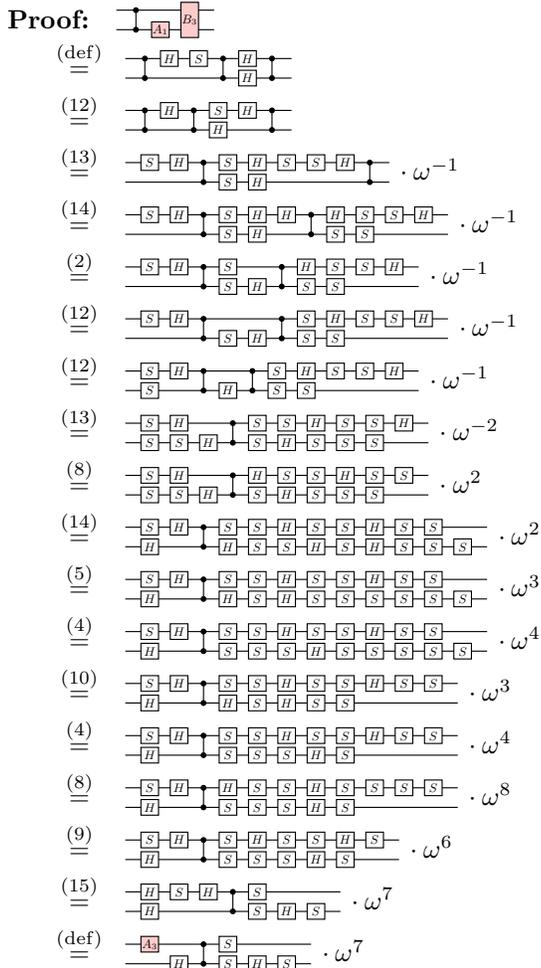

### 3.15 Equation

**Proof:**

### 3.16 Equation

**Proof:**

### 3.17 Equation

**Proof:**

(def)  $\equiv$

(13)  $\equiv$   $\cdot \omega^{-1}$

(5)  $\equiv$

(12)  $\equiv$

(12)  $\equiv$

(12)  $\equiv$

(2)  $\equiv$

(3)  $\equiv$

(2)  $\equiv$

(14)  $\equiv$

(12)  $\equiv$

(3)  $\equiv$

(12)  $\equiv$

(12)  $\equiv$

(5)  $\equiv$   $\cdot \omega^{-1}$

(13)  $\equiv$

(12)  $\equiv$

(2)  $\equiv$

(3)  $\equiv$

(5)  $\equiv$   $\cdot \omega^{-1}$

(17)  $\equiv$   $\cdot \omega^{-1}$

(3)  $\equiv$   $\cdot \omega^{-1}$

(12)  $\equiv$   $\cdot \omega^{-1}$

(10)  $\equiv$

(4)  $\equiv$   $\cdot \omega^{-1}$

(5)  $\equiv$   $\cdot \omega^{-2}$

(14)  $\equiv$   $\cdot \omega^{-2}$

(12)  $\equiv$   $\cdot \omega^{-2}$

(3)  $\equiv$   $\cdot \omega^{-2}$

(12)  $\equiv$   $\cdot \omega^{-2}$

(12)  $\equiv$   $\cdot \omega^{-2}$

(6)  $\equiv$   $\cdot \omega^{-1}$

(2)  $\equiv$   $\cdot \omega^{-1}$

(5)  $\equiv$   $\cdot \omega^{-2}$



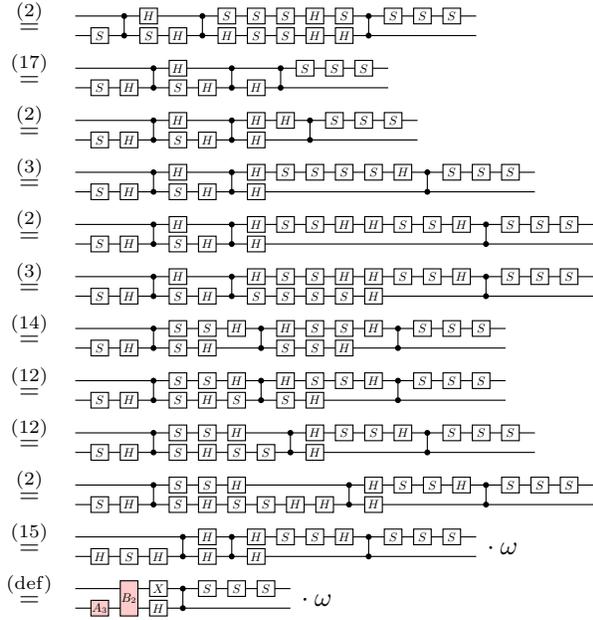

### 3.19 Equation

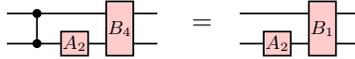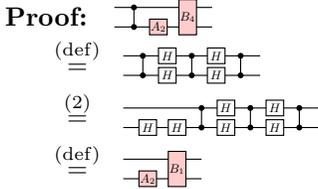

### 3.20 Equation

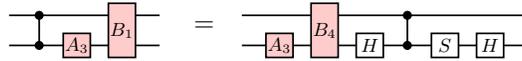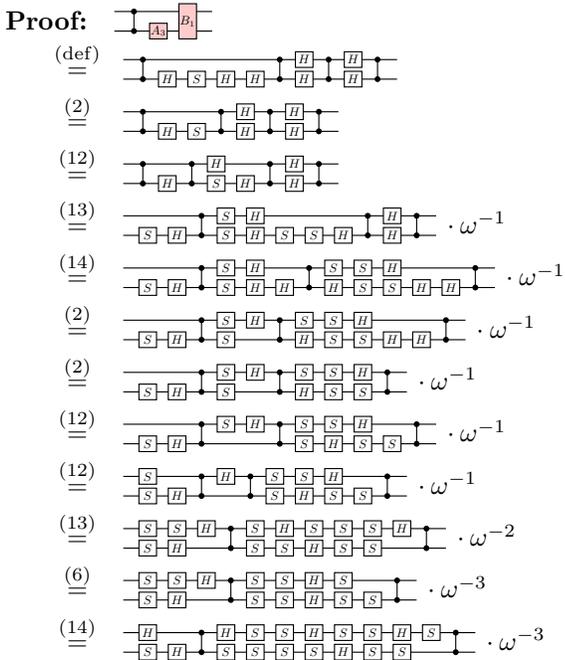





$$\begin{aligned}
& \stackrel{(12)}{=} \text{Diagram 1} \cdot \omega \\
& \stackrel{(2)}{=} \text{Diagram 2} \cdot \omega \\
& \stackrel{(3)}{=} \text{Diagram 3} \cdot \omega \\
& \stackrel{(2)}{=} \text{Diagram 4} \cdot \omega \\
& \stackrel{(17)}{=} \text{Diagram 5} \cdot \omega \\
& \stackrel{(12)}{=} \text{Diagram 6} \cdot \omega \\
& \stackrel{(\text{def})}{=} \text{Diagram 7} \cdot \omega
\end{aligned}$$

### 3.22 Equation

$$\text{Diagram 8} = \text{Diagram 9} \cdot \omega$$

**Proof:**

$$\begin{aligned}
& \stackrel{(\text{def})}{=} \text{Diagram 10} \\
& \stackrel{(12)}{=} \text{Diagram 11} \\
& \stackrel{(17)}{=} \text{Diagram 12} \\
& \stackrel{(15)}{=} \text{Diagram 13} \cdot \omega^{-1} \\
& \stackrel{(2)}{=} \text{Diagram 14} \cdot \omega^{-1} \\
& \stackrel{(14)}{=} \text{Diagram 15} \cdot \omega^{-1} \\
& \stackrel{(3)}{=} \text{Diagram 16} \cdot \omega^{-1} \\
& \stackrel{(2)}{=} \text{Diagram 17} \cdot \omega^{-1} \\
& \stackrel{(3)}{=} \text{Diagram 18} \cdot \omega^{-1} \\
& \stackrel{(2)}{=} \text{Diagram 19} \cdot \omega^{-1} \\
& \stackrel{(12)}{=} \text{Diagram 20} \cdot \omega^{-1} \\
& \stackrel{(13)}{=} \text{Diagram 21} \cdot \omega^{-2} \\
& \stackrel{(7)}{=} \text{Diagram 22} \\
& \stackrel{(14)}{=} \text{Diagram 23} \\
& \stackrel{(14)}{=} \text{Diagram 24} \\
& \stackrel{(2)}{=} \text{Diagram 25} \\
& \stackrel{(3)}{=} \text{Diagram 26} \\
& \stackrel{(2)}{=} \text{Diagram 27} \\
& \stackrel{(14)}{=} \text{Diagram 28} \\
& \stackrel{(3)}{=} \text{Diagram 29} \\
& \stackrel{(2)}{=} \text{Diagram 30} \\
& \stackrel{(3)}{=} \text{Diagram 31} \\
& \stackrel{(2)}{=} \text{Diagram 32} \\
& \stackrel{(12)}{=} \text{Diagram 33}
\end{aligned}$$



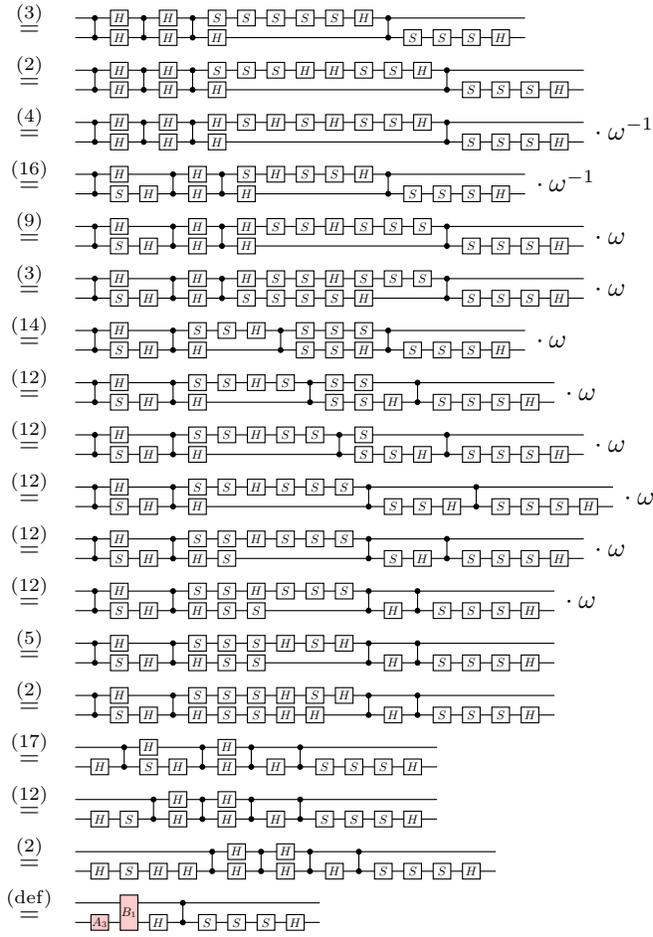

### 3.24 Equation

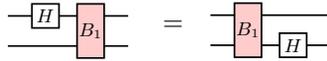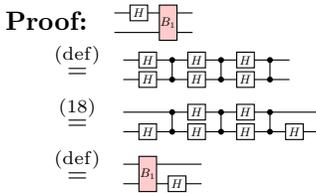

### 3.25 Equation

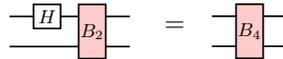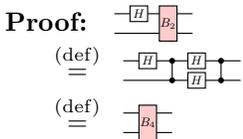

### 3.26 Equation

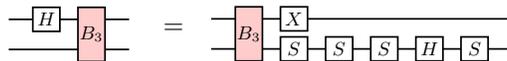

**Proof:**

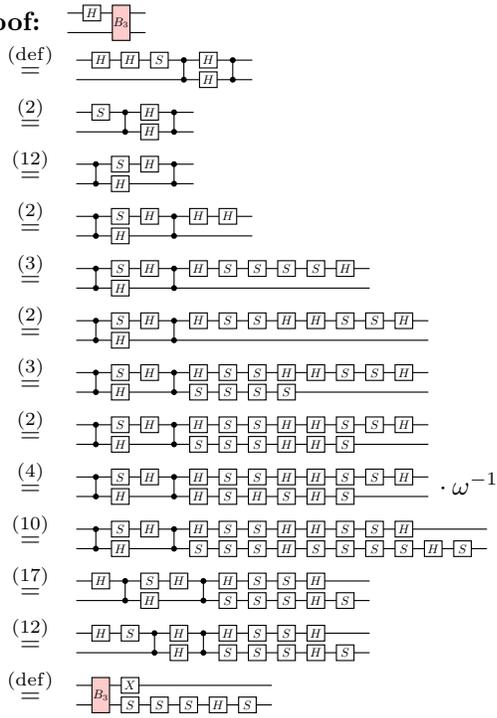

### 3.27 Equation

$$\begin{array}{c} \boxed{H} \\ \hline \boxed{B_4} \end{array} = \begin{array}{c} \boxed{B_2} \\ \hline \end{array}$$

**Proof:**

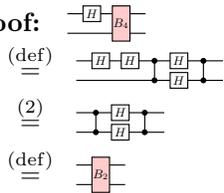

### 3.28 Equation

$$\begin{array}{c} \boxed{S} \\ \hline \boxed{B_1} \end{array} = \begin{array}{c} \boxed{B_1} \\ \hline \boxed{H} \boxed{S} \boxed{H} \end{array}$$

**Proof:**

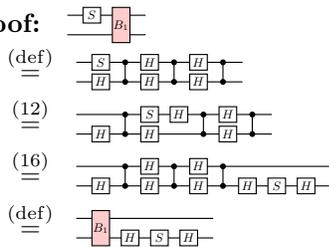

### 3.29 Equation

$$\begin{array}{c} \boxed{S} \\ \hline \boxed{B_2} \end{array} = \begin{array}{c} \boxed{B_3} \boxed{X} \\ \hline \boxed{S} \boxed{S} \boxed{S} \boxed{H} \boxed{S} \end{array}$$

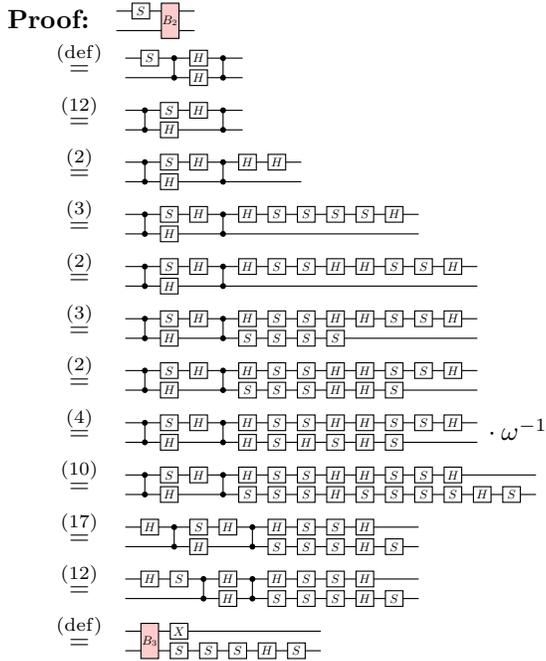

### 3.30 Equation

$$\begin{array}{c} \boxed{S} \\ \hline \boxed{B_3} \end{array} = \begin{array}{c} \boxed{B_2} \\ \hline \boxed{S} \boxed{H} \boxed{S} \end{array}$$

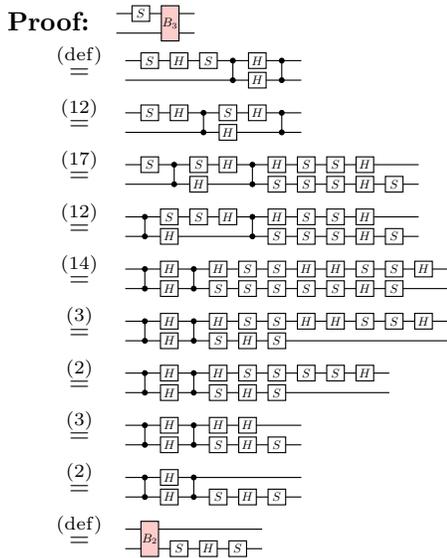

### 3.31 Equation

$$\begin{array}{c} \boxed{S} \\ \hline \boxed{B_4} \end{array} = \begin{array}{c} \boxed{B_4} \\ \hline \boxed{H} \boxed{S} \boxed{H} \end{array}$$

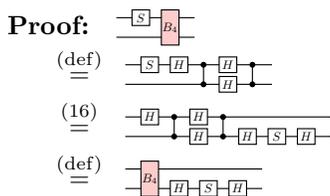

### 3.32 Equation

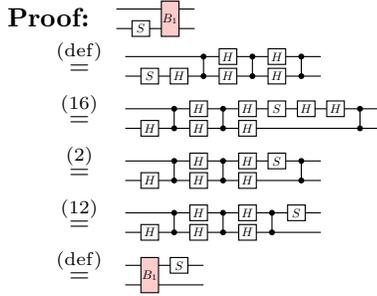

### 3.33 Equation

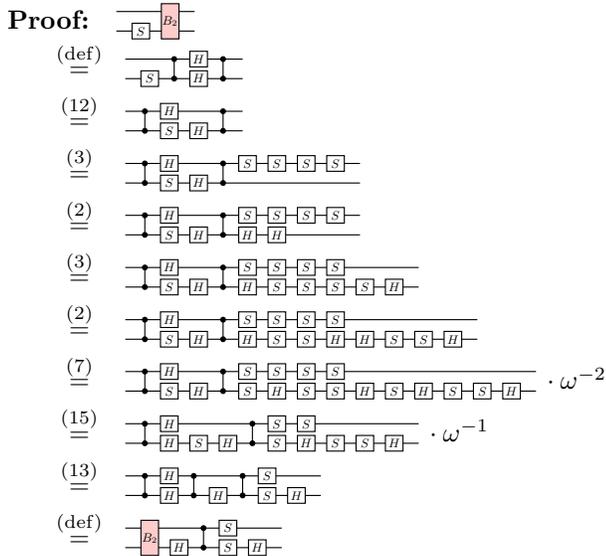

### 3.34 Equation

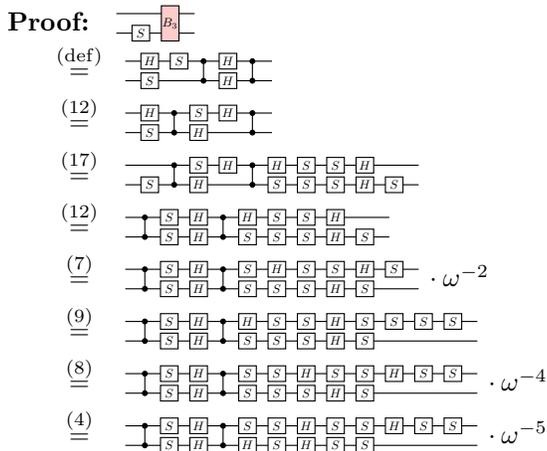

(10) 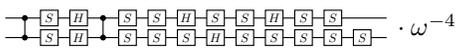 · ω<sup>-4</sup>

(4) 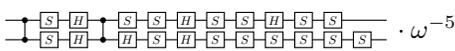 · ω<sup>-5</sup>

(5) 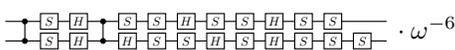 · ω<sup>-6</sup>

(7) 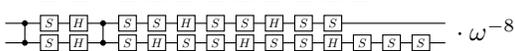 · ω<sup>-8</sup>

(15) 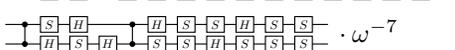 · ω<sup>-7</sup>

(8) 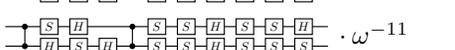 · ω<sup>-11</sup>

(6) 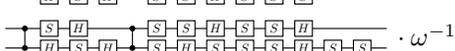 · ω<sup>-10</sup>

(13) 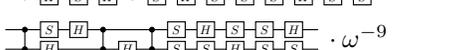 · ω<sup>-9</sup>

(9) 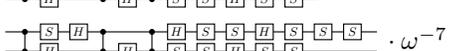 · ω<sup>-7</sup>

(2) 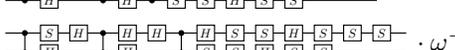 · ω<sup>-7</sup>

(14) 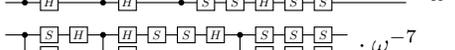 · ω<sup>-7</sup>

(2) 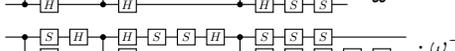 · ω<sup>-7</sup>

(14) 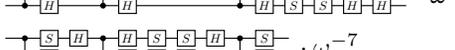 · ω<sup>-7</sup>

(3) 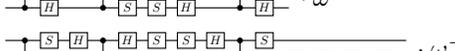 · ω<sup>-7</sup>

(12) 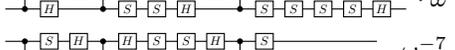 · ω<sup>-7</sup>

(12) 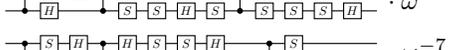 · ω<sup>-7</sup>

(12) 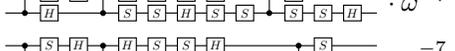 · ω<sup>-7</sup>

(5) 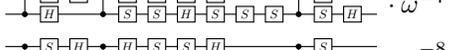 · ω<sup>-8</sup>

(17) 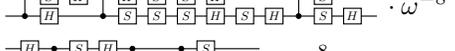 · ω<sup>-8</sup>

(12) 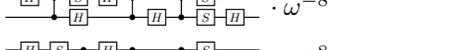 · ω<sup>-8</sup>

(1) 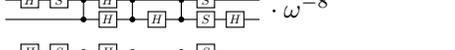 · ω<sup>-8</sup>

(def) 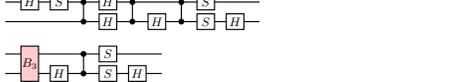 · ω<sup>-8</sup>

### 3.35 Equation

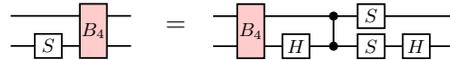

**Proof:** 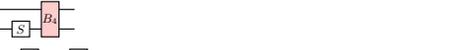 · ω<sup>-8</sup>

(def) 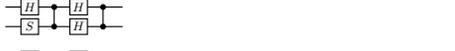 · ω<sup>-8</sup>

(12) 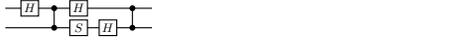 · ω<sup>-8</sup>

(3) 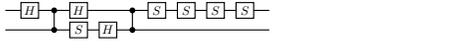 · ω<sup>-8</sup>

(2) 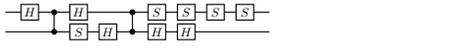 · ω<sup>-8</sup>

(3) 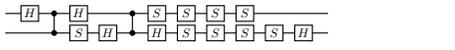 · ω<sup>-8</sup>

(2) 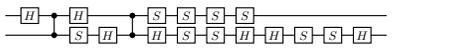 · ω<sup>-8</sup>

(7) 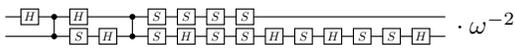 · ω<sup>-2</sup>

(15) 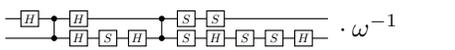 · ω<sup>-1</sup>

(13) 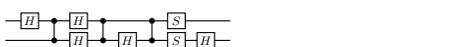 · ω<sup>-1</sup>



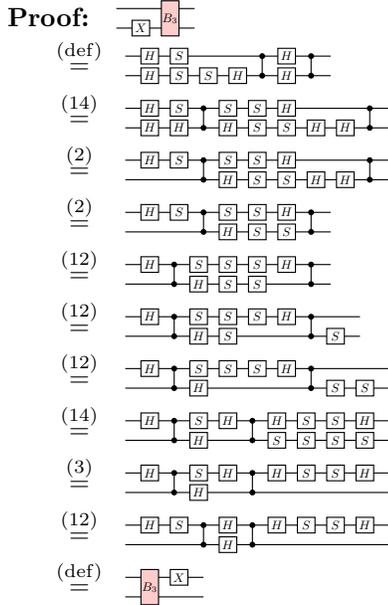

### 3.39 Equation

$$\begin{array}{c} \text{---} \\ \text{---} \end{array} \begin{array}{c} \boxed{B_4} \\ \boxed{X} \end{array} = \begin{array}{c} \text{---} \\ \text{---} \end{array} \begin{array}{c} \boxed{B_4} \\ \boxed{X} \end{array}$$

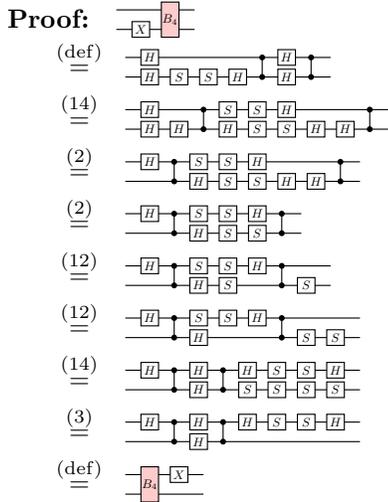

### 3.40 Equation

$$\begin{array}{c} \text{---} \\ \text{---} \end{array} \begin{array}{c} \boxed{B_1} \\ \text{---} \\ \text{---} \end{array} = \begin{array}{c} \text{---} \\ \text{---} \end{array} \begin{array}{c} \boxed{B_1} \\ \text{---} \\ \text{---} \end{array} \begin{array}{c} \text{---} \\ \text{---} \end{array} \begin{array}{c} \boxed{H} \\ \boxed{H} \\ \boxed{H} \\ \boxed{H} \end{array}$$

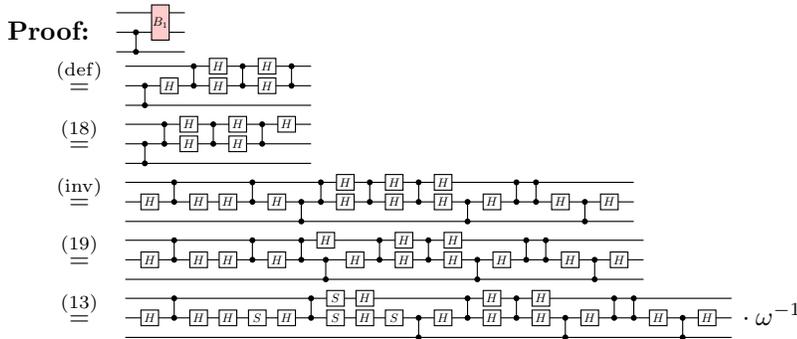

$$\begin{aligned}
& \underline{\underline{(15)}} \quad \text{Diagram 1} \cdot \omega^{-2} \\
& \underline{\underline{(7)}} \quad \text{Diagram 2} \\
& \underline{\underline{(2)}} \quad \text{Diagram 3} \\
& \underline{\underline{(12)}} \quad \text{Diagram 4} \\
& \underline{\underline{(12)}} \quad \text{Diagram 5} \\
& \underline{\underline{(12)}} \quad \text{Diagram 6} \\
& \underline{\underline{(14)}} \quad \text{Diagram 7} \\
& \underline{\underline{(2)}} \quad \text{Diagram 8} \\
& \underline{\underline{(14)}} \quad \text{Diagram 9} \\
& \underline{\underline{(8)}} \quad \text{Diagram 10} \cdot \omega^4 \\
& \underline{\underline{(2)}} \quad \text{Diagram 11} \cdot \omega^4 \\
& \underline{\underline{(12)}} \quad \text{Diagram 12} \cdot \omega^4 \\
& \underline{\underline{(12)}} \quad \text{Diagram 13} \cdot \omega^4 \\
& \underline{\underline{(14)}} \quad \text{Diagram 14} \cdot \omega^4 \\
& \underline{\underline{(8)}} \quad \text{Diagram 15} \cdot \omega^8 \\
& \underline{\underline{(2)}} \quad \text{Diagram 16} \cdot \omega^8 \\
& \underline{\underline{(12)}} \quad \text{Diagram 17} \cdot \omega^8 \\
& \underline{\underline{(12)}} \quad \text{Diagram 18} \cdot \omega^8 \\
& \underline{\underline{(3)}} \quad \text{Diagram 19} \cdot \omega^8 \\
& \underline{\underline{(14)}} \quad \text{Diagram 20} \cdot \omega^8 \\
& \underline{\underline{(3)}} \quad \text{Diagram 21} \cdot \omega^8 \\
& \underline{\underline{(2)}} \quad \text{Diagram 22} \cdot \omega^8 \\
& \underline{\underline{(16)}} \quad \text{Diagram 23} \cdot \omega^8 \\
& \underline{\underline{(2)}} \quad \text{Diagram 24} \cdot \omega^8 \\
& \underline{\underline{(16)}} \quad \text{Diagram 25} \cdot \omega^8 \\
& \underline{\underline{(2)}} \quad \text{Diagram 26} \cdot \omega^8 \\
& \underline{\underline{(12)}} \quad \text{Diagram 27} \cdot \omega^8 \\
& \underline{\underline{(12)}} \quad \text{Diagram 28} \cdot \omega^8 \\
& \underline{\underline{(12)}} \quad \text{Diagram 29} \cdot \omega^8 \\
& \underline{\underline{(14)}} \quad \text{Diagram 30} \cdot \omega^8 \\
& \underline{\underline{(12)}} \quad \text{Diagram 31} \cdot \omega^8
\end{aligned}$$

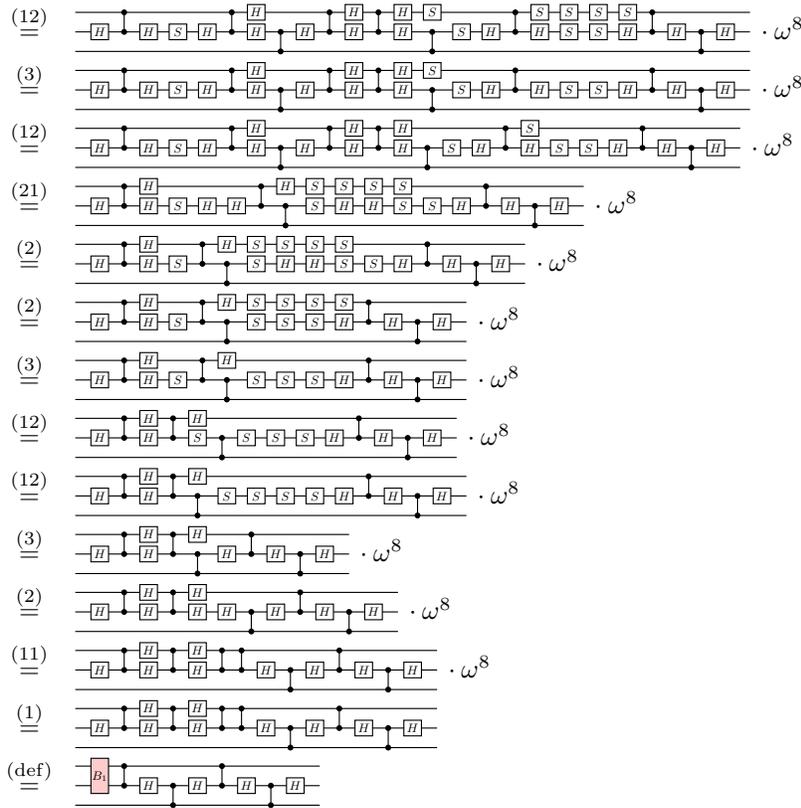

### 3.41 Equation

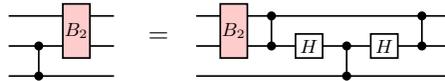

**Proof:**

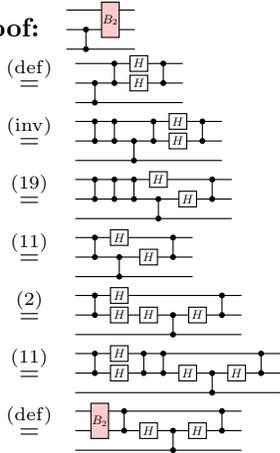

### 3.42 Equation

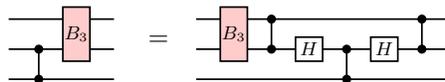

**Proof:**

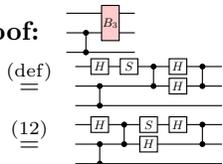

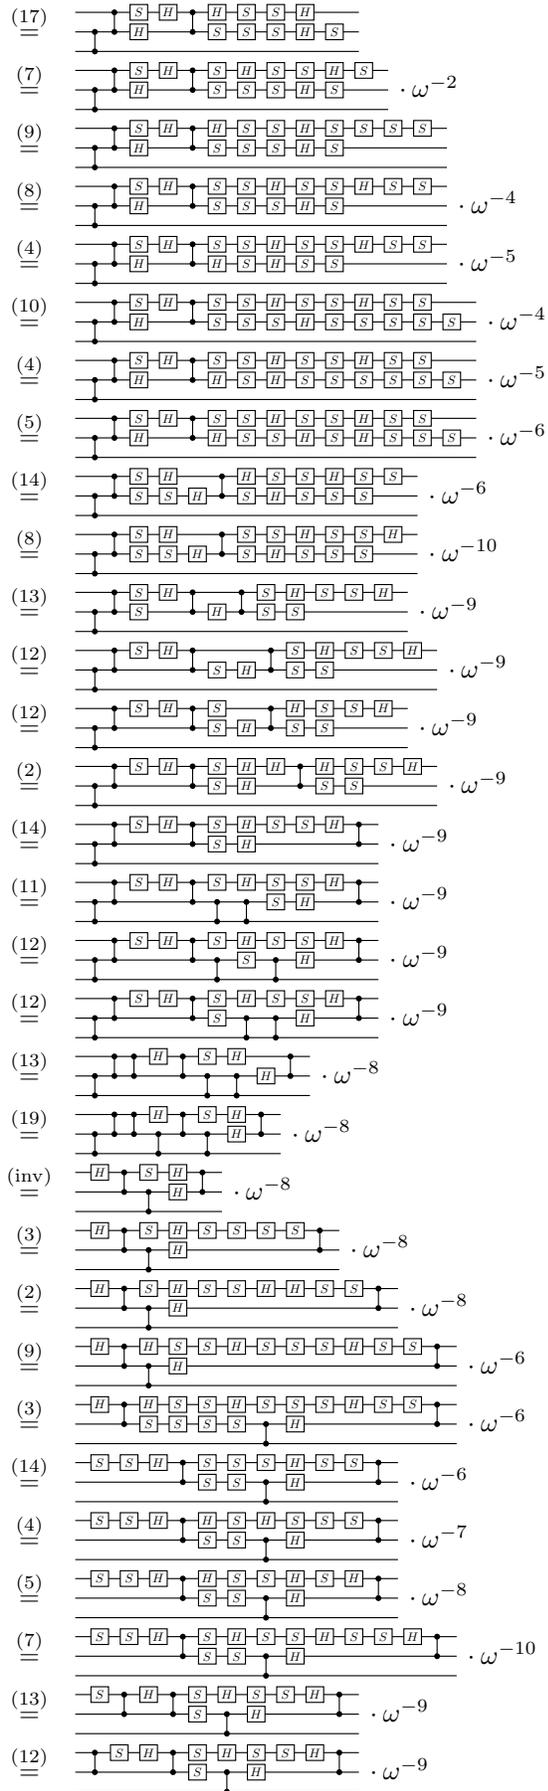

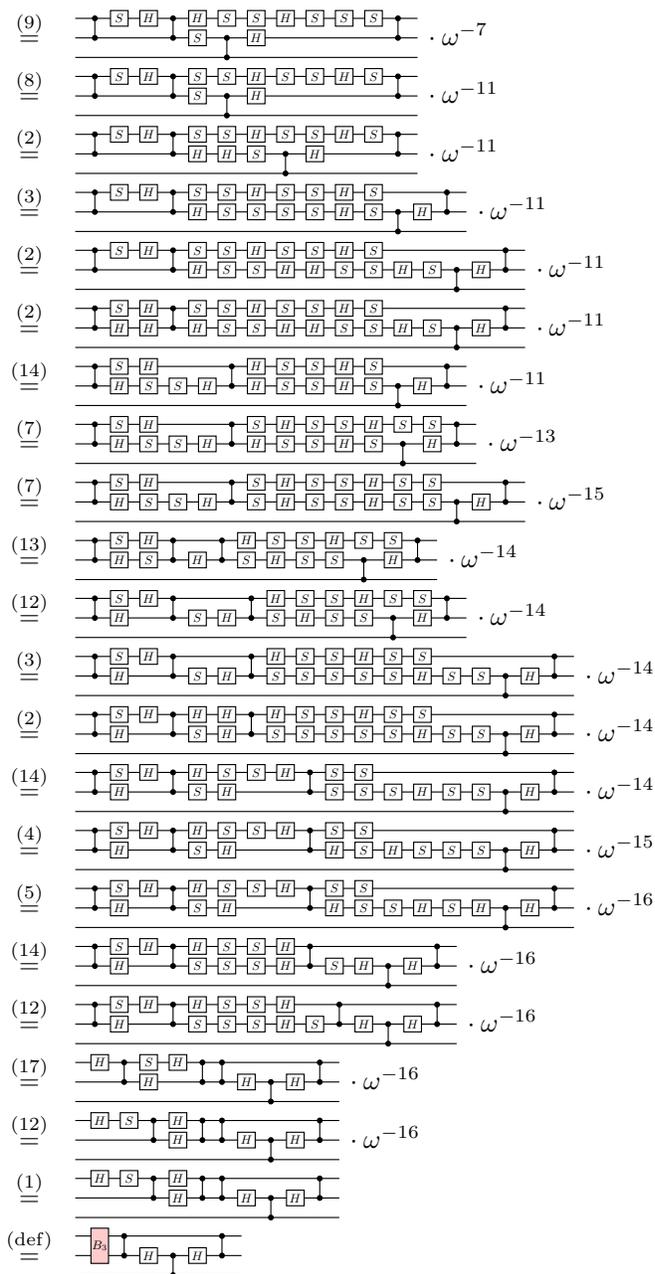

### 3.43 Equation

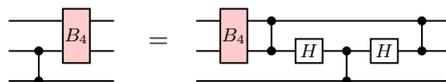

**Proof:**

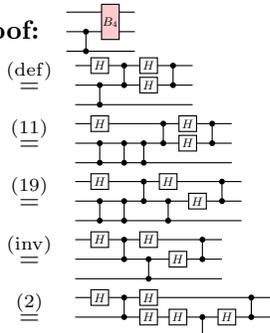

$$\begin{aligned}
 & \underline{\underline{(11)}} \quad \begin{array}{c} \text{---} \boxed{H} \text{---} \boxed{H} \text{---} \text{---} \text{---} \text{---} \\ \text{---} \text{---} \text{---} \boxed{H} \text{---} \text{---} \text{---} \text{---} \end{array} \\
 & \underline{\underline{(\text{def})}} \quad \begin{array}{c} \text{---} \boxed{B} \text{---} \text{---} \text{---} \text{---} \\ \text{---} \text{---} \text{---} \boxed{H} \text{---} \text{---} \text{---} \end{array}
 \end{aligned}$$

### 3.44 Equation

$$\text{---} \boxed{X} \boxed{C_1} \text{---} = \text{---} \boxed{C_2} \text{---}$$

**Proof:**

$$\begin{aligned}
 & \text{---} \boxed{X} \boxed{C_1} \text{---} \\
 & \underline{\underline{(\text{def})}} \quad \text{---} \boxed{H} \boxed{S} \boxed{S} \boxed{H} \text{---} \\
 & \underline{\underline{(\text{def})}} \quad \text{---} \boxed{C_2} \text{---}
 \end{aligned}$$

### 3.45 Equation

$$\text{---} \boxed{X} \boxed{C_2} \text{---} = \text{---} \boxed{C_1} \text{---}$$

**Proof:**

$$\begin{aligned}
 & \text{---} \boxed{X} \boxed{C_2} \text{---} \\
 & \underline{\underline{(\text{def})}} \quad \text{---} \boxed{H} \boxed{S} \boxed{S} \boxed{H} \boxed{H} \boxed{S} \boxed{S} \boxed{H} \text{---} \\
 & \underline{\underline{(2)}} \quad \text{---} \boxed{H} \boxed{S} \boxed{S} \boxed{S} \boxed{S} \boxed{H} \text{---} \\
 & \underline{\underline{(3)}} \quad \text{---} \boxed{H} \boxed{H} \text{---} \\
 & \underline{\underline{(2)}} \quad \text{---} \\
 & \underline{\underline{(\text{def})}} \quad \text{---} \boxed{C_1} \text{---}
 \end{aligned}$$

### 3.46 Equation

$$\text{---} \boxed{S} \boxed{C_1} \text{---} = \text{---} \boxed{C_1} \boxed{S} \text{---}$$

**Proof:**

$$\begin{aligned}
 & \text{---} \boxed{S} \boxed{C_1} \text{---} \\
 & \underline{\underline{(\text{def})}} \quad \text{---} \boxed{S} \text{---} \\
 & \underline{\underline{(\text{def})}} \quad \text{---} \boxed{C_1} \boxed{S} \text{---}
 \end{aligned}$$

### 3.47 Equation

$$\text{---} \boxed{S} \boxed{C_2} \text{---} = \text{---} \boxed{C_2} \boxed{S} \boxed{S} \boxed{S} \text{---} \cdot \omega^2$$

**Proof:**

$$\begin{aligned}
 & \text{---} \boxed{S} \boxed{C_2} \text{---} \\
 & \underline{\underline{(\text{def})}} \quad \text{---} \boxed{S} \boxed{H} \boxed{S} \boxed{S} \boxed{H} \text{---} \\
 & \underline{\underline{(9)}} \quad \text{---} \boxed{H} \boxed{S} \boxed{S} \boxed{H} \boxed{S} \boxed{S} \boxed{S} \text{---} \cdot \omega^2 \\
 & \underline{\underline{(\text{def})}} \quad \text{---} \boxed{C_2} \boxed{S} \boxed{S} \boxed{S} \text{---} \cdot \omega^2
 \end{aligned}$$

### 3.48 Equation

$$\begin{array}{c} \bullet \\ \text{---} \boxed{C_1} \text{---} \\ \bullet \end{array} = \begin{array}{c} \text{---} \boxed{C_1} \text{---} \\ \bullet \end{array}$$

**Proof:**

$$\begin{aligned}
 & \begin{array}{c} \bullet \\ \text{---} \boxed{C_1} \text{---} \\ \bullet \end{array} \\
 & \underline{\underline{(\text{def})}} \quad \begin{array}{c} \bullet \\ \text{---} \\ \bullet \end{array} \\
 & \underline{\underline{(\text{def})}} \quad \begin{array}{c} \text{---} \boxed{C_1} \text{---} \\ \bullet \end{array}
 \end{aligned}$$

### 3.49 Equation

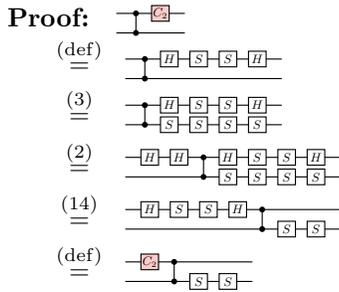

### 3.50 Equation

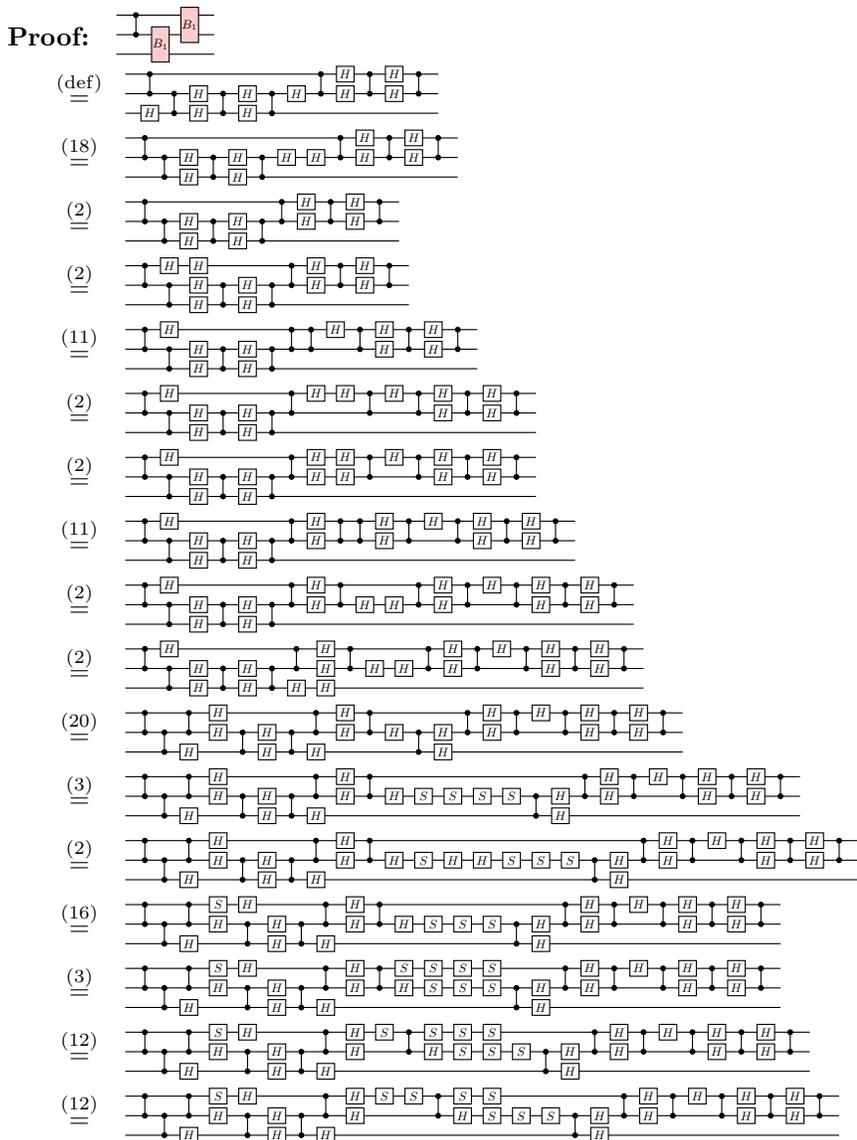

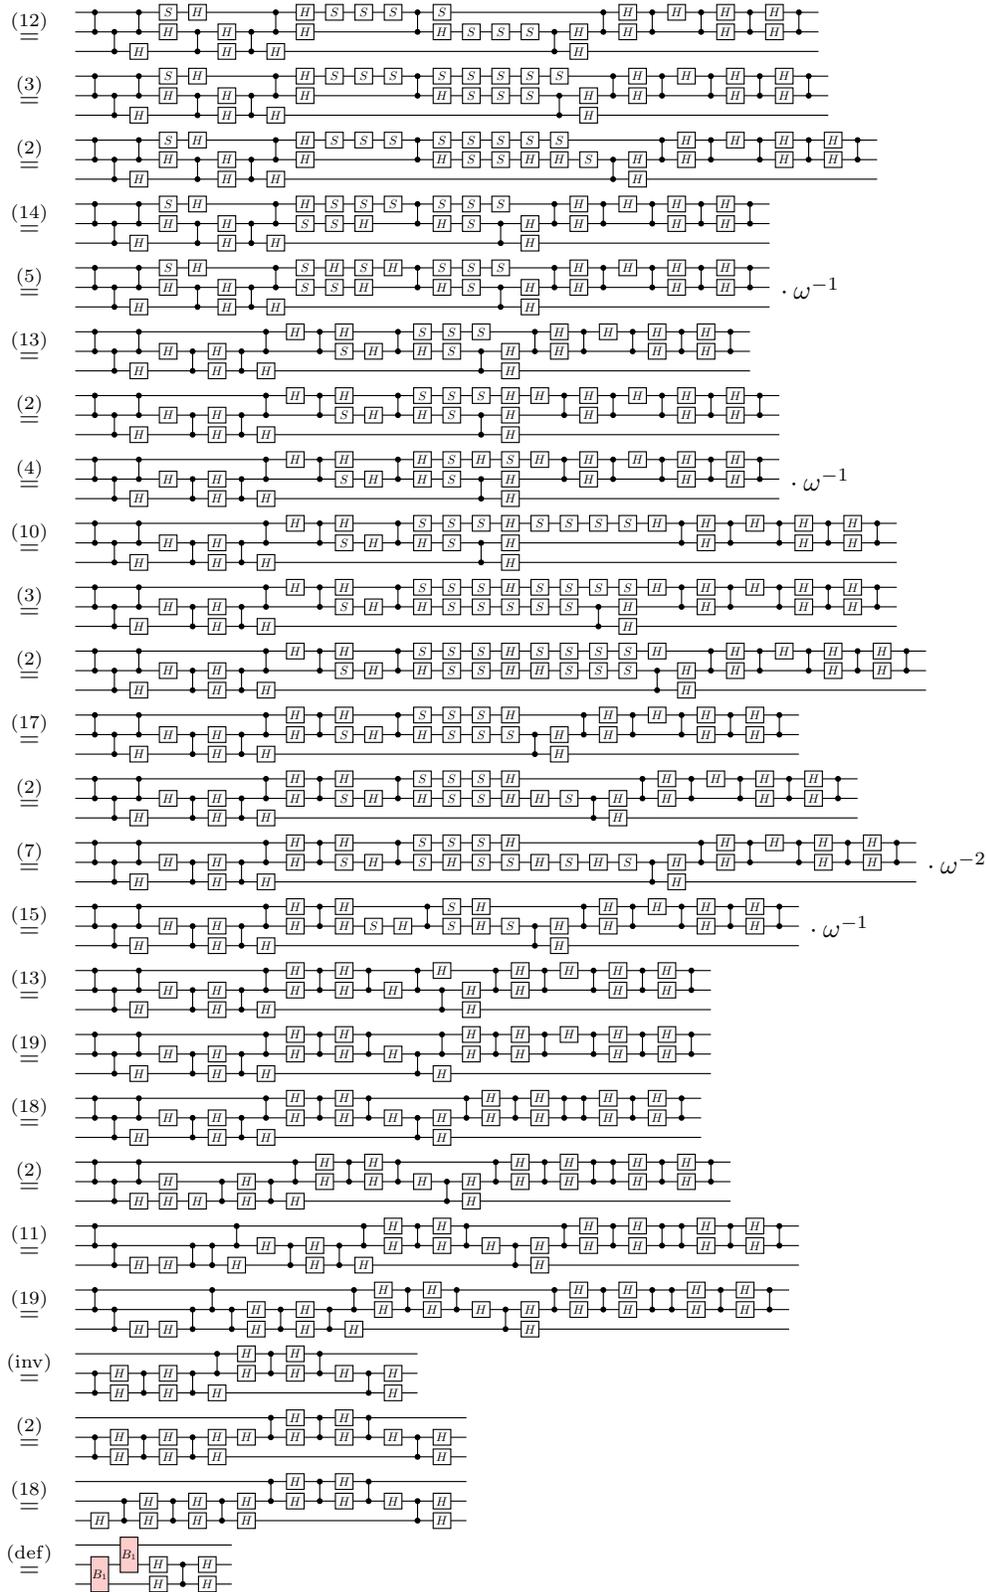

### 3.51 Equation

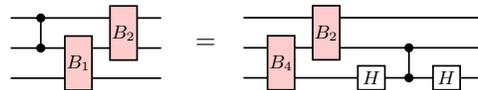

**Proof:**

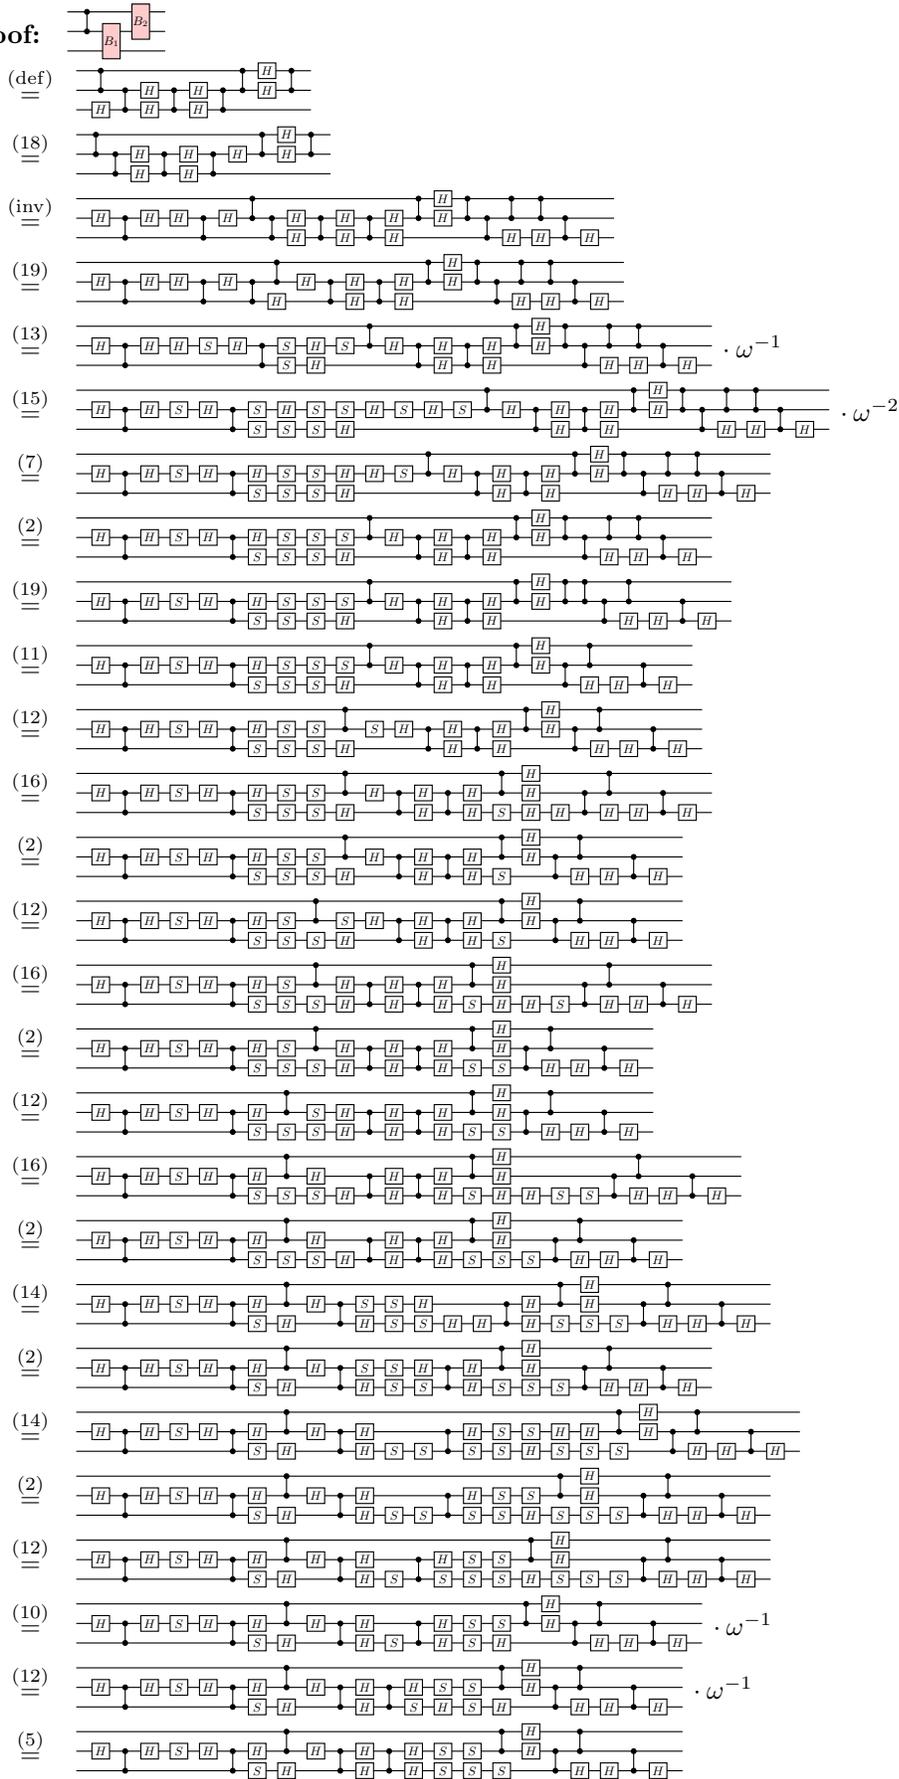



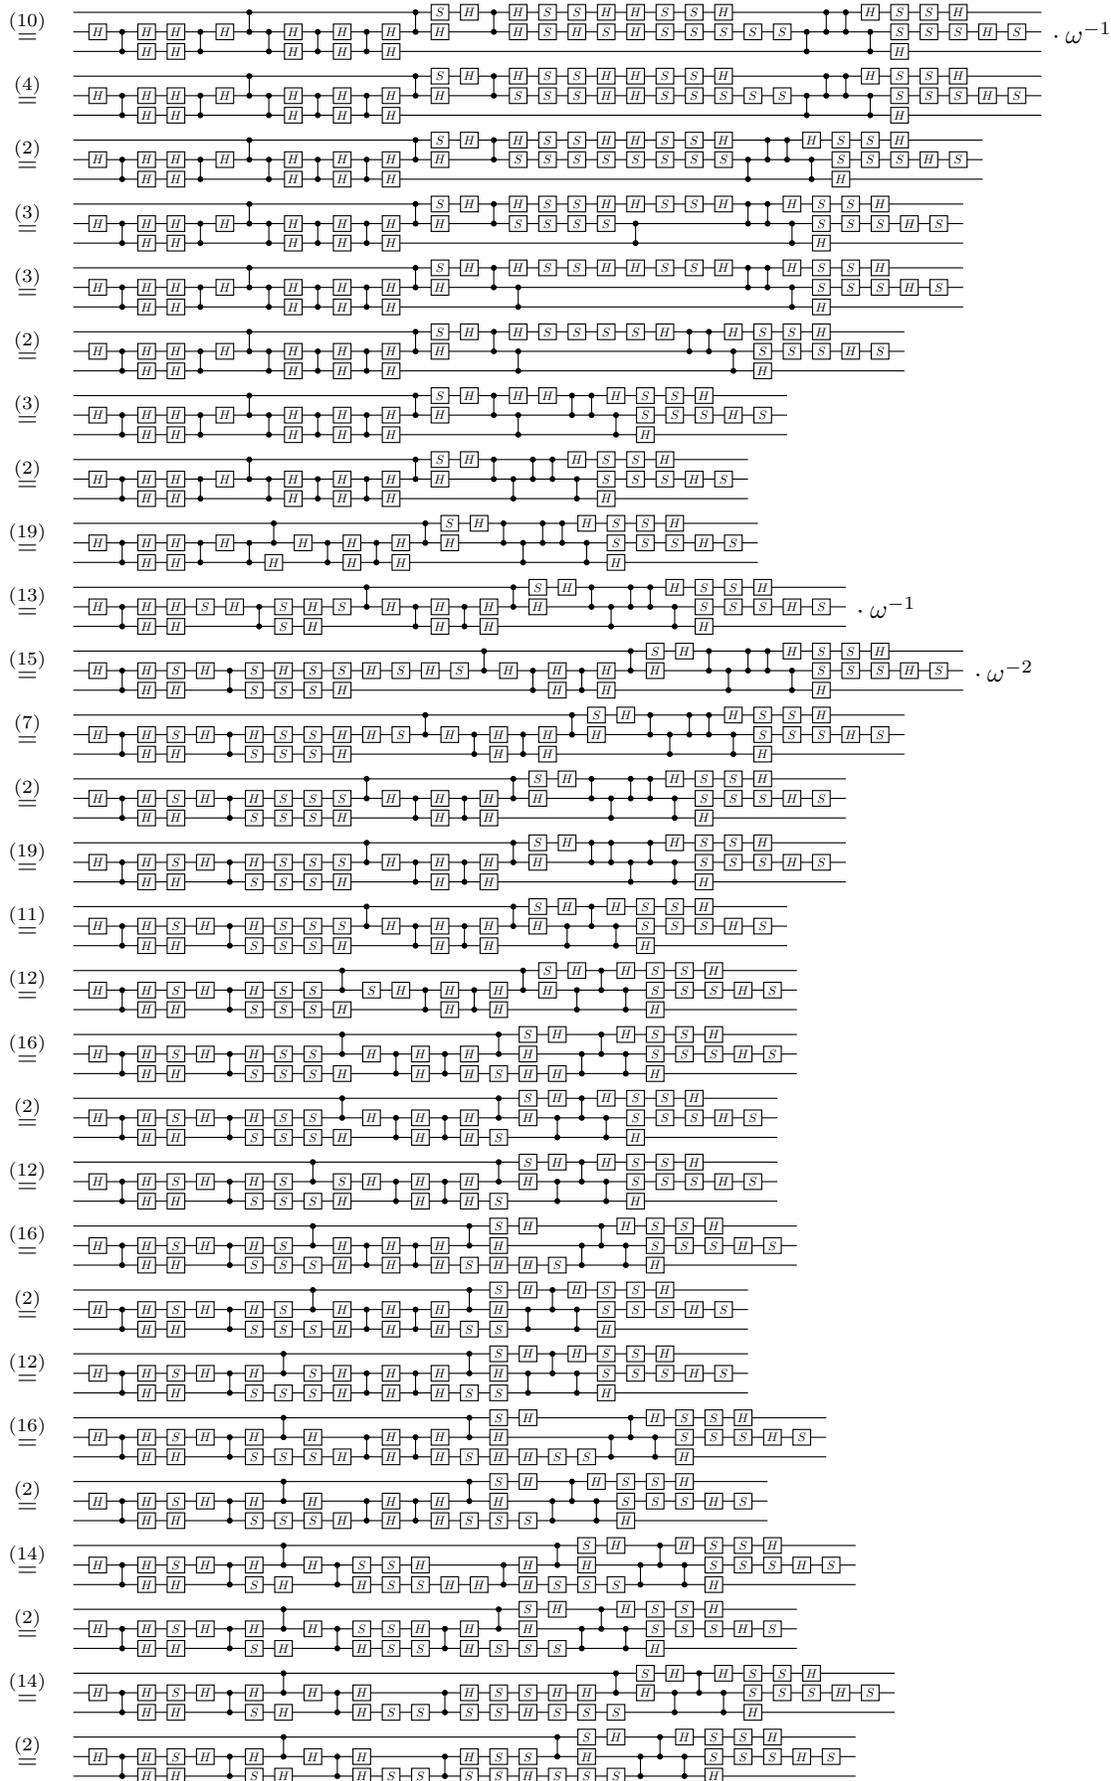

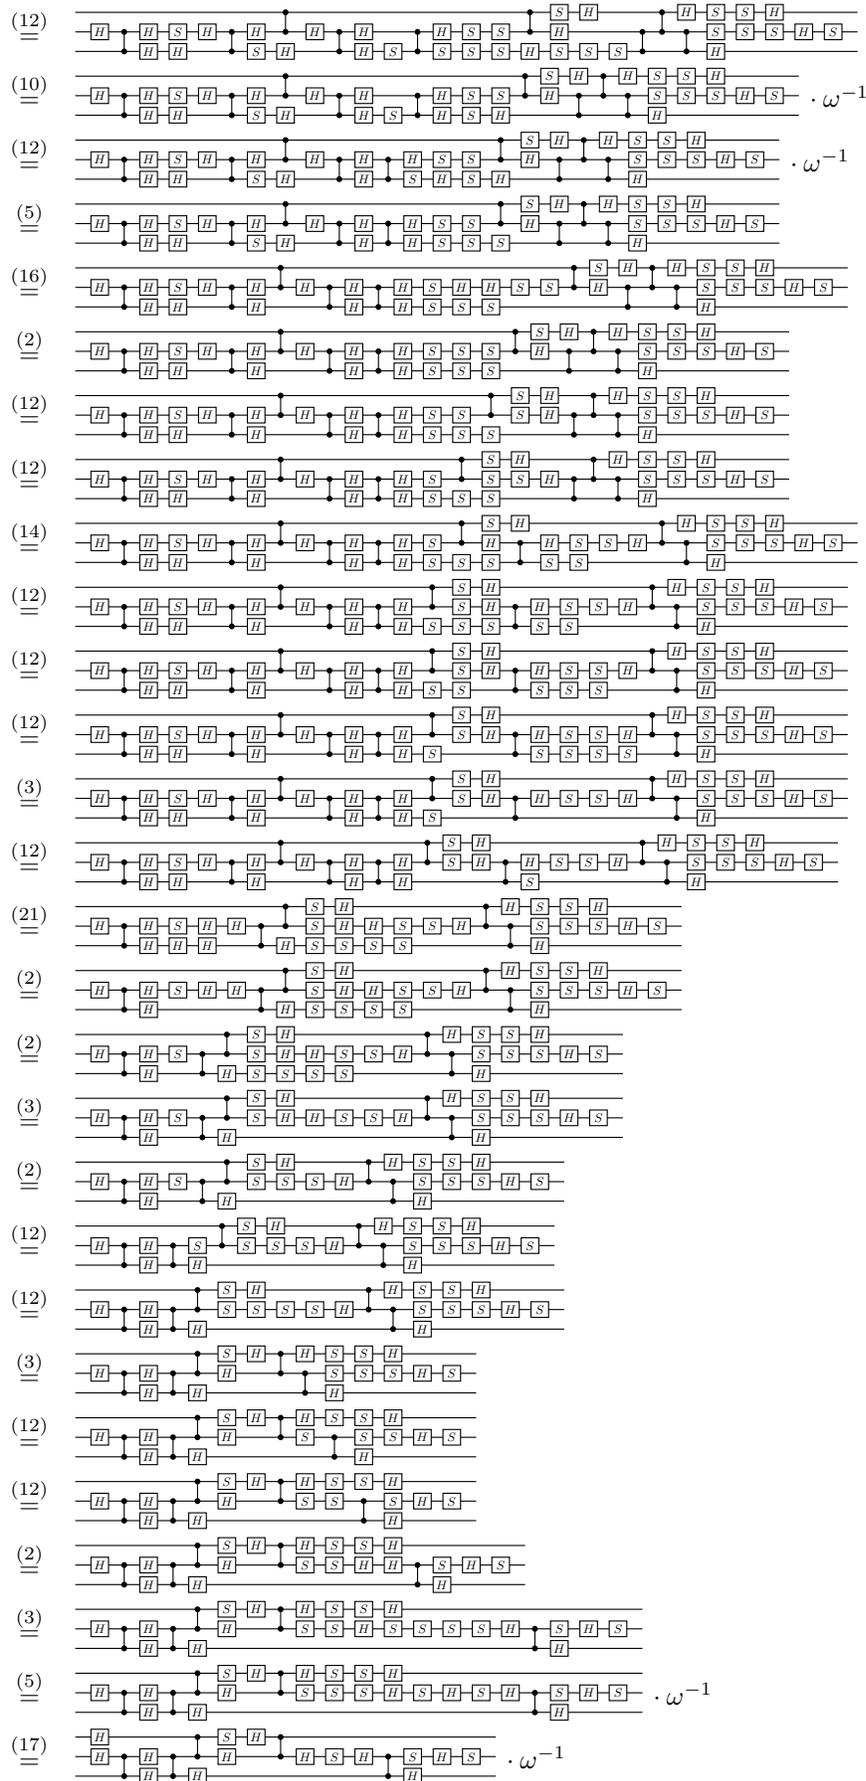



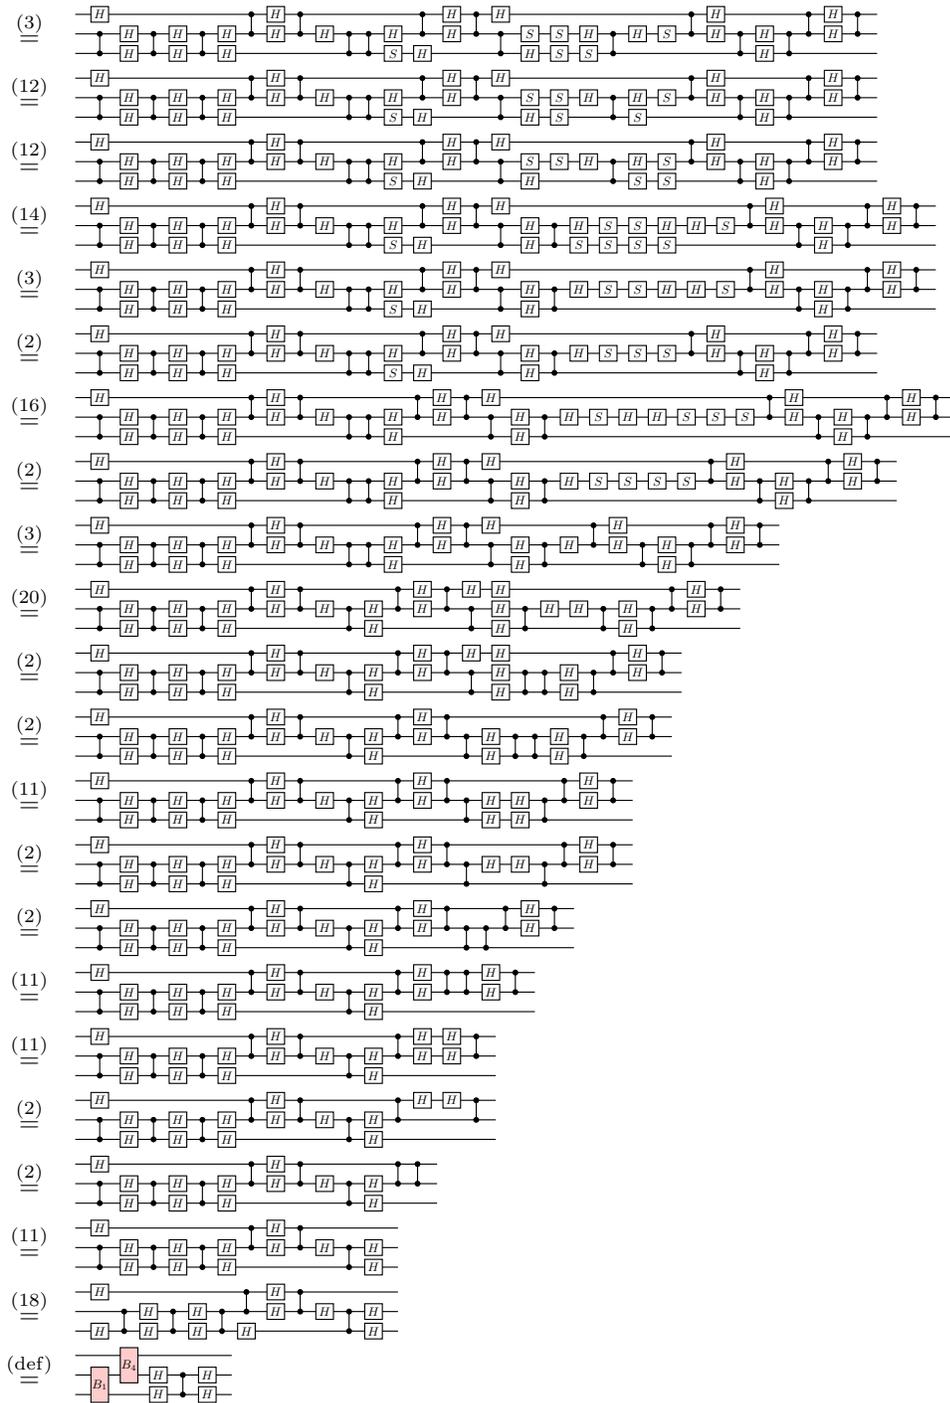

### 3.54 Equation

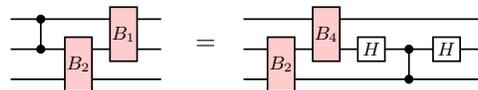

**Proof:**

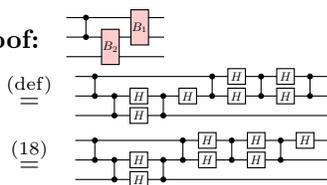



$$\begin{aligned}
& \underline{\underline{(16)}} \quad \text{[Diagram 1]} \cdot \omega^8 \\
& \underline{\underline{(2)}} \quad \text{[Diagram 2]} \cdot \omega^8 \\
& \underline{\underline{(16)}} \quad \text{[Diagram 3]} \cdot \omega^8 \\
& \underline{\underline{(2)}} \quad \text{[Diagram 4]} \cdot \omega^8 \\
& \underline{\underline{(12)}} \quad \text{[Diagram 5]} \cdot \omega^8 \\
& \underline{\underline{(12)}} \quad \text{[Diagram 6]} \cdot \omega^8 \\
& \underline{\underline{(12)}} \quad \text{[Diagram 7]} \cdot \omega^8 \\
& \underline{\underline{(14)}} \quad \text{[Diagram 8]} \cdot \omega^8 \\
& \underline{\underline{(12)}} \quad \text{[Diagram 9]} \cdot \omega^8 \\
& \underline{\underline{(12)}} \quad \text{[Diagram 10]} \cdot \omega^8 \\
& \underline{\underline{(3)}} \quad \text{[Diagram 11]} \cdot \omega^8 \\
& \underline{\underline{(12)}} \quad \text{[Diagram 12]} \cdot \omega^8 \\
& \underline{\underline{(21)}} \quad \text{[Diagram 13]} \cdot \omega^8 \\
& \underline{\underline{(2)}} \quad \text{[Diagram 14]} \cdot \omega^8 \\
& \underline{\underline{(2)}} \quad \text{[Diagram 15]} \cdot \omega^8 \\
& \underline{\underline{(3)}} \quad \text{[Diagram 16]} \cdot \omega^8 \\
& \underline{\underline{(12)}} \quad \text{[Diagram 17]} \cdot \omega^8 \\
& \underline{\underline{(12)}} \quad \text{[Diagram 18]} \cdot \omega^8 \\
& \underline{\underline{(3)}} \quad \text{[Diagram 19]} \cdot \omega^8 \\
& \underline{\underline{(19)}} \quad \text{[Diagram 20]} \cdot \omega^8 \\
& \underline{\underline{(11)}} \quad \text{[Diagram 21]} \cdot \omega^8 \\
& \underline{\underline{(1)}} \quad \text{[Diagram 22]} \\
& \underline{\underline{(\text{def})}} \quad \text{[Diagram 23]}
\end{aligned}$$

### 3.55 Equation

$$\text{[Diagram 24]} = \text{[Diagram 25]} \cdot \omega^6$$

**Proof:**

$$\begin{aligned}
& \underline{\underline{(\text{def})}} \quad \text{[Diagram 26]}
\end{aligned}$$



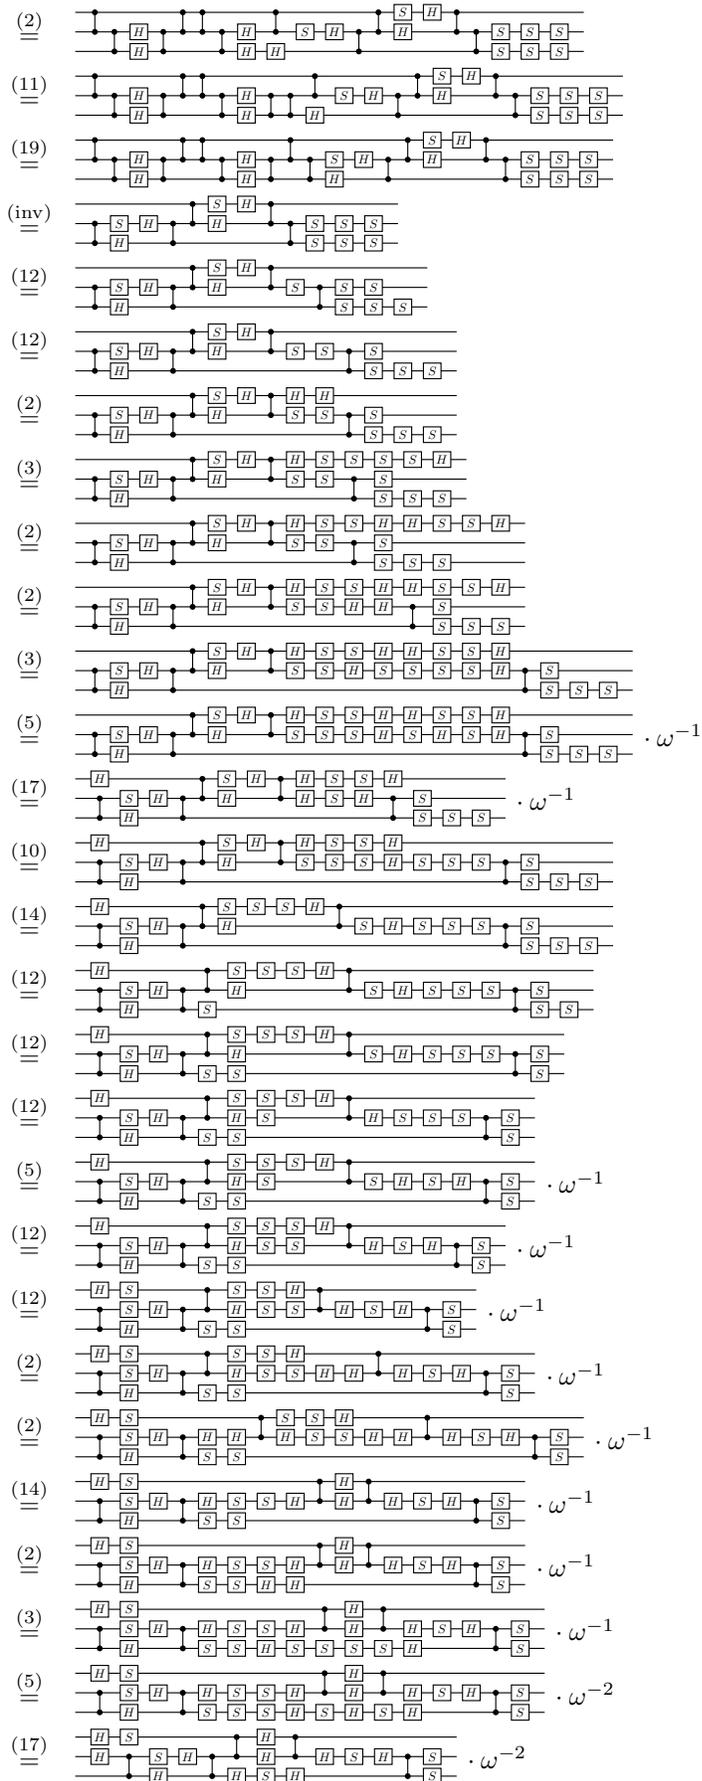





$$\begin{aligned}
& \underline{(14)} \quad \text{[Diagram with H and S gates]} \\
& \underline{(2)} \quad \text{[Diagram with H and S gates]} \\
& \underline{(3)} \quad \text{[Diagram with H and S gates]} \\
& \underline{(5)} \quad \text{[Diagram with H and S gates]} \cdot \omega^{-1} \\
& \underline{(17)} \quad \text{[Diagram with H and S gates]} \cdot \omega^{-1} \\
& \underline{(12)} \quad \text{[Diagram with H and S gates]} \cdot \omega^{-1} \\
& \underline{(1)} \quad \text{[Diagram with H and S gates]} \cdot \omega^7 \\
& \underline{\text{(def)}} \quad \text{[Diagram with } B_3, B_2, X \text{ gates]} \cdot \omega^7
\end{aligned}$$

### 3.57 Equation

$$\text{[Diagram with } B_2, B_4 \text{ gates]} = \text{[Diagram with } B_2, B_1, H \text{ gates]}$$

**Proof:**

$$\begin{aligned}
& \underline{\text{(def)}} \quad \text{[Diagram with } B_2, B_4 \text{ gates]} \\
& \underline{(11)} \quad \text{[Diagram with H gates]} \\
& \underline{(19)} \quad \text{[Diagram with H gates]} \\
& \underline{(3)} \quad \text{[Diagram with H gates]} \\
& \underline{(12)} \quad \text{[Diagram with H and S gates]} \\
& \underline{(12)} \quad \text{[Diagram with H and S gates]} \\
& \underline{(3)} \quad \text{[Diagram with H and S gates]} \\
& \underline{(2)} \quad \text{[Diagram with H and S gates]} \\
& \underline{(2)} \quad \text{[Diagram with H and S gates]} \\
& \underline{(21)} \quad \text{[Diagram with H and S gates]} \\
& \underline{(12)} \quad \text{[Diagram with H and S gates]} \\
& \underline{(3)} \quad \text{[Diagram with H and S gates]} \\
& \underline{(12)} \quad \text{[Diagram with H and S gates]} \\
& \underline{(12)} \quad \text{[Diagram with H and S gates]} \\
& \underline{(14)} \quad \text{[Diagram with H and S gates]} \\
& \underline{(12)} \quad \text{[Diagram with H and S gates]}
\end{aligned}$$

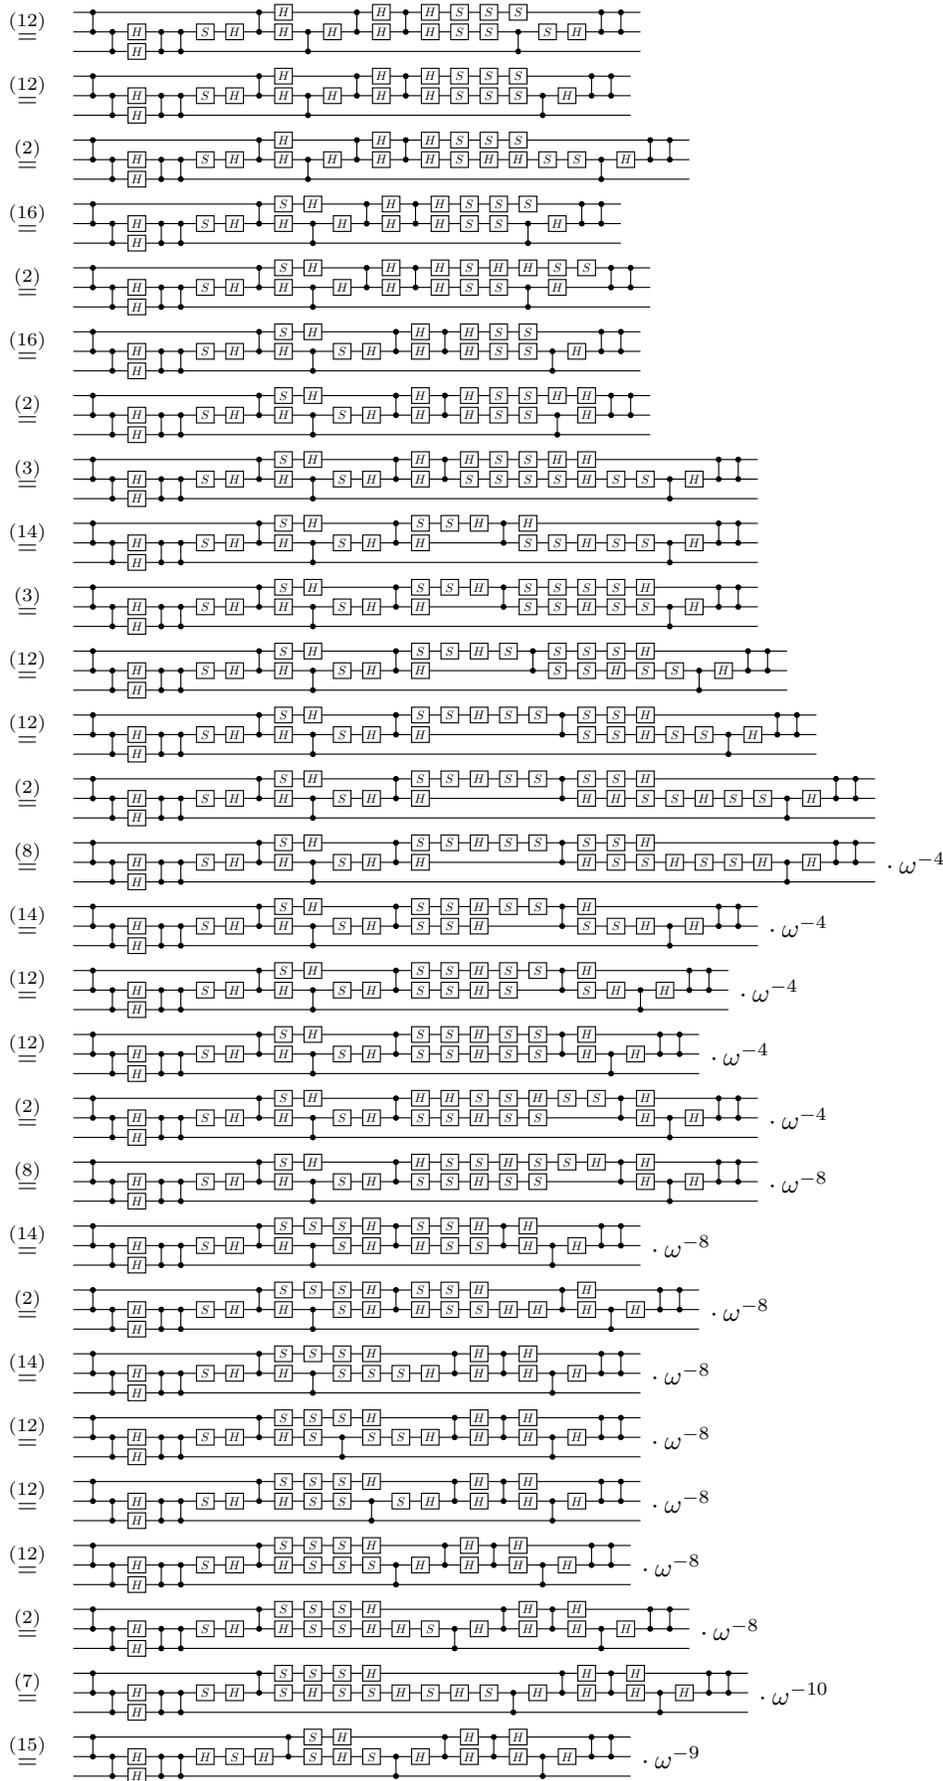

$$\begin{aligned}
(13) \quad & \text{---} \cdot \omega^{-8} \\
(19) \quad & \text{---} \cdot \omega^{-8} \\
(2) \quad & \text{---} \cdot \omega^{-8} \\
(11) \quad & \text{---} \cdot \omega^{-8} \\
(19) \quad & \text{---} \cdot \omega^{-8} \\
(\text{inv}) \quad & \text{---} \cdot \omega^{-8} \\
(18) \quad & \text{---} \cdot \omega^{-8} \\
(1) \quad & \text{---} \\
(\text{def}) \quad & \text{---}
\end{aligned}$$

### 3.58 Equation

$$\text{---} = \text{---} \cdot \omega^7$$

**Proof:**

$$\begin{aligned}
& \text{---} \\
(\text{def}) \quad & \text{---} \\
(12) \quad & \text{---} \\
(17) \quad & \text{---} \\
(2) \quad & \text{---} \\
(12) \quad & \text{---} \\
(12) \quad & \text{---} \\
(14) \quad & \text{---} \\
(2) \quad & \text{---} \\
(12) \quad & \text{---} \\
(12) \quad & \text{---} \\
(14) \quad & \text{---} \\
(3) \quad & \text{---} \\
(18) \quad & \text{---} \\
(2) \quad & \text{---} \\
(\text{inv}) \quad & \text{---}
\end{aligned}$$

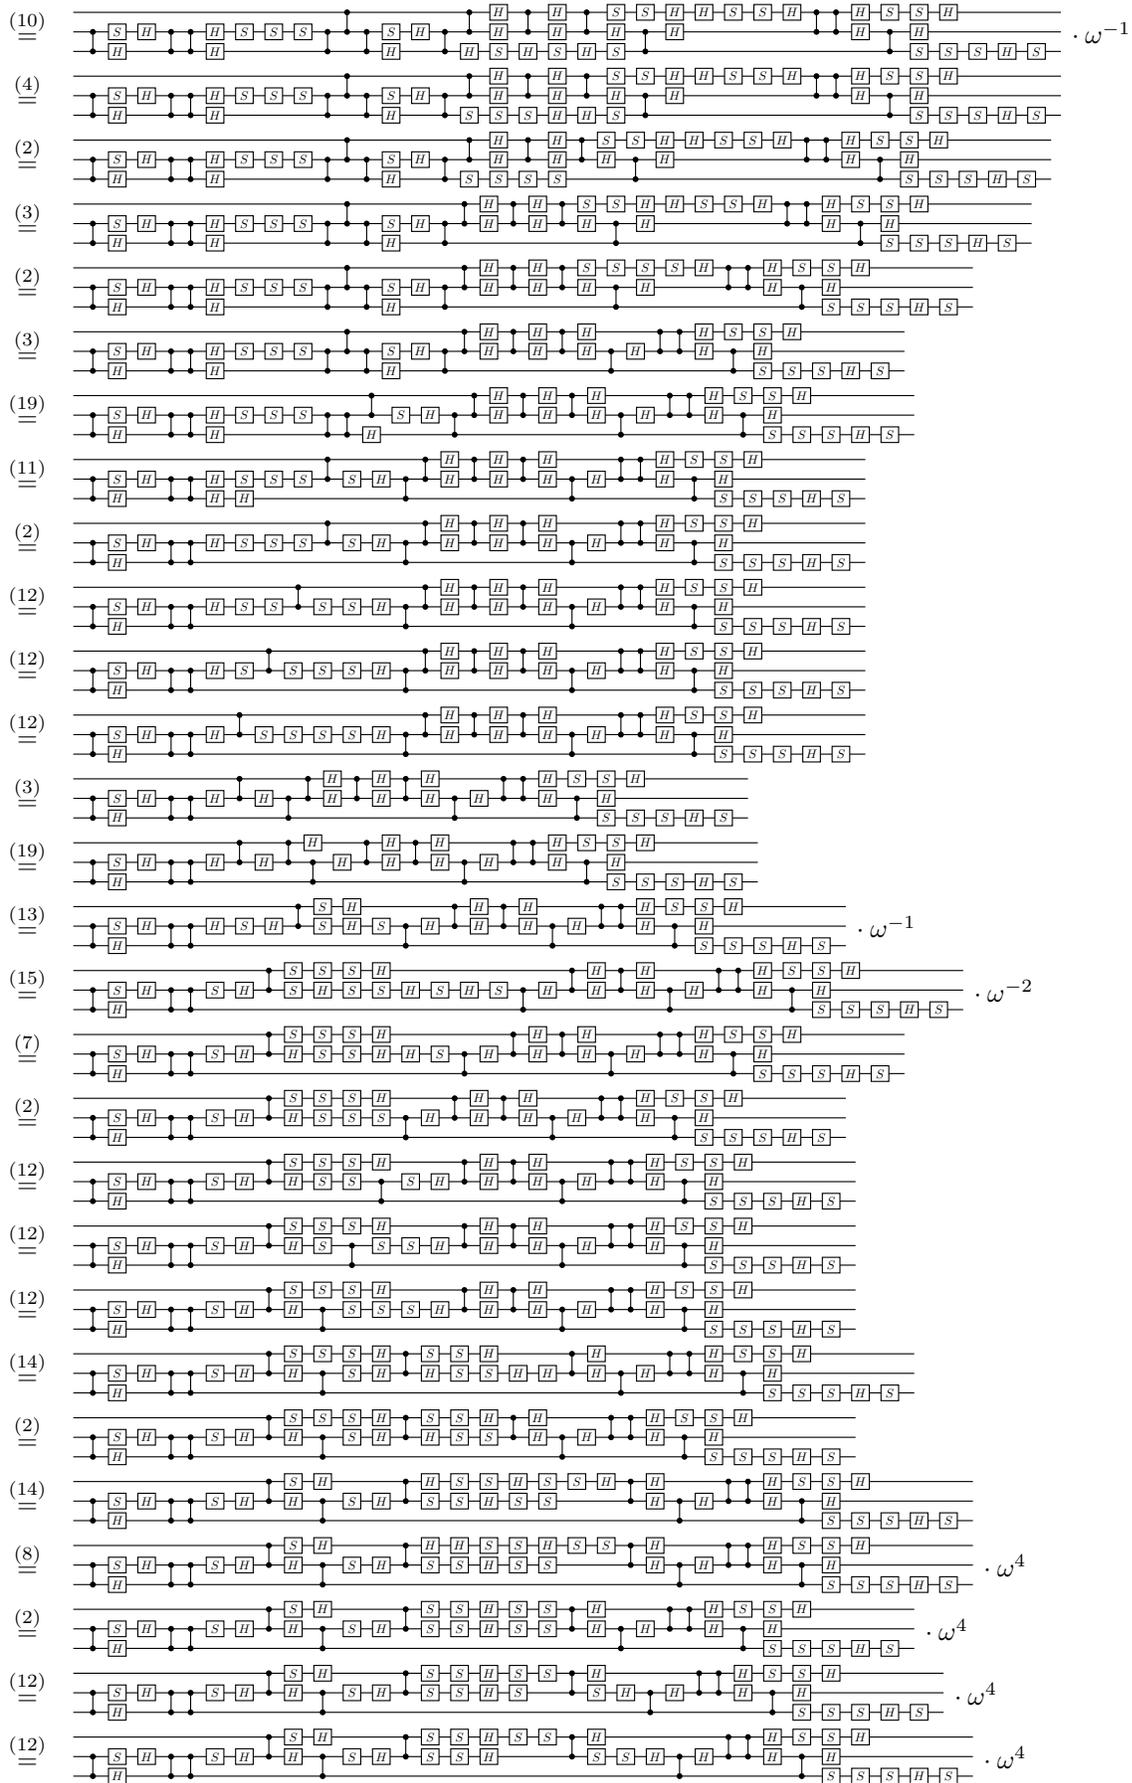

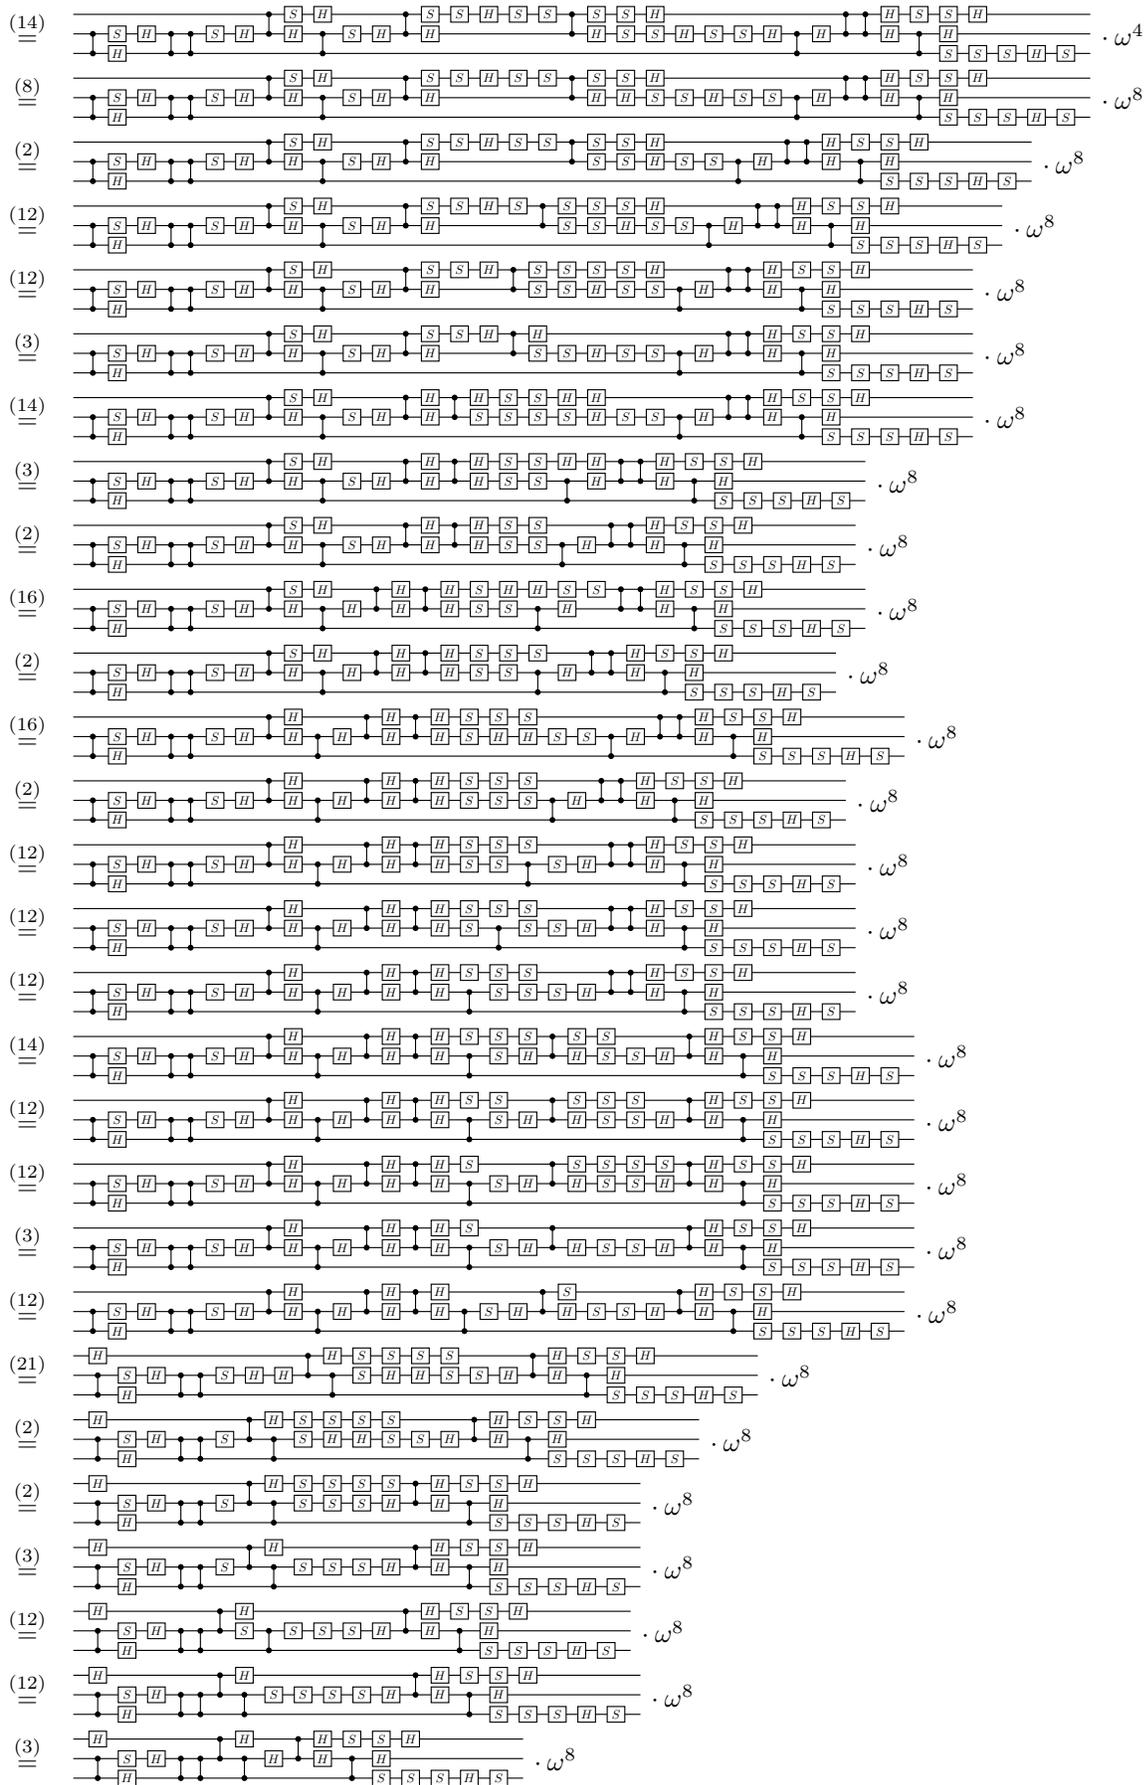



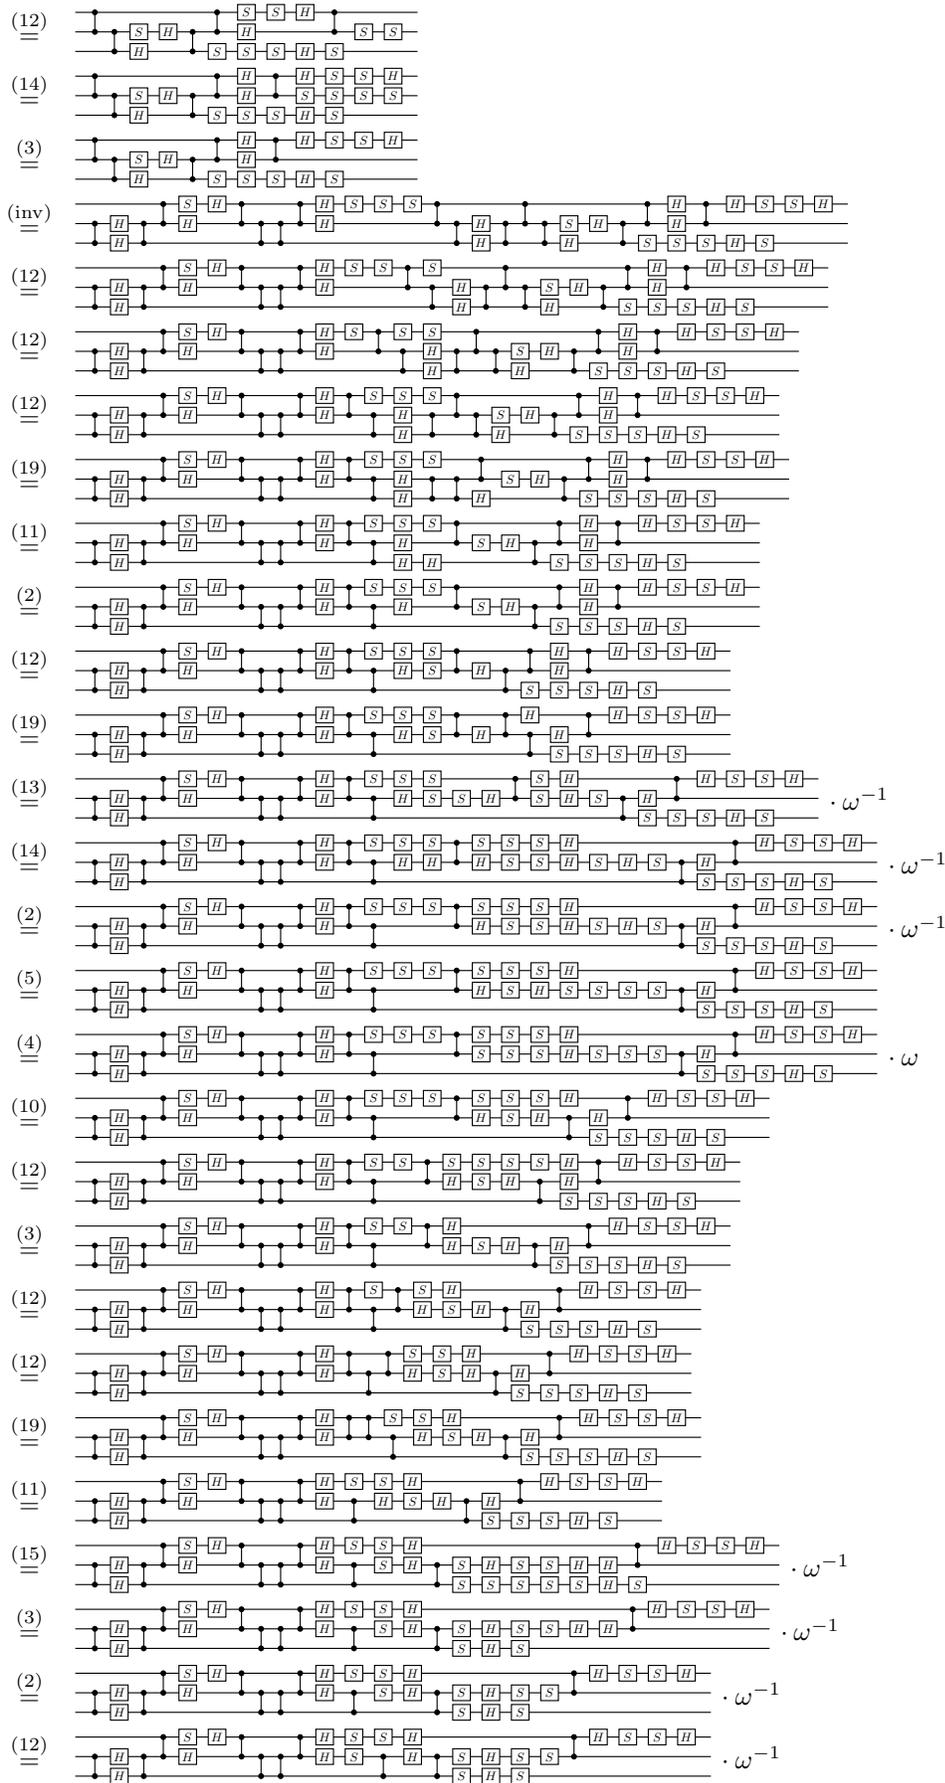

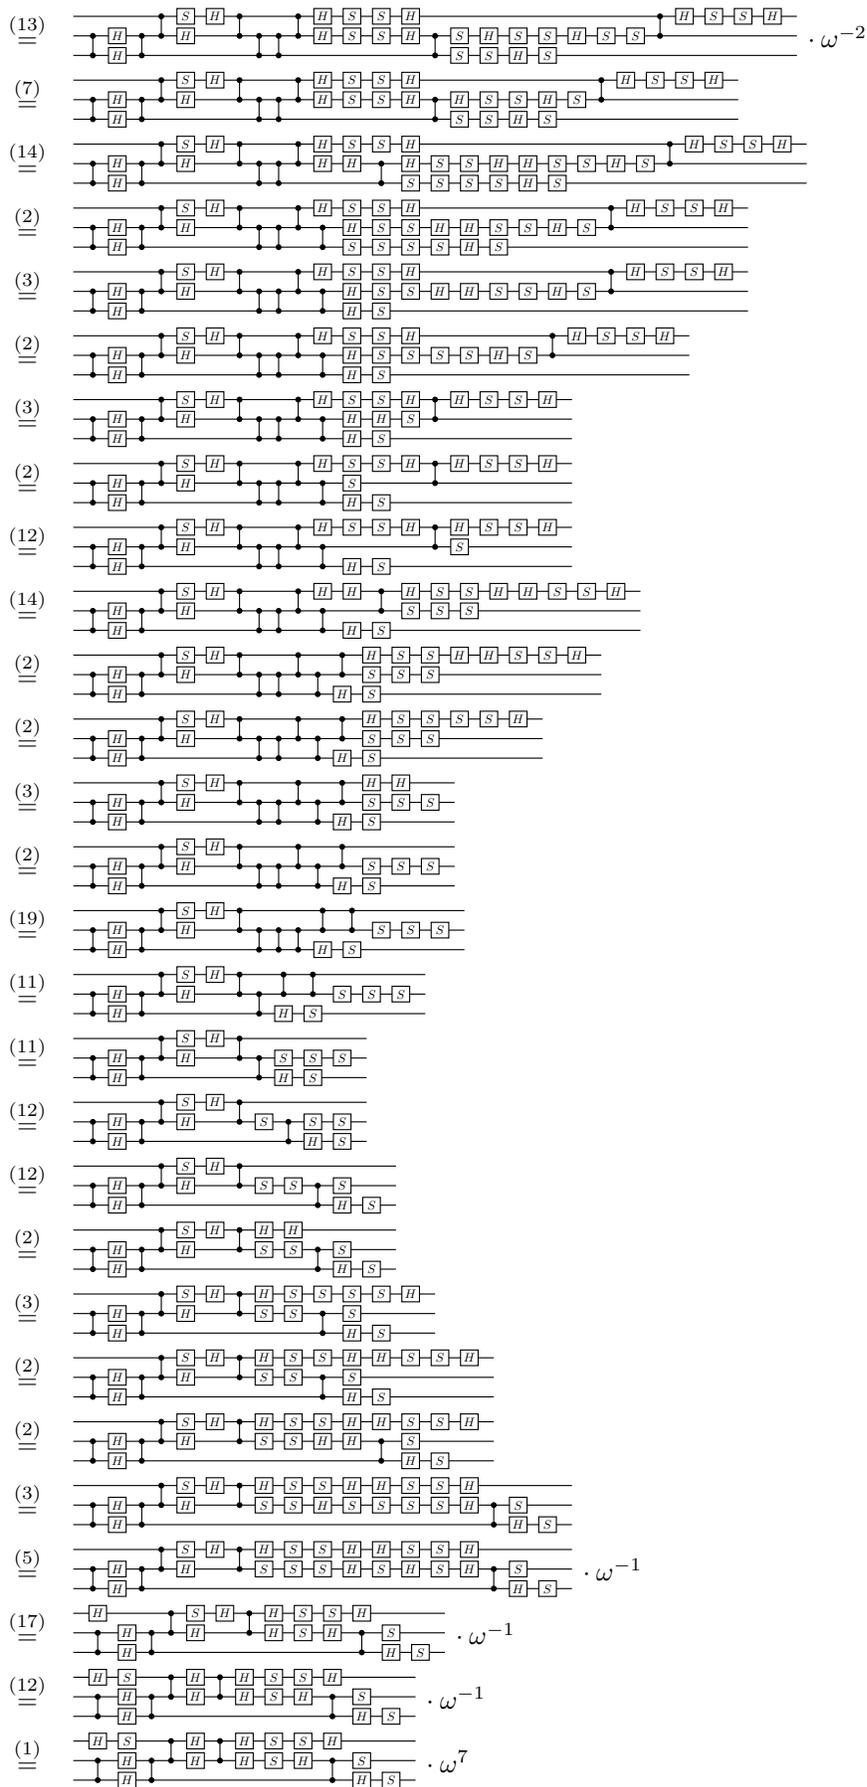



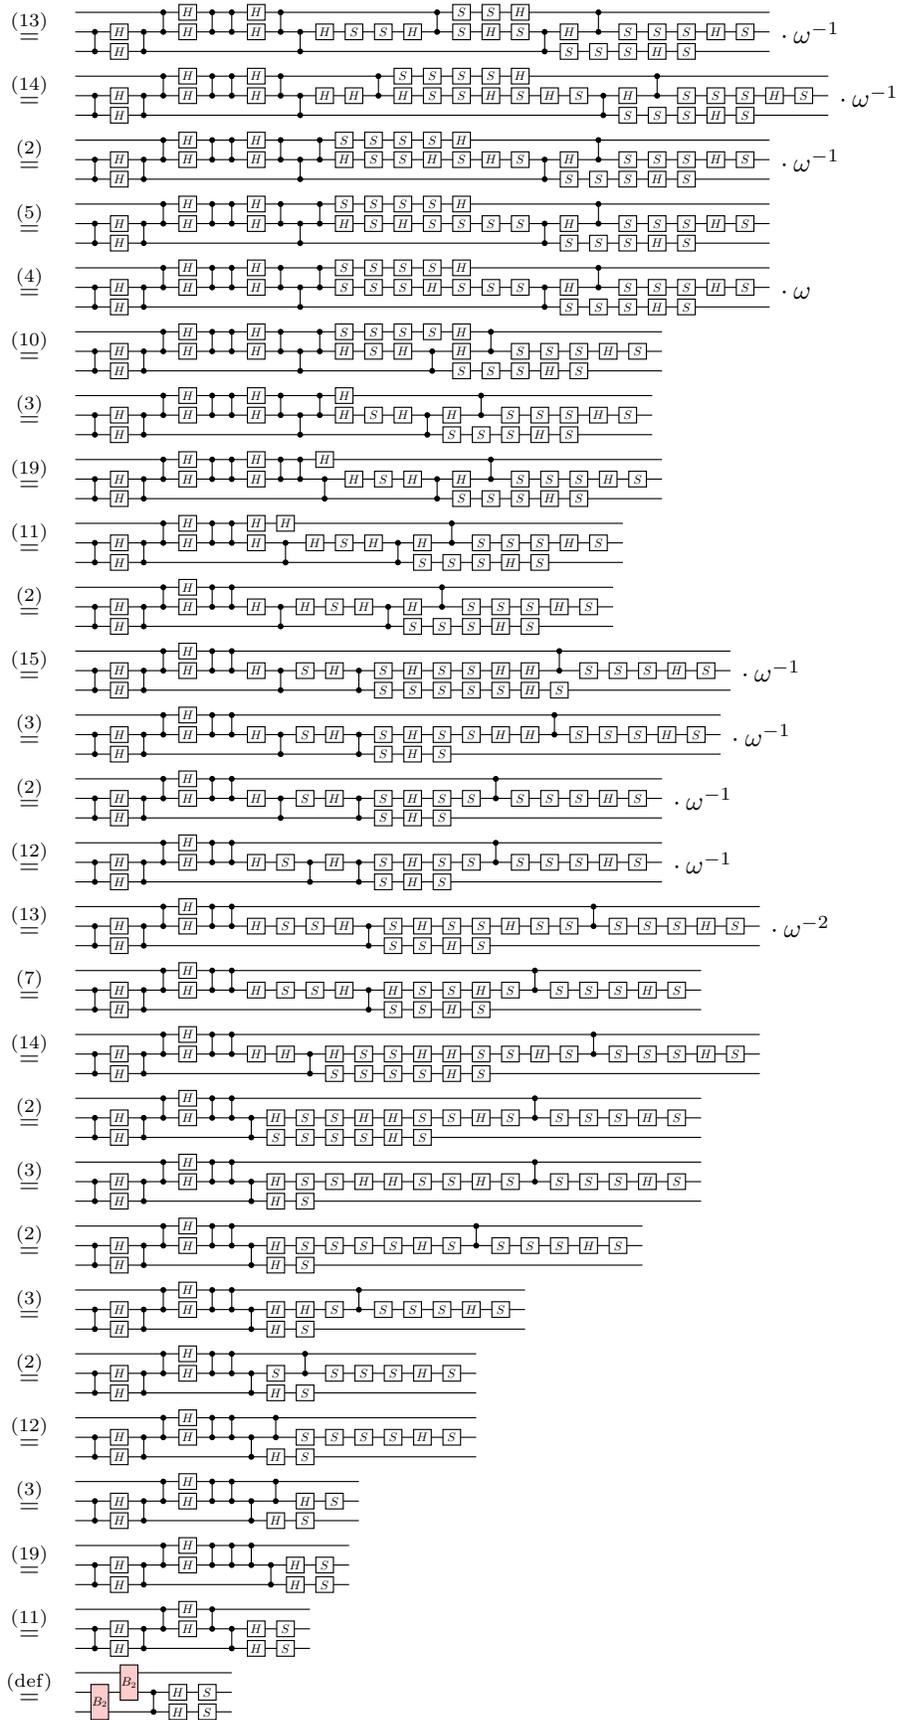

### 3.61 Equation

**Proof:**

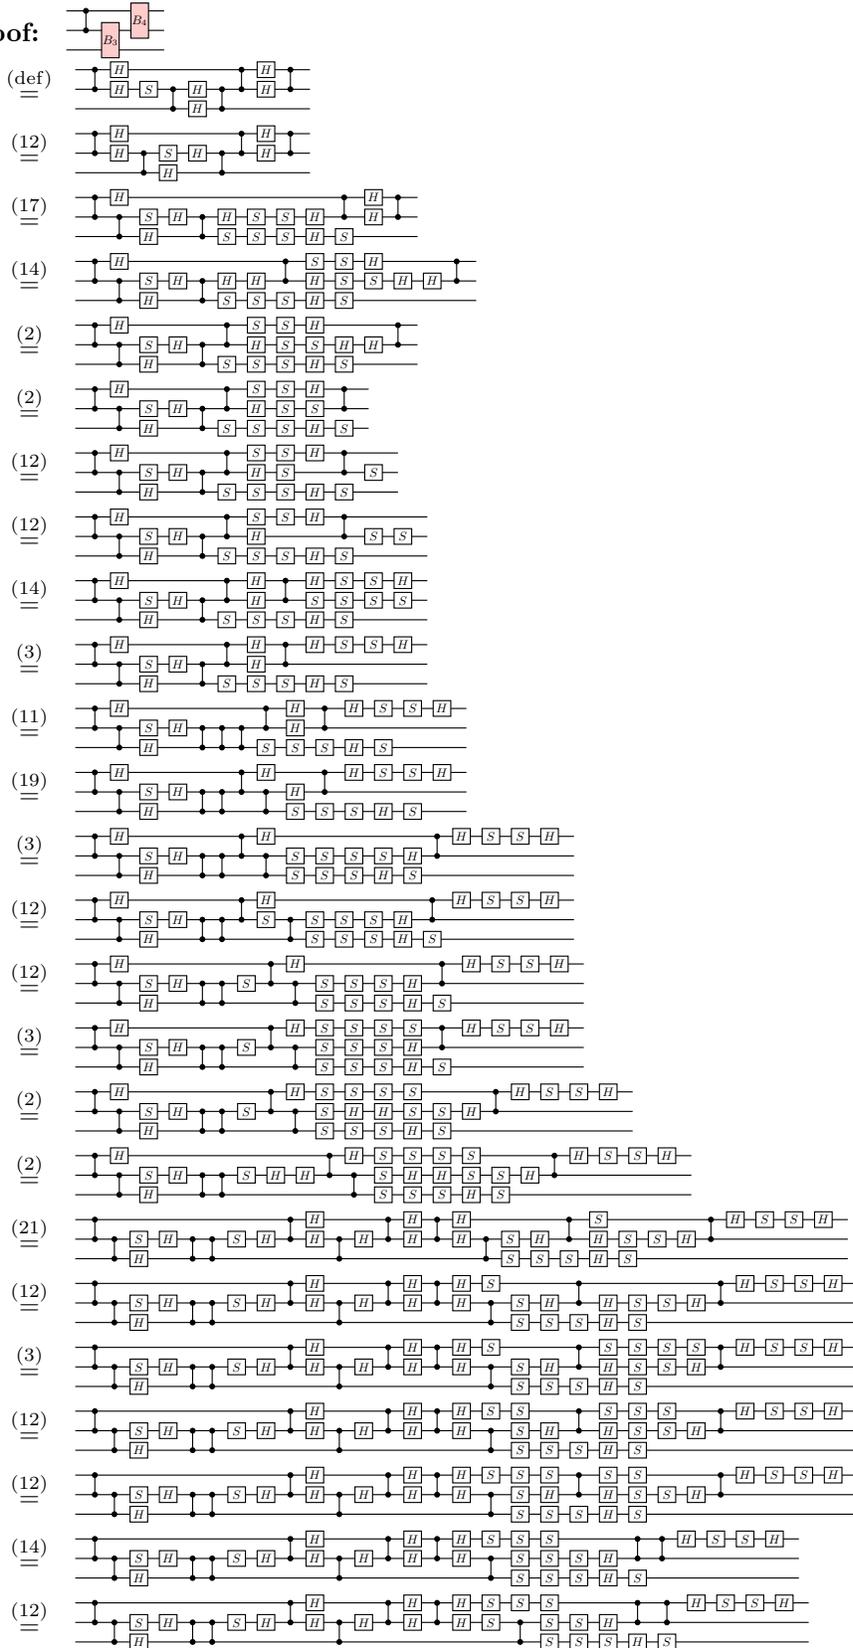

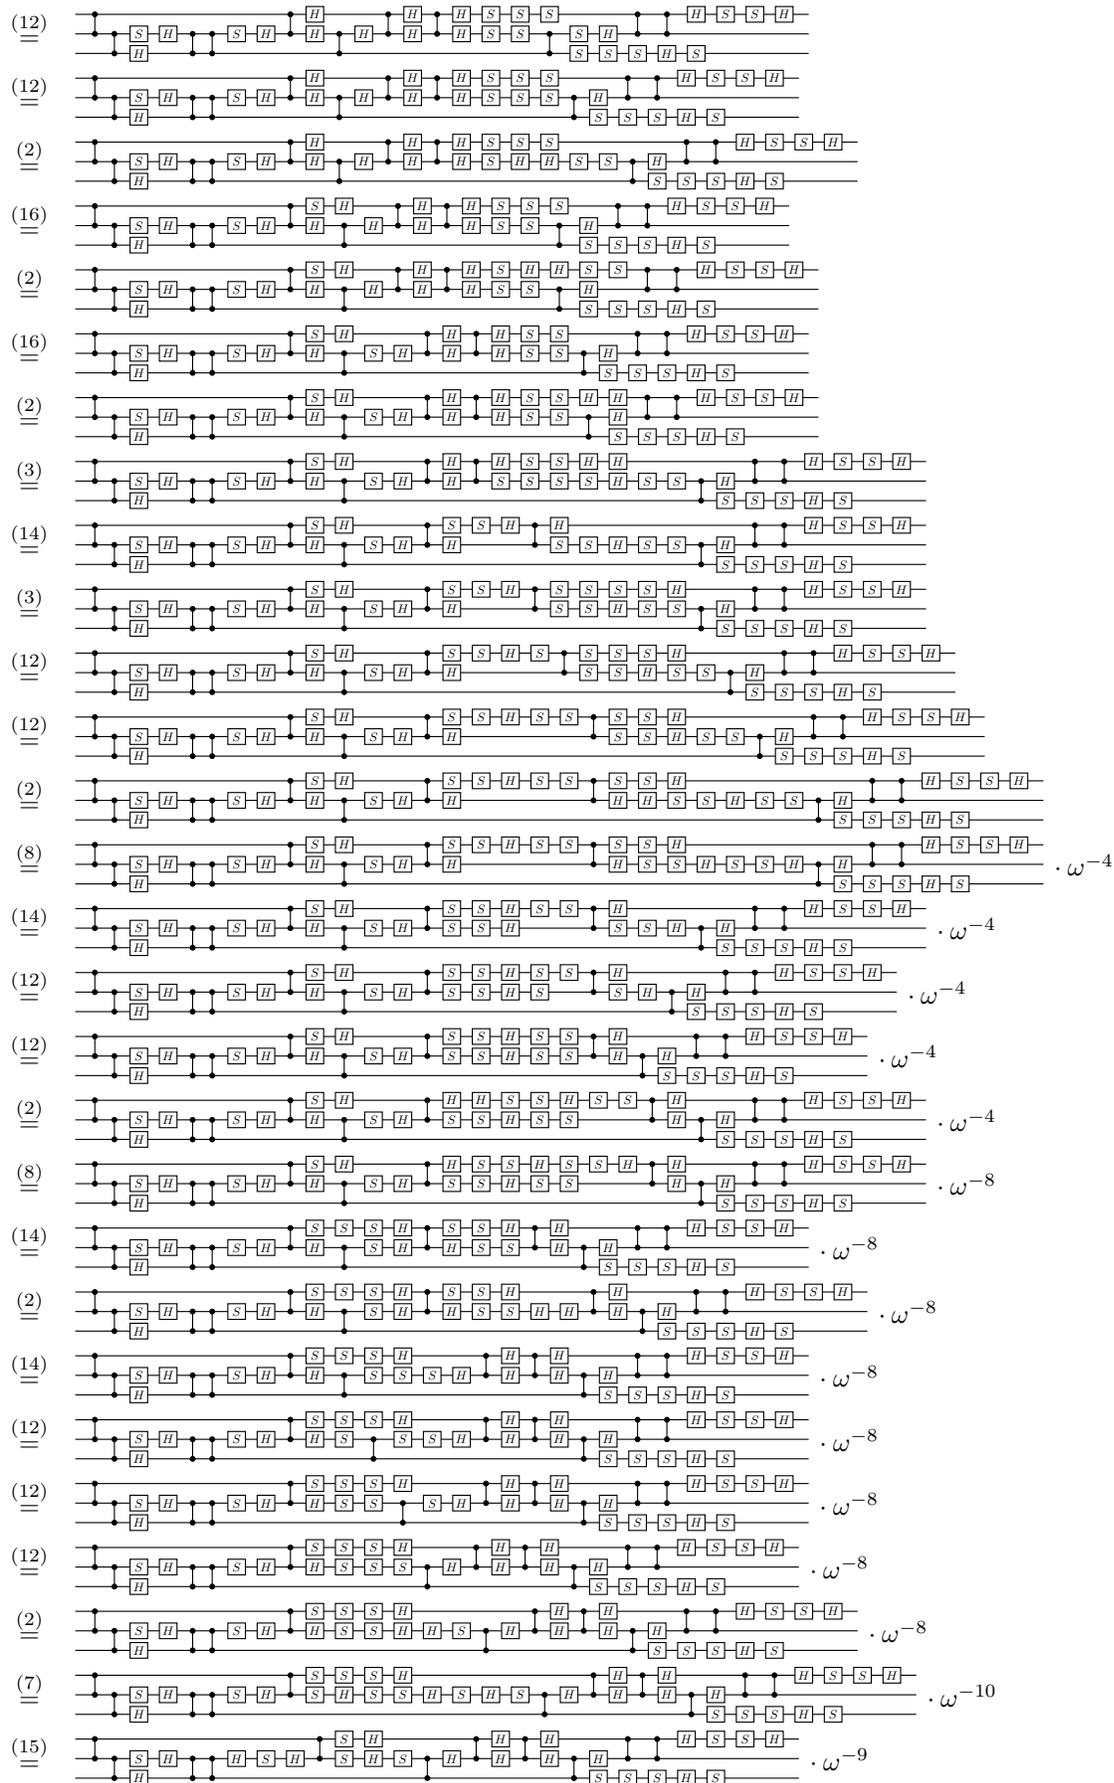

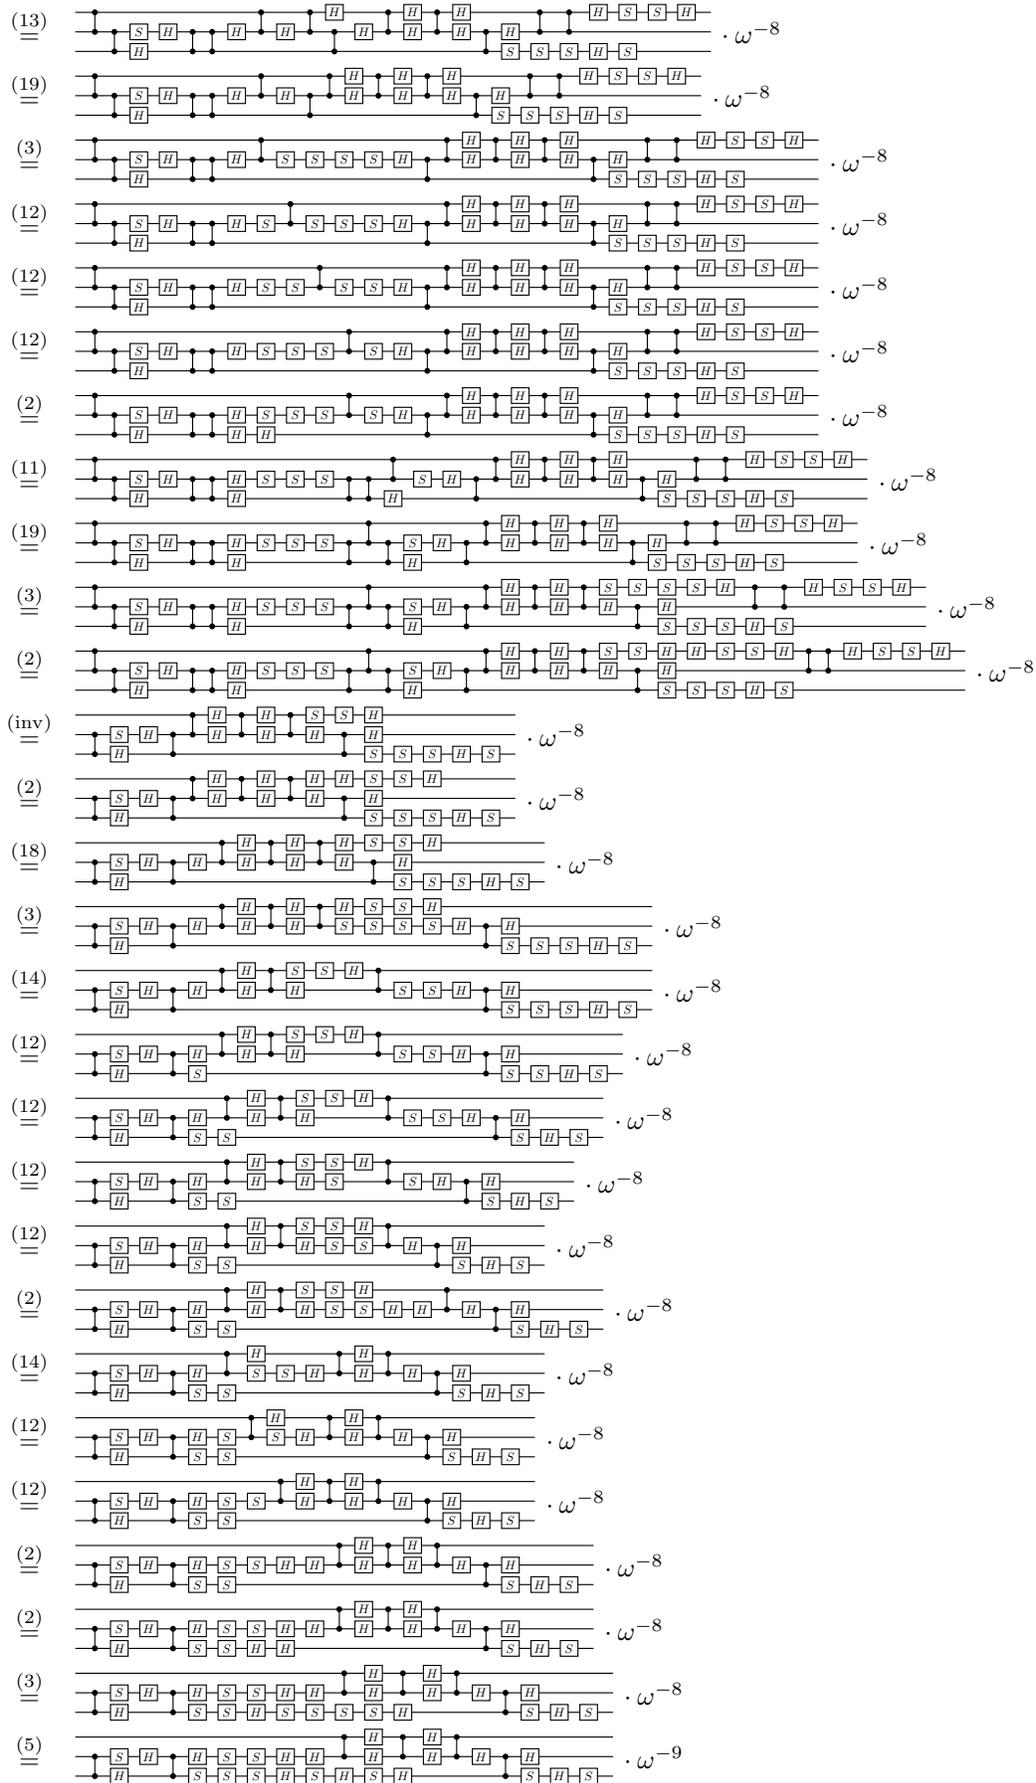

$$\begin{aligned}
(17) \quad & \text{---} \omega^{-9} \\
(12) \quad & \text{---} \omega^{-9} \\
(1) \quad & \text{---} \omega^7 \\
(\text{def}) \quad & \text{---} \omega^7
\end{aligned}$$

### 3.62 Equation

**Proof:**

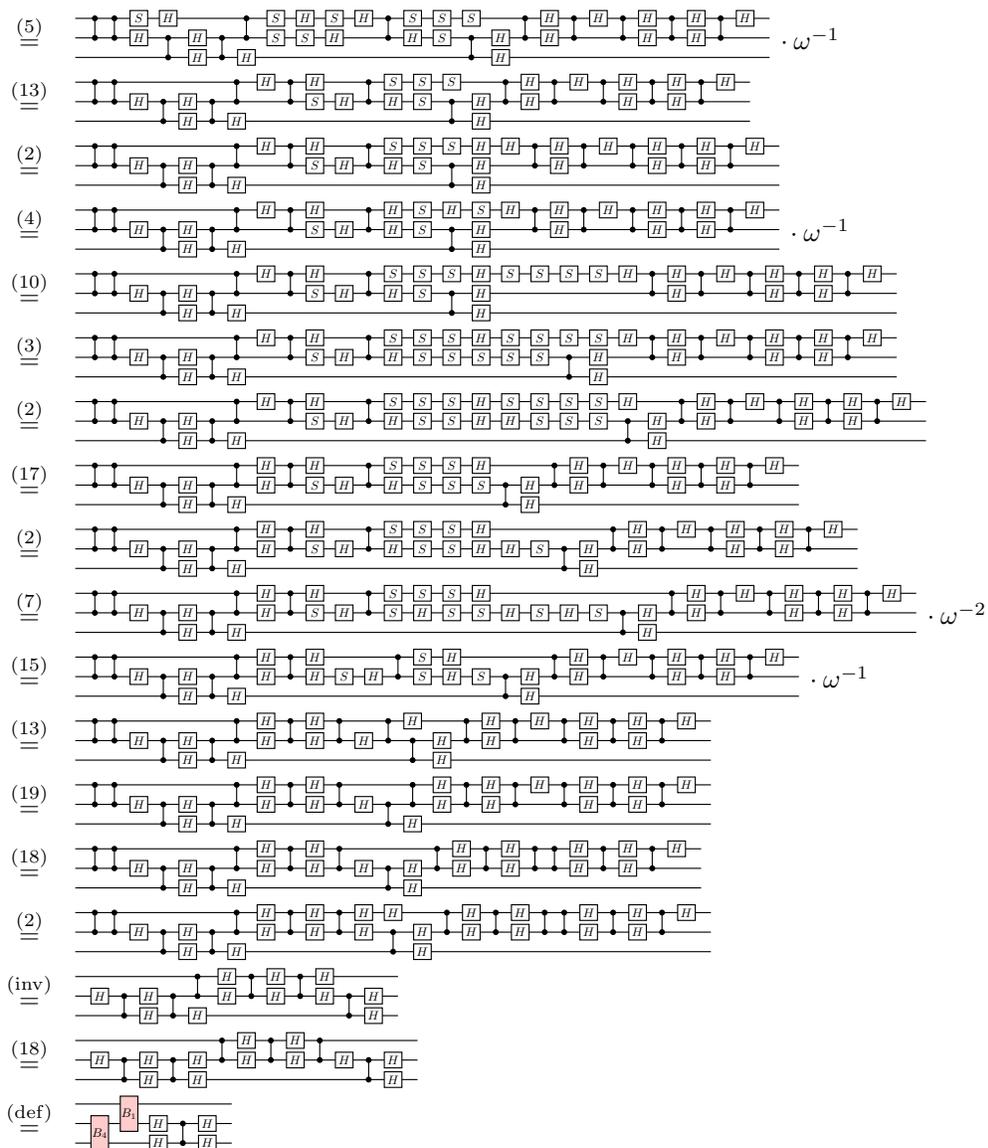

### 3.63 Equation

$$\begin{array}{c} \bullet \\ \bullet \end{array} \begin{array}{c} B_2 \\ B_1 \end{array} = \begin{array}{c} B_2 \\ B_1 \end{array} \begin{array}{c} H \\ H \end{array}$$

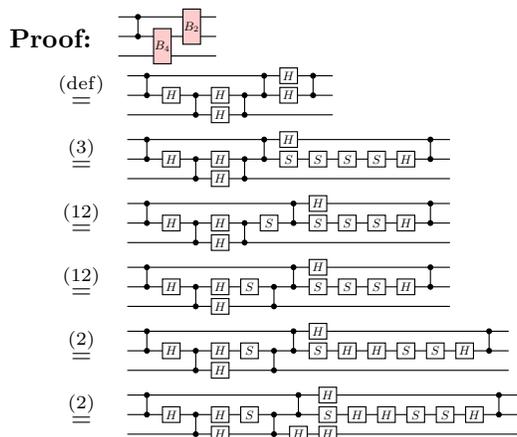

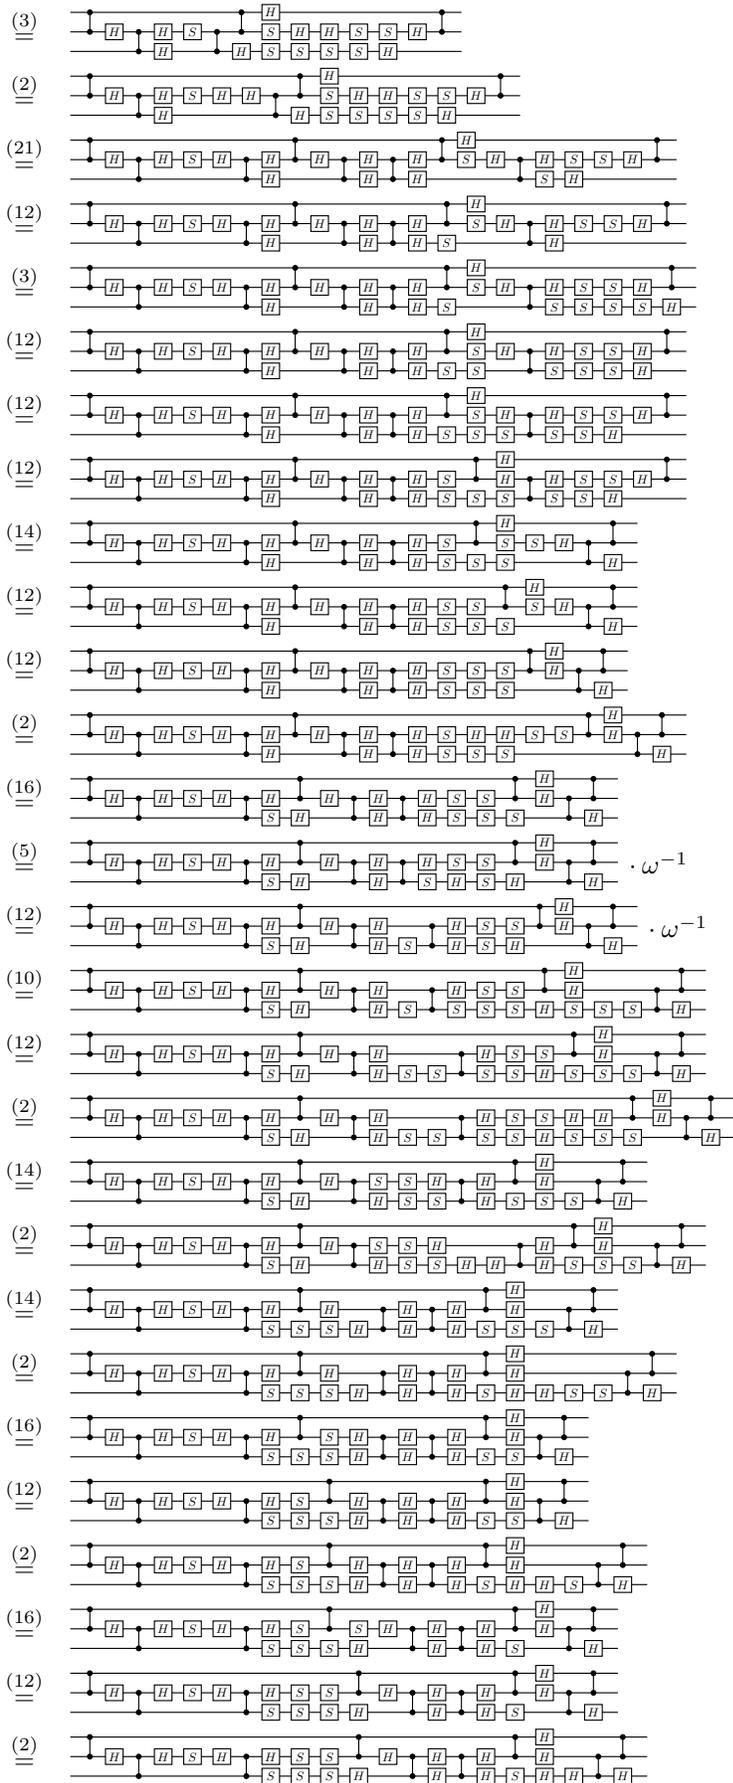

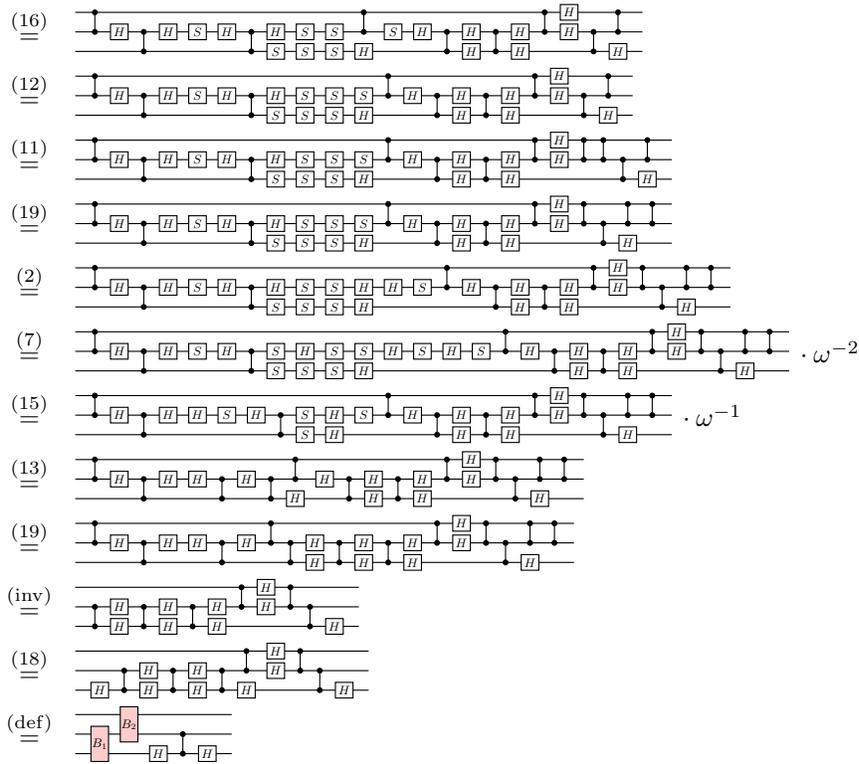

### 3.64 Equation

**Proof:**

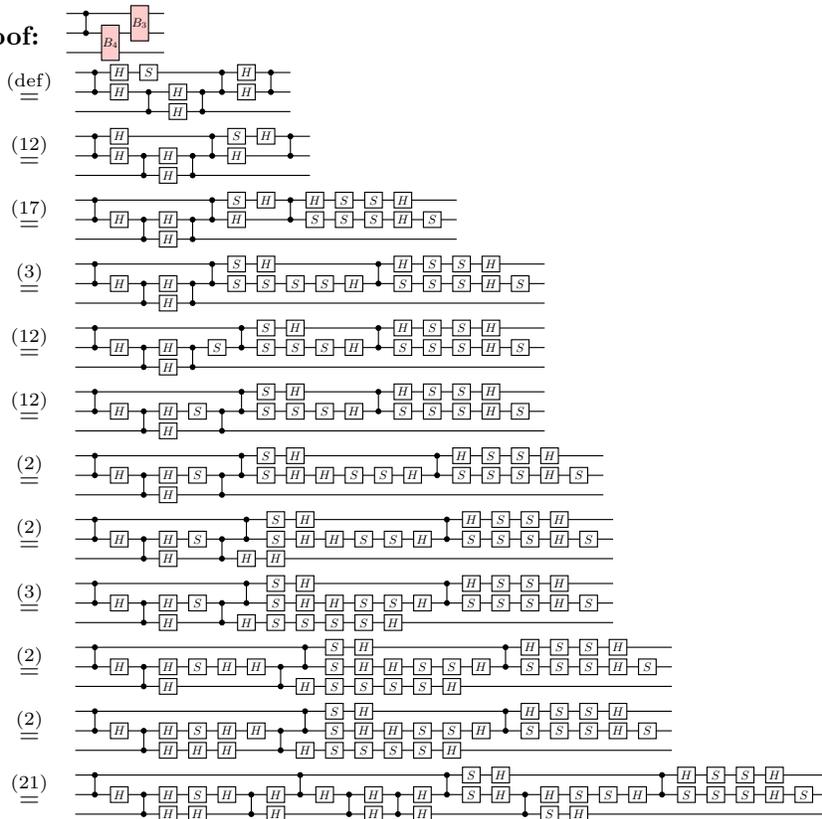

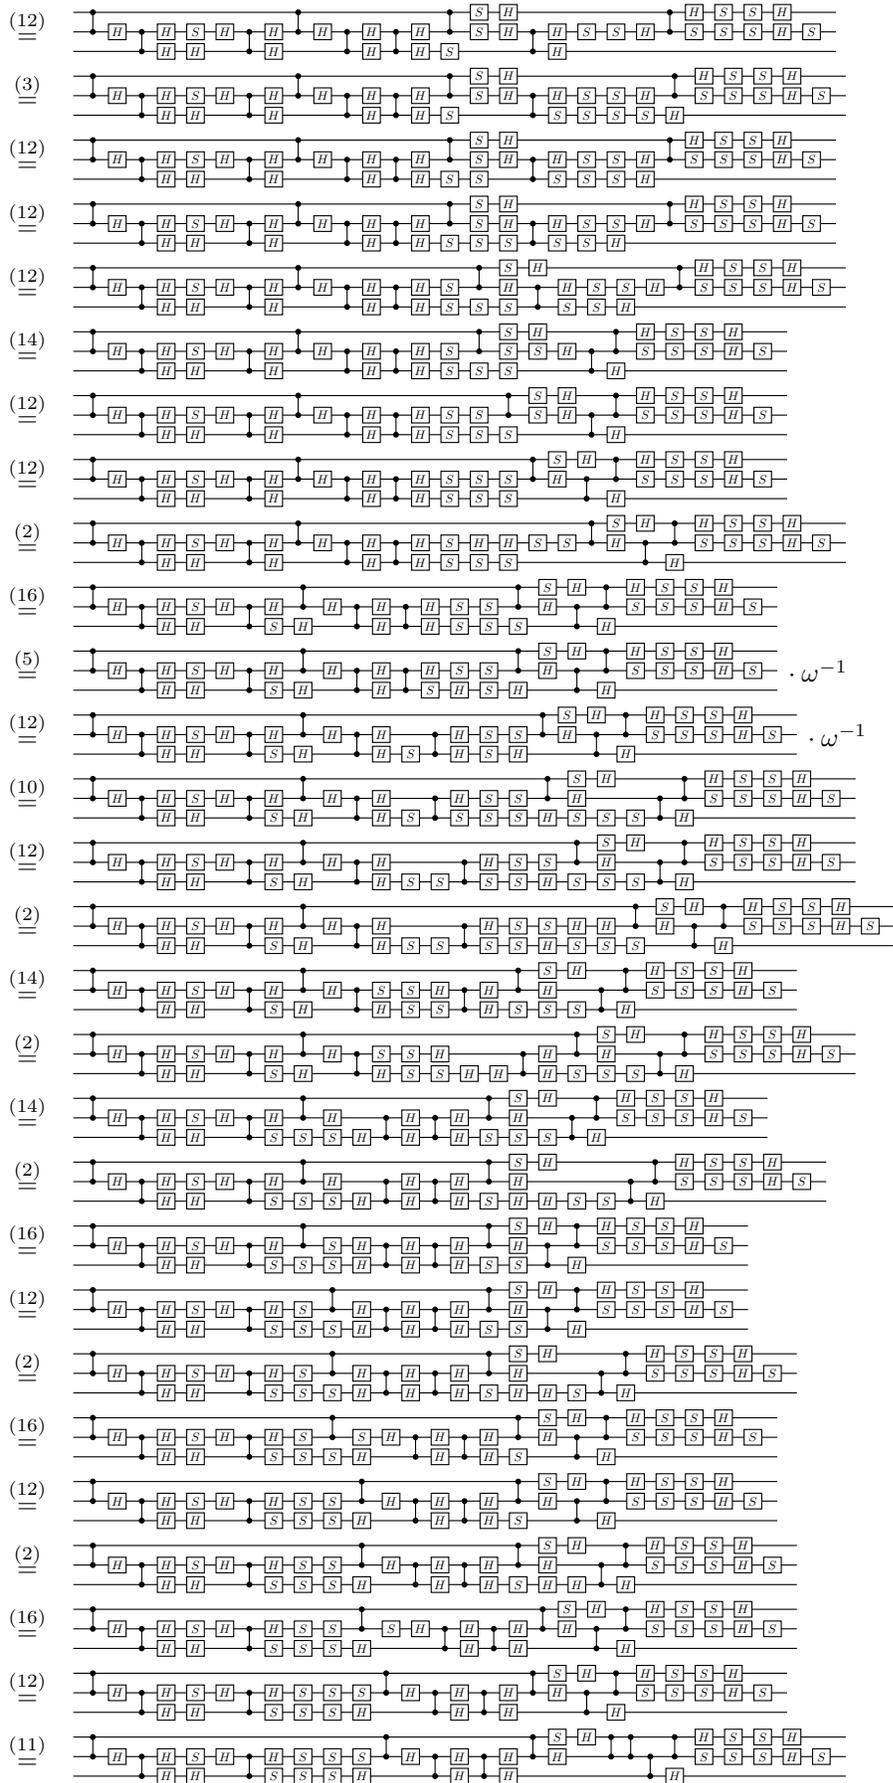

(19) 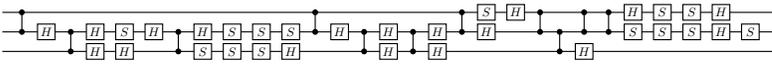  $\cdot \omega^{-2}$

(2) 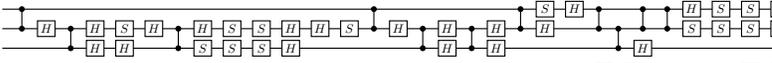  $\cdot \omega^{-1}$

(7) 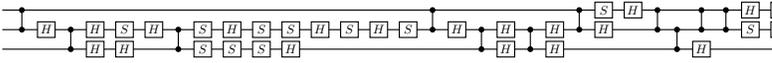  $\cdot \omega^{-1}$

(13) 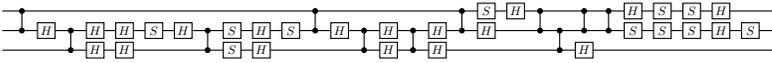  $\cdot \omega^{-1}$

(19) 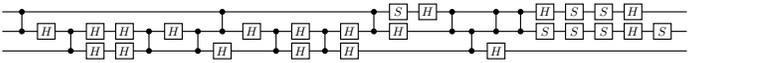  $\cdot \omega^{-1}$

(2) 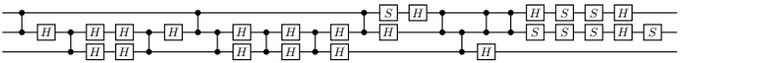  $\cdot \omega^{-1}$

(3) 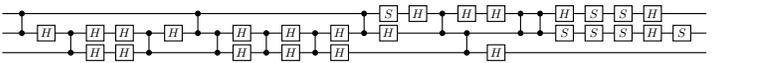  $\cdot \omega^{-1}$

(2) 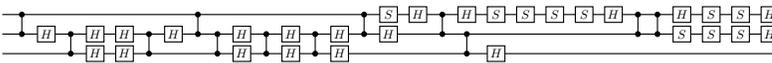  $\cdot \omega^{-1}$

(3) 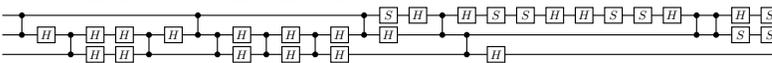  $\cdot \omega^{-1}$

(2) 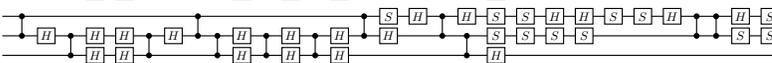  $\cdot \omega^{-1}$

(4) 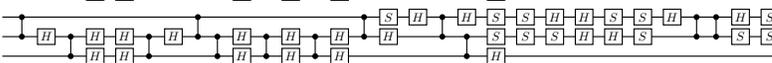  $\cdot \omega^{-1}$

(10) 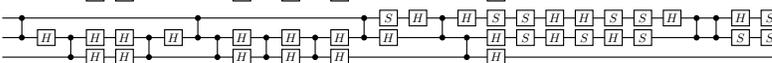  $\cdot \omega^{-1}$

(inv) 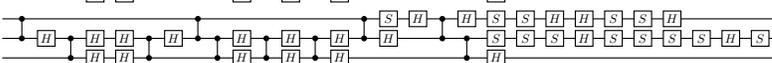  $\cdot \omega^{-1}$

(18) 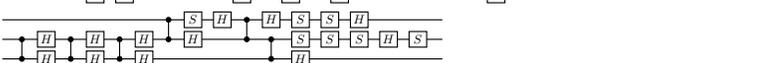  $\cdot \omega^{-1}$

(12) 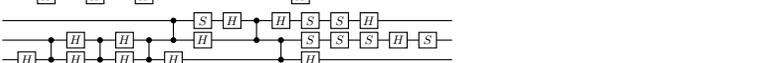  $\cdot \omega^{-1}$

(12) 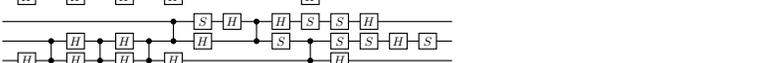  $\cdot \omega^{-1}$

(2) 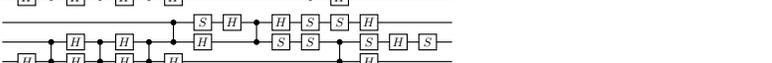  $\cdot \omega^{-1}$

(3) 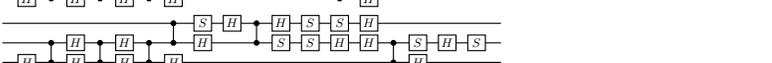  $\cdot \omega^{-1}$

(5) 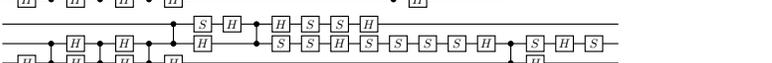  $\cdot \omega^{-1}$

(17) 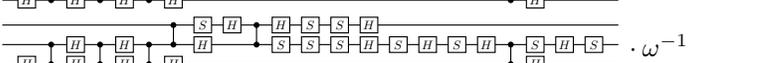  $\cdot \omega^{-1}$

(12) 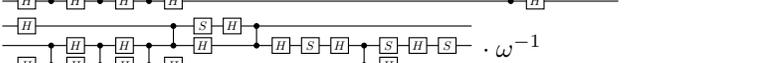  $\cdot \omega^{-1}$

(1) 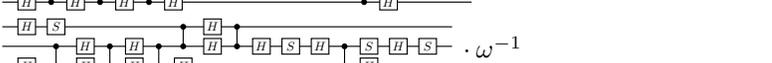  $\cdot \omega^7$

(def) 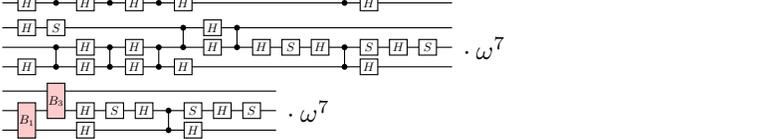  $\cdot \omega^7$

### 3.65 Equation

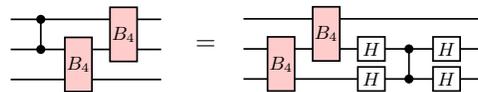

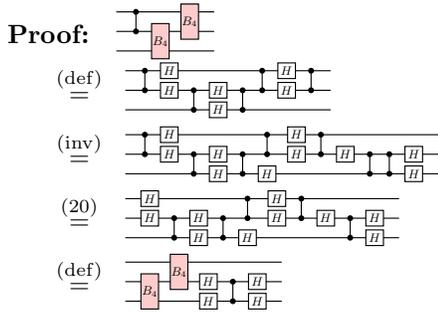

### 3.66 Equation

$$\begin{array}{c} \text{---} \\ | \\ \text{---} \end{array} \begin{array}{c} \boxed{D_1} \\ | \\ \text{---} \end{array} = \begin{array}{c} \text{---} \\ | \\ \text{---} \end{array} \begin{array}{c} \boxed{D_1} \\ | \\ \text{---} \end{array} \begin{array}{c} \boxed{H} \\ | \\ \text{---} \end{array}$$

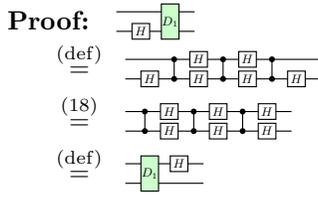

### 3.67 Equation

$$\begin{array}{c} \text{---} \\ | \\ \text{---} \end{array} \begin{array}{c} \boxed{D_2} \\ | \\ \text{---} \end{array} = \begin{array}{c} \text{---} \\ | \\ \text{---} \end{array} \begin{array}{c} \boxed{D_4} \\ | \\ \text{---} \end{array}$$

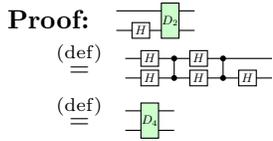

### 3.68 Equation

$$\begin{array}{c} \text{---} \\ | \\ \text{---} \end{array} \begin{array}{c} \boxed{D_3} \\ | \\ \text{---} \end{array} = \begin{array}{c} \text{---} \\ | \\ \text{---} \end{array} \begin{array}{c} \boxed{D_3} \\ | \\ \text{---} \end{array} \begin{array}{c} \boxed{S} \\ | \\ \text{---} \end{array} \begin{array}{c} \boxed{S} \\ | \\ \text{---} \end{array} \begin{array}{c} \boxed{S} \\ | \\ \text{---} \end{array} \begin{array}{c} \boxed{H} \\ | \\ \text{---} \end{array} \begin{array}{c} \boxed{S} \\ | \\ \text{---} \end{array}$$

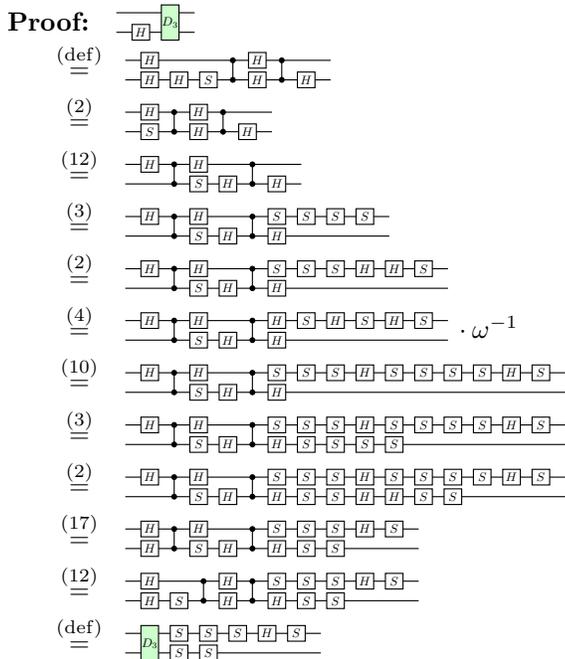



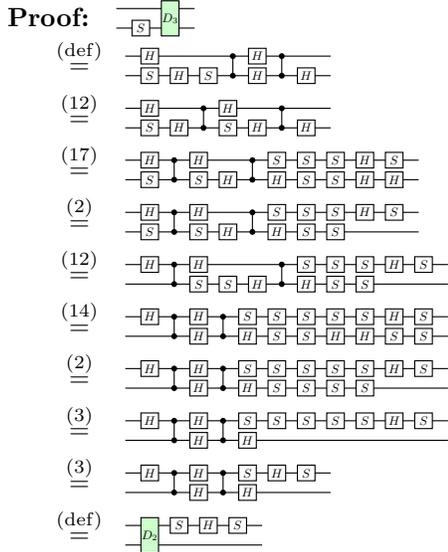

### 3.73 Equation

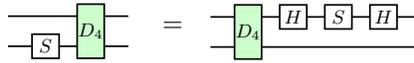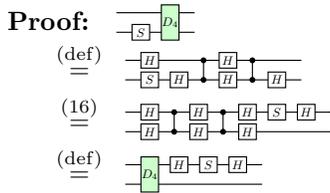

### 3.74 Equation

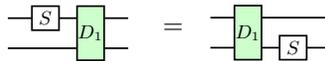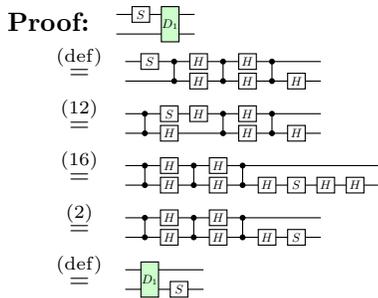

### 3.75 Equation

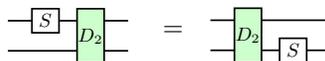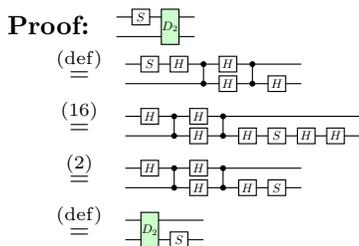

### 3.76 Equation

$$\begin{array}{c} \boxed{S} \\ \hline \end{array} \begin{array}{c} \boxed{D_3} \\ \hline \end{array} = \begin{array}{c} \boxed{D_3} \\ \hline \end{array} \begin{array}{c} \boxed{S} \\ \hline \end{array}$$

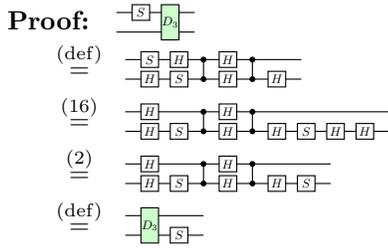

### 3.77 Equation

$$\begin{array}{c} \boxed{S} \\ \hline \end{array} \begin{array}{c} \boxed{D_4} \\ \hline \end{array} = \begin{array}{c} \boxed{D_4} \\ \hline \end{array} \begin{array}{c} \boxed{S} \\ \hline \end{array}$$

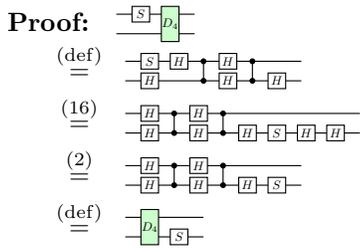

### 3.78 Equation

$$\begin{array}{c} \bullet \\ \bullet \\ \hline \end{array} \begin{array}{c} \boxed{D_1} \\ \hline \end{array} = \begin{array}{c} \boxed{D_4} \\ \hline \end{array}$$

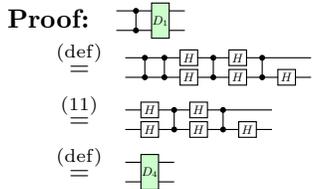

### 3.79 Equation

$$\begin{array}{c} \bullet \\ \bullet \\ \hline \end{array} \begin{array}{c} \boxed{D_2} \\ \hline \end{array} = \begin{array}{c} \boxed{D_3} \\ \hline \end{array} \begin{array}{c} \boxed{S} \\ \hline \end{array} \begin{array}{c} \boxed{S} \\ \hline \end{array} \begin{array}{c} \boxed{S} \\ \hline \end{array} \begin{array}{c} \boxed{H} \\ \hline \end{array}$$

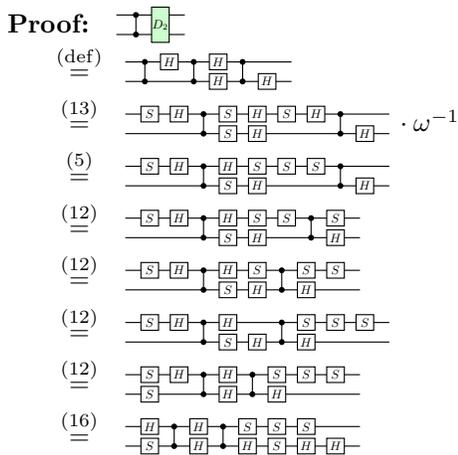

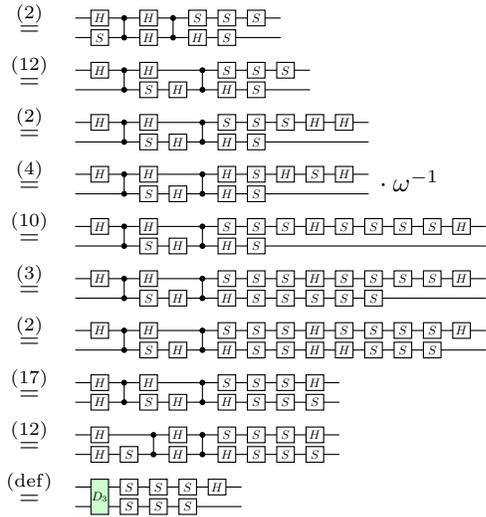

### 3.80 Equation

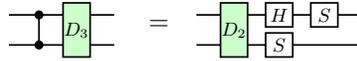

**Proof:**

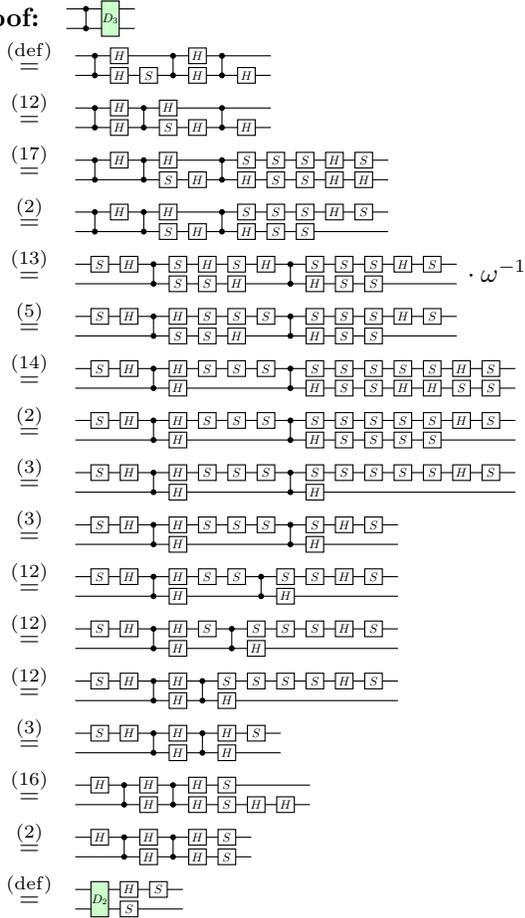

### 3.81 Equation

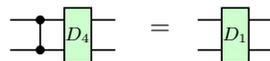

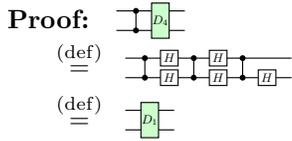

### 3.82 Equation

$$-S-E_1- = -E_2-$$

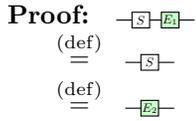

### 3.83 Equation

$$-S-E_2- = -E_3-$$

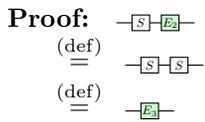

### 3.84 Equation

$$-S-E_3- = -E_4-$$

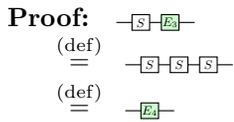

### 3.85 Equation

$$-S-E_4- = -E_1-$$

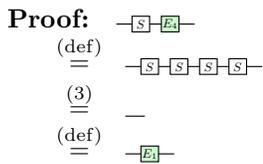

### 3.86 Equation

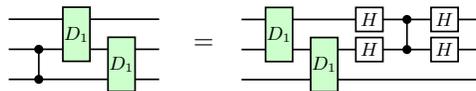

**Proof:**

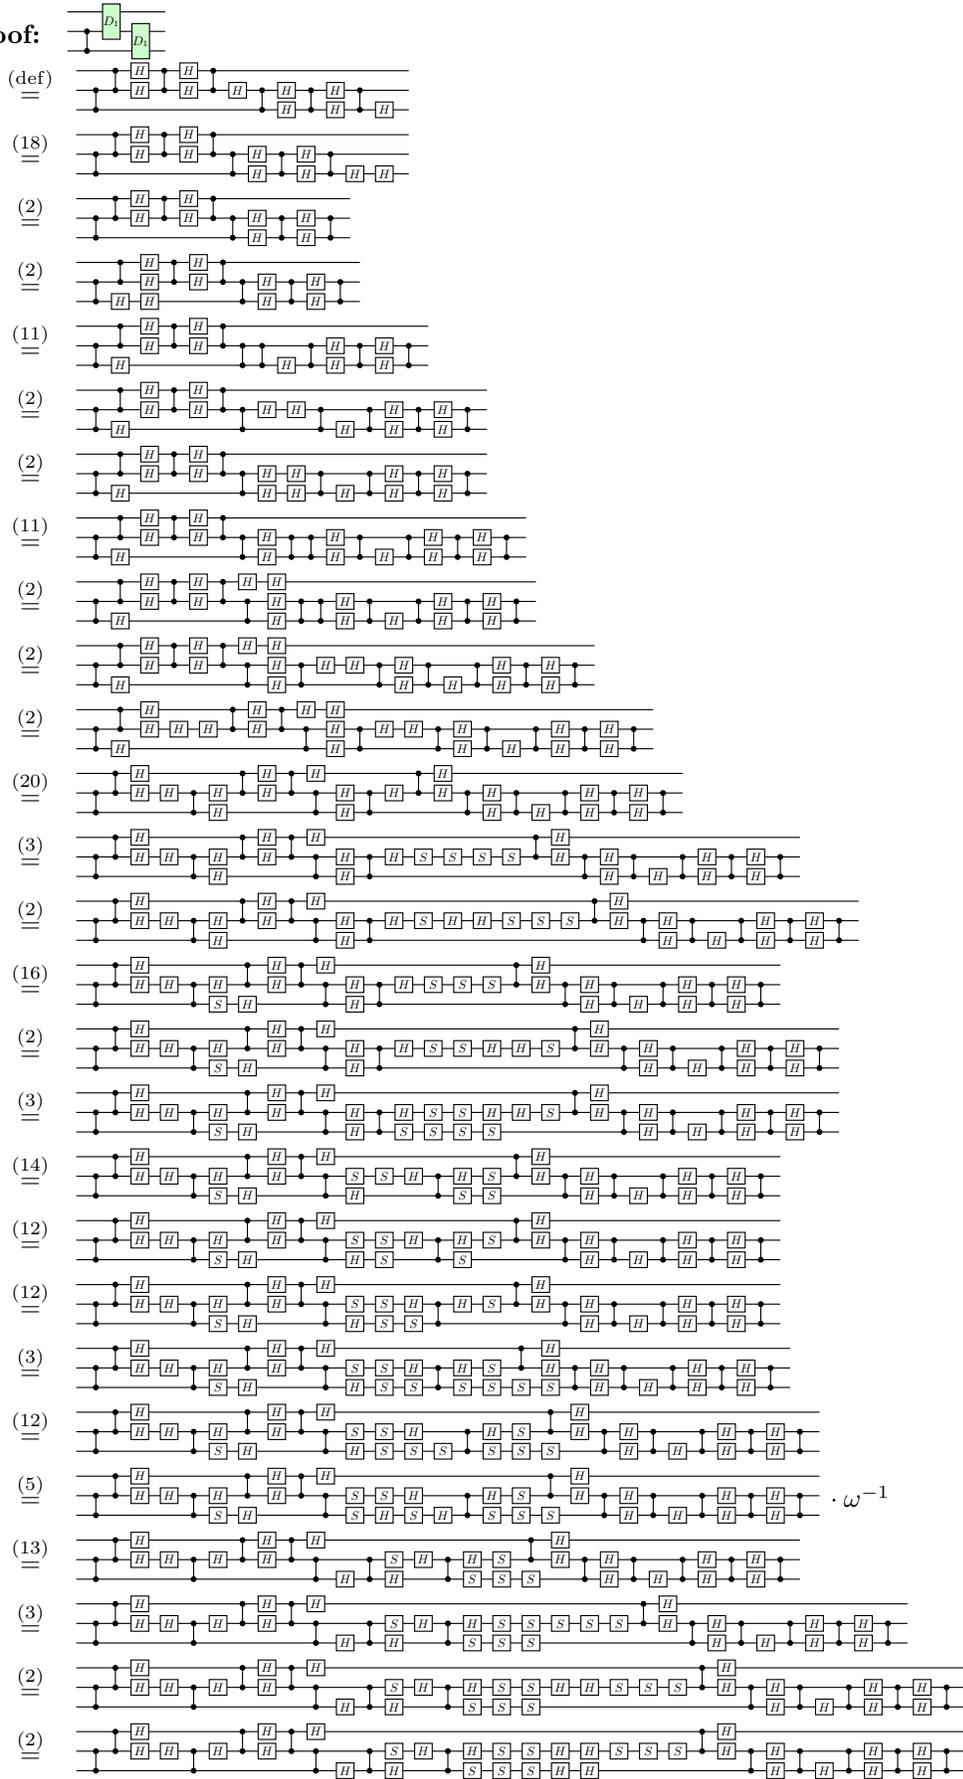

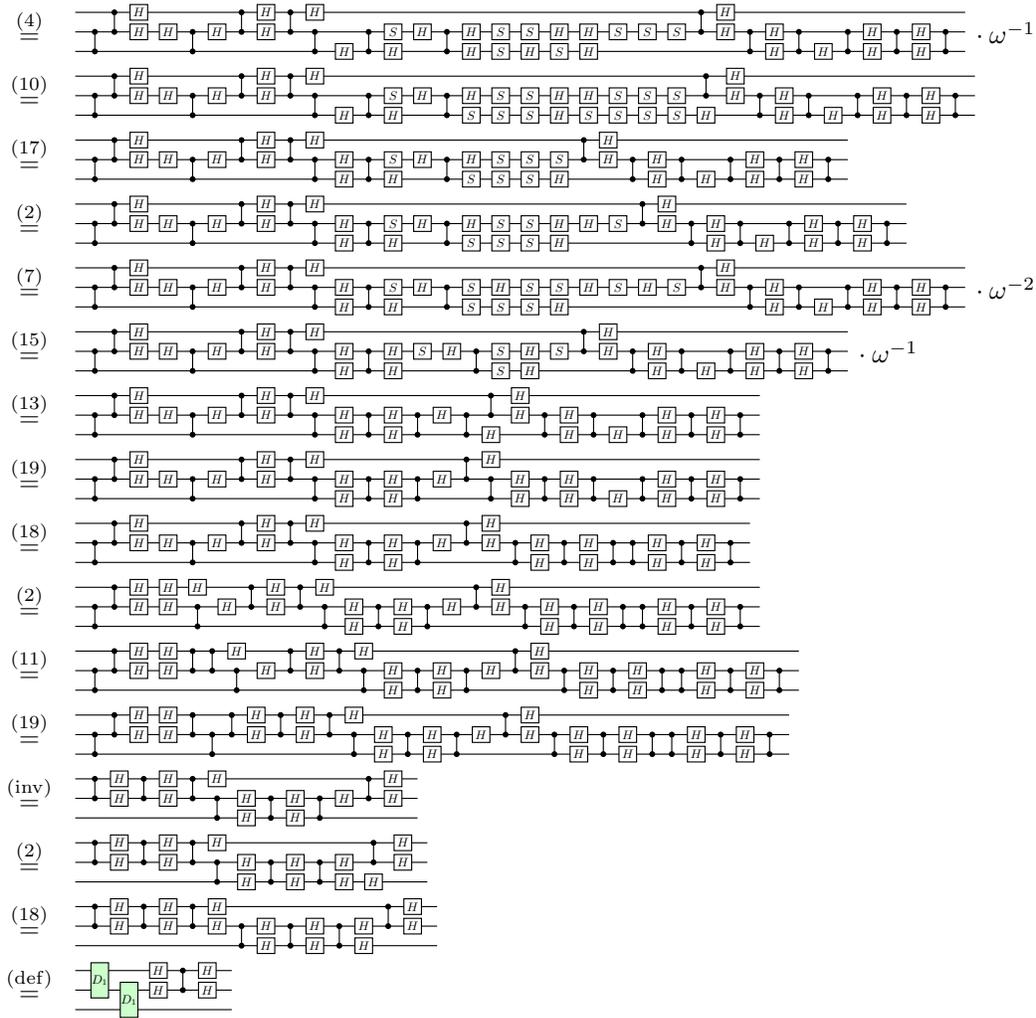

### 3.87 Equation

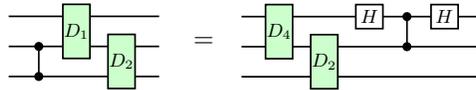

**Proof:**

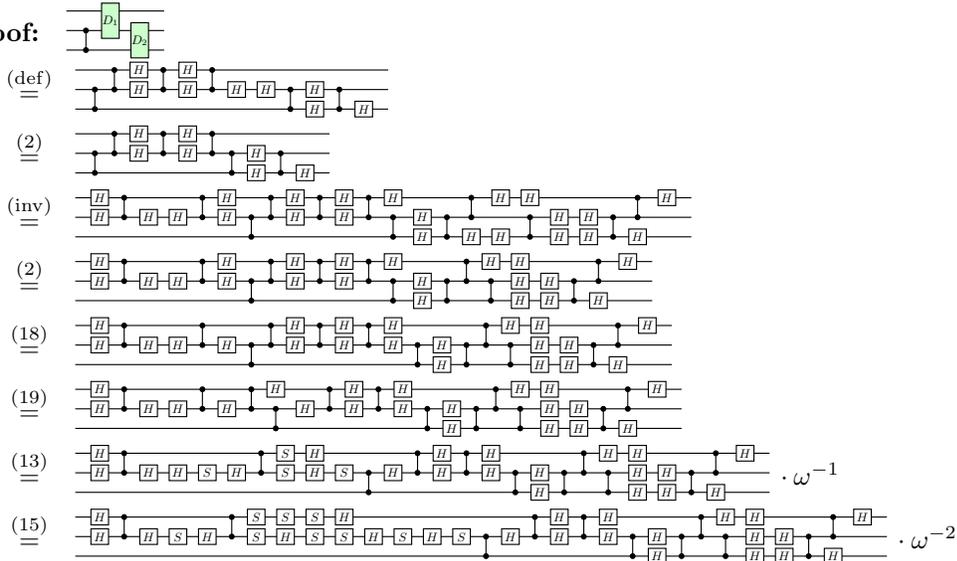

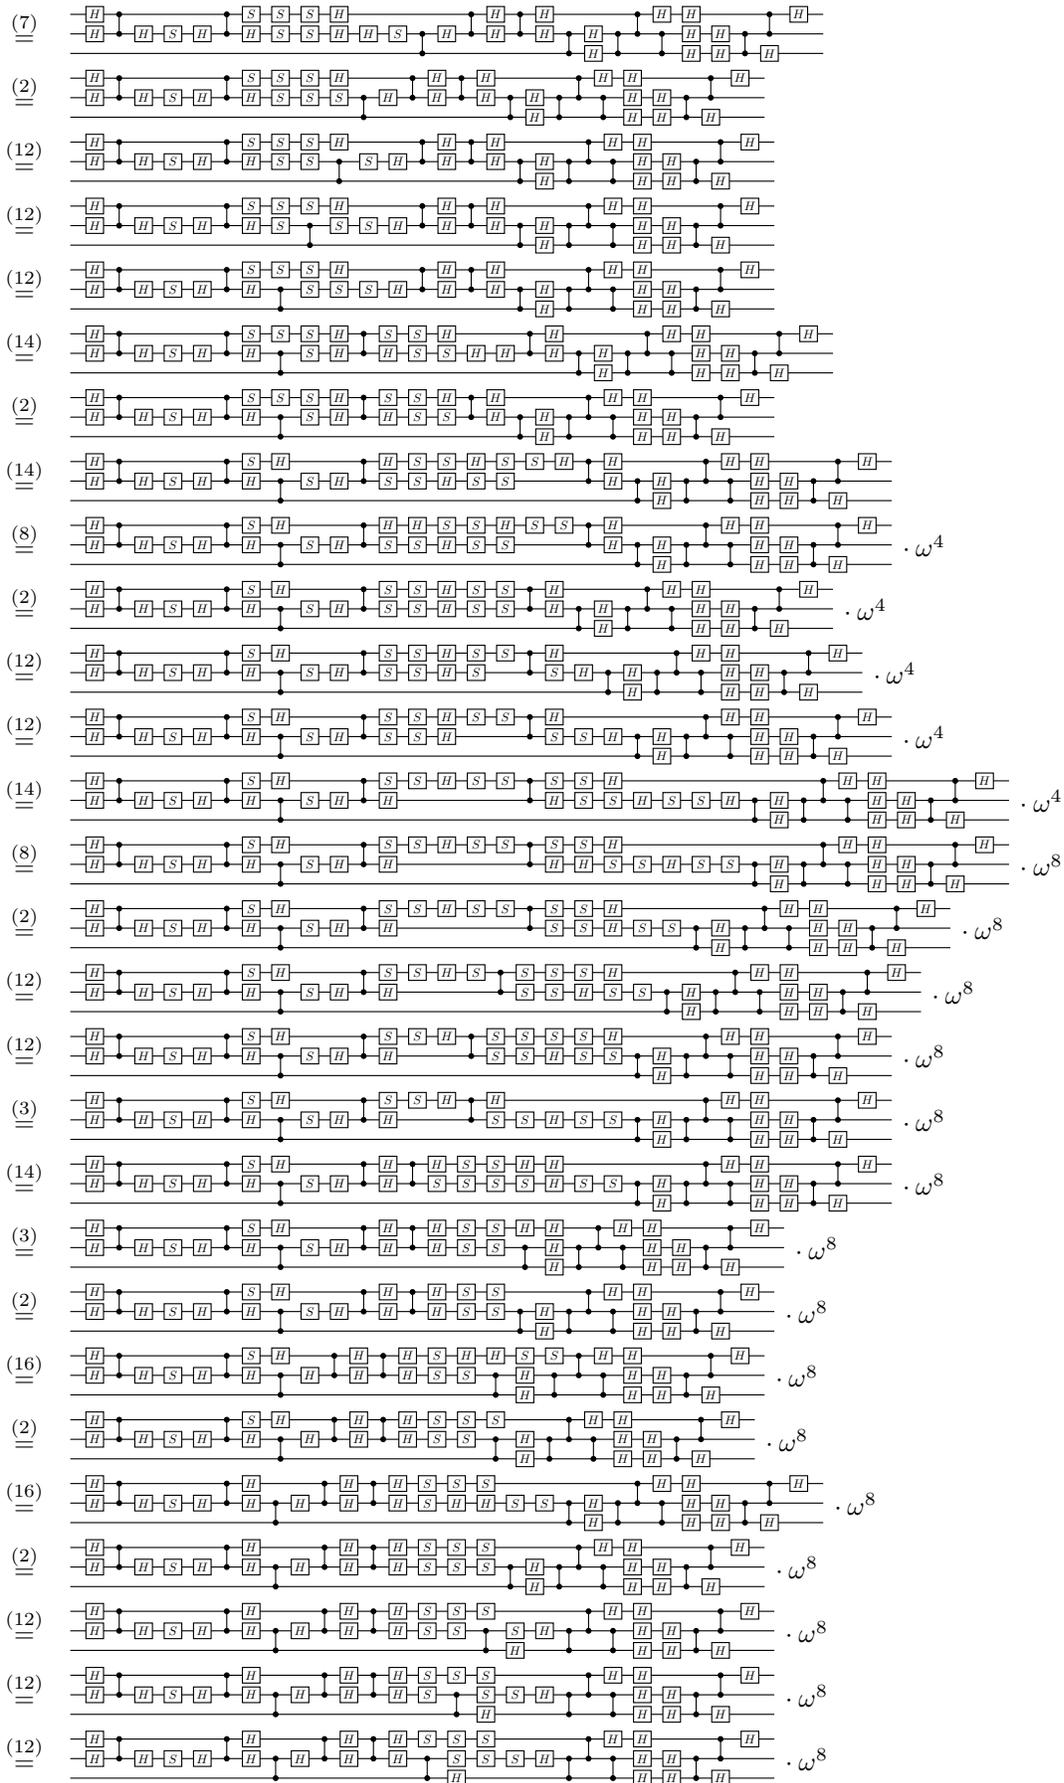

(19) 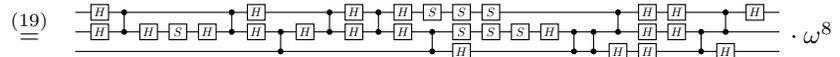 · ω<sup>8</sup>

(11) 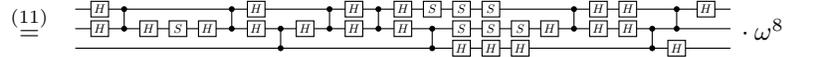 · ω<sup>8</sup>

(2) 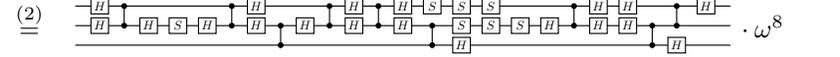 · ω<sup>8</sup>

(14) 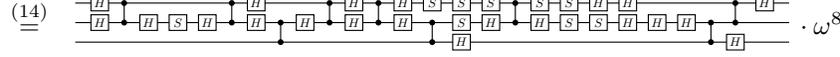 · ω<sup>8</sup>

(2) 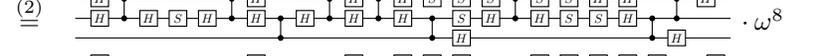 · ω<sup>8</sup>

(12) 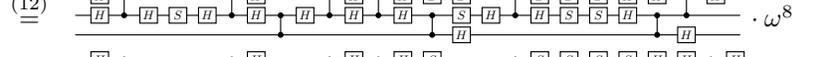 · ω<sup>8</sup>

(12) 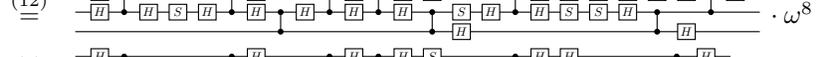 · ω<sup>8</sup>

(3) 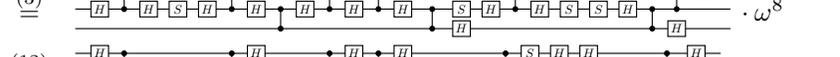 · ω<sup>8</sup>

(12) 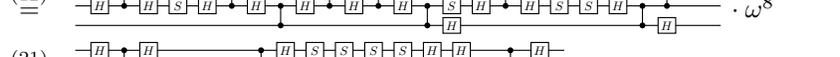 · ω<sup>8</sup>

(21) 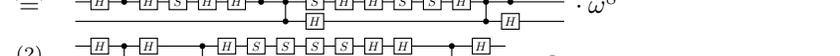 · ω<sup>8</sup>

(2) 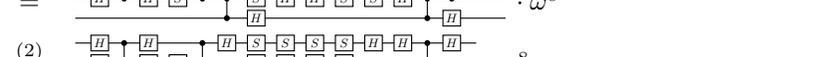 · ω<sup>8</sup>

(2) 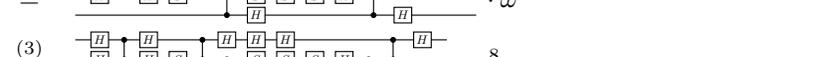 · ω<sup>8</sup>

(3) 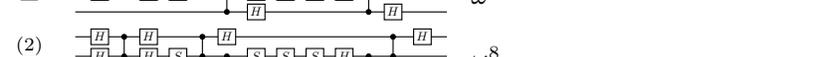 · ω<sup>8</sup>

(2) 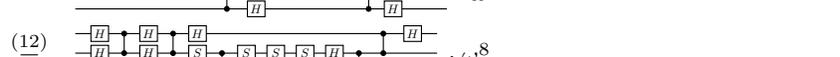 · ω<sup>8</sup>

(12) 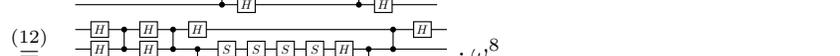 · ω<sup>8</sup>

(12) 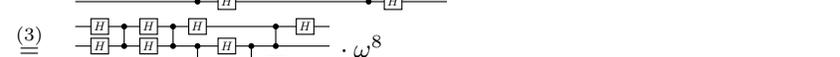 · ω<sup>8</sup>

(3) 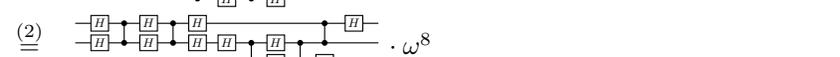 · ω<sup>8</sup>

(2) 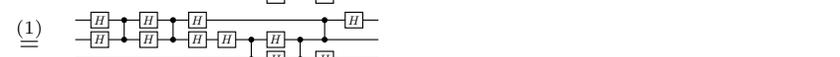 · ω<sup>8</sup>

(1) 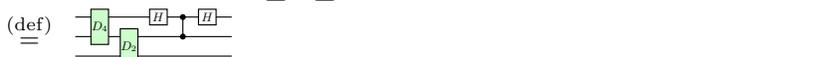 · ω<sup>8</sup>

(def) 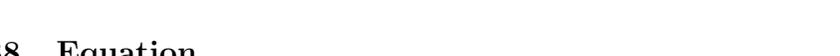 · ω<sup>8</sup>

### 3.88 Equation

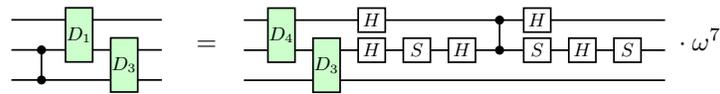 · ω<sup>7</sup>

**Proof:**

(def) 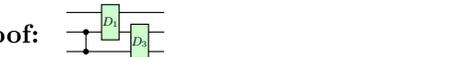

(2) 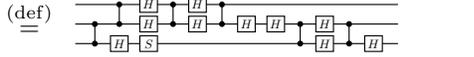

(12) 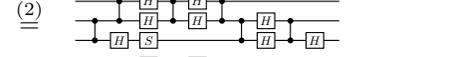

(17) 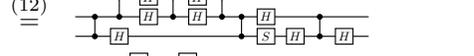

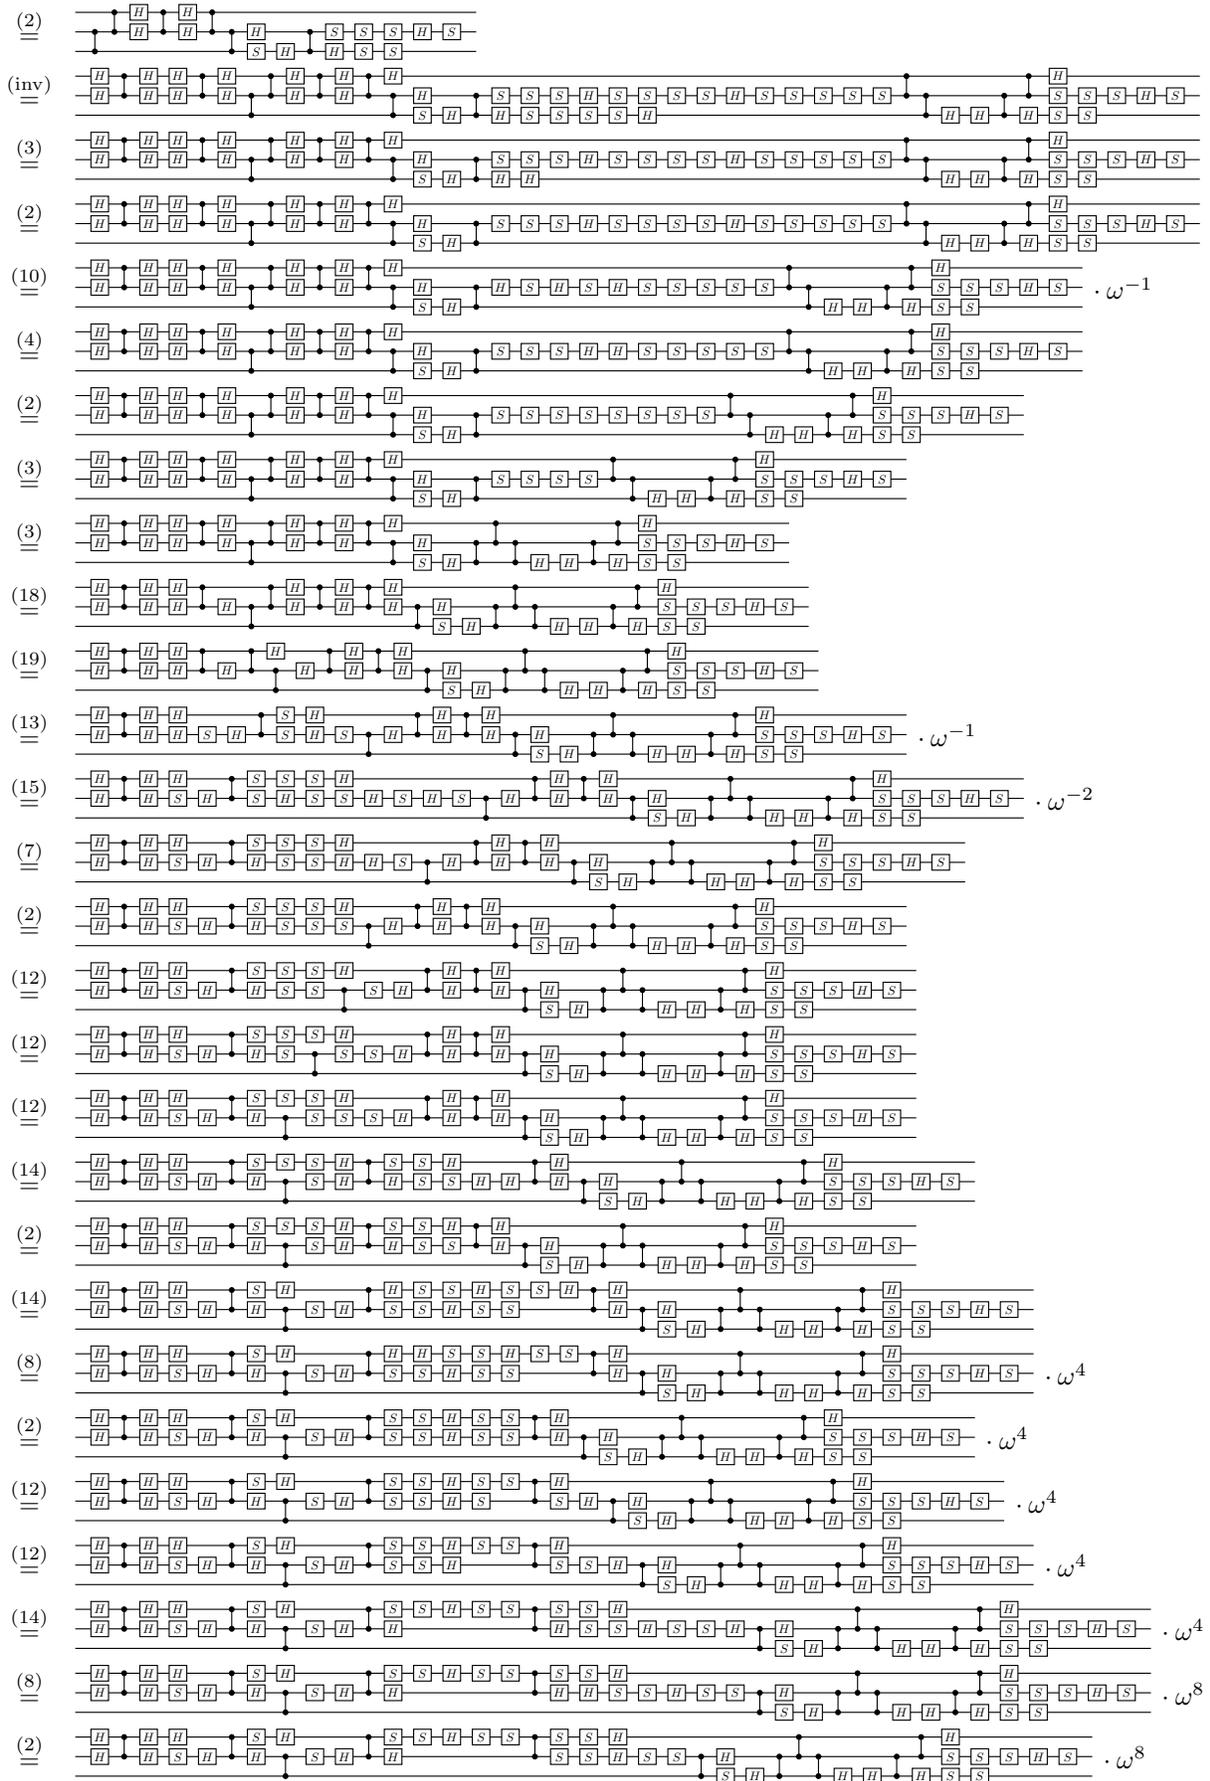

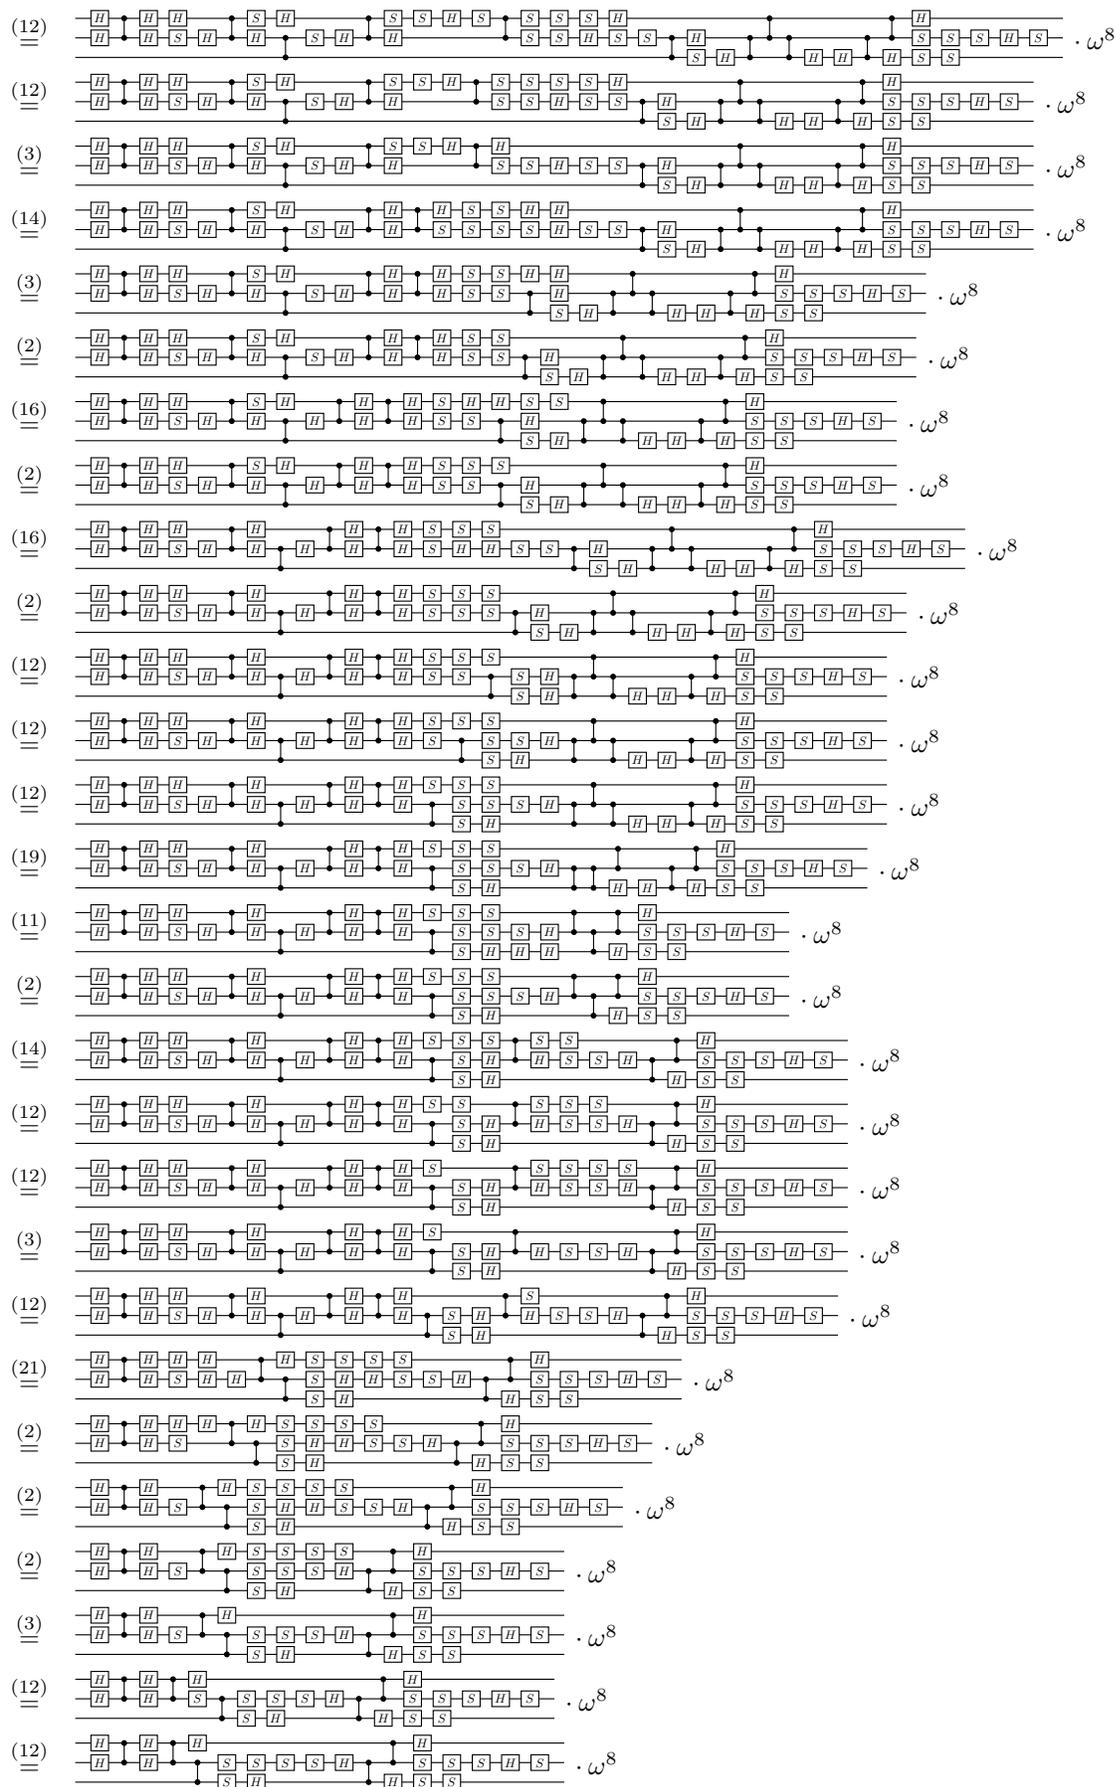

$$\begin{aligned}
& \underline{(3)} \quad \text{[Diagram with 4 qubits, 8 H gates, 4 S gates]} \cdot \omega^8 \\
& \underline{(12)} \quad \text{[Diagram with 4 qubits, 8 H gates, 4 S gates]} \cdot \omega^8 \\
& \underline{(12)} \quad \text{[Diagram with 4 qubits, 8 H gates, 4 S gates]} \cdot \omega^8 \\
& \underline{(2)} \quad \text{[Diagram with 4 qubits, 8 H gates, 4 S gates]} \cdot \omega^8 \\
& \underline{(3)} \quad \text{[Diagram with 4 qubits, 8 H gates, 4 S gates]} \cdot \omega^8 \\
& \underline{(5)} \quad \text{[Diagram with 4 qubits, 8 H gates, 4 S gates]} \cdot \omega^7 \\
& \underline{(2)} \quad \text{[Diagram with 4 qubits, 8 H gates, 4 S gates]} \cdot \omega^7 \\
& \underline{(17)} \quad \text{[Diagram with 4 qubits, 8 H gates, 4 S gates]} \cdot \omega^7 \\
& \underline{(12)} \quad \text{[Diagram with 4 qubits, 8 H gates, 4 S gates]} \cdot \omega^7 \\
& \underline{(2)} \quad \text{[Diagram with 4 qubits, 8 H gates, 4 S gates]} \cdot \omega^7 \\
& \underline{(\text{def})} \quad \text{[Diagram with 4 qubits, 8 H gates, 4 S gates, and 2 D gates]} \cdot \omega^7
\end{aligned}$$

### 3.89 Equation

$$\text{[Diagram: } D_1 \text{ and } D_4 \text{ gates on two qubits]} = \text{[Diagram: } D_1 \text{ and } D_4 \text{ gates on two qubits with H gates}$$

**Proof:**

$$\begin{aligned}
& \underline{(\text{def})} \quad \text{[Diagram with 4 qubits, 8 H gates, 4 S gates, and 2 D gates]} \\
& \underline{(2)} \quad \text{[Diagram with 4 qubits, 8 H gates, 4 S gates]} \\
& \underline{(2)} \quad \text{[Diagram with 4 qubits, 8 H gates, 4 S gates]} \\
& \underline{(2)} \quad \text{[Diagram with 4 qubits, 8 H gates, 4 S gates]} \\
& \underline{(2)} \quad \text{[Diagram with 4 qubits, 8 H gates, 4 S gates]} \\
& \underline{(2)} \quad \text{[Diagram with 4 qubits, 8 H gates, 4 S gates]} \\
& \underline{(20)} \quad \text{[Diagram with 4 qubits, 8 H gates, 4 S gates]} \\
& \underline{(2)} \quad \text{[Diagram with 4 qubits, 8 H gates, 4 S gates]} \\
& \underline{(11)} \quad \text{[Diagram with 4 qubits, 8 H gates, 4 S gates]} \\
& \underline{(19)} \quad \text{[Diagram with 4 qubits, 8 H gates, 4 S gates]} \\
& \underline{(2)} \quad \text{[Diagram with 4 qubits, 8 H gates, 4 S gates]} \\
& \underline{(\text{inv})} \quad \text{[Diagram with 4 qubits, 8 H gates, 4 S gates]} \\
& \underline{(2)} \quad \text{[Diagram with 4 qubits, 8 H gates, 4 S gates]}
\end{aligned}$$

(def) 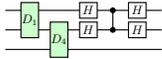

### 3.90 Equation

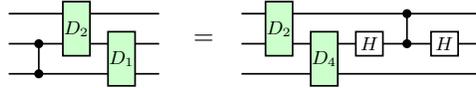

**Proof:**

(def) 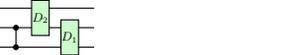

(18) 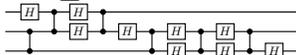

(2) 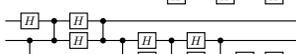

(inv) 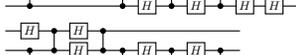

(2) 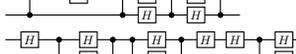

(19) 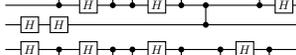

(11) 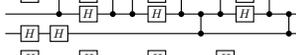

(2) 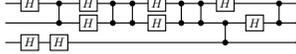

(19) 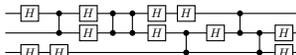

(13) 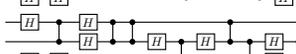  $\cdot \omega^{-1}$

(15) 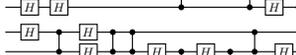  $\cdot \omega^{-2}$

(7) 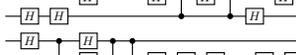

(2) 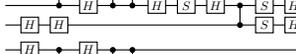

(12) 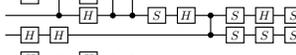

(16) 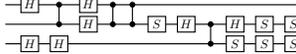

(2) 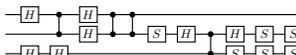

(12) 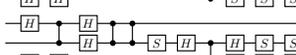

(16) 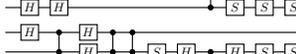

(2) 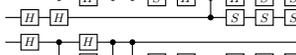

(12) 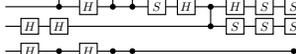

(16) 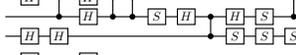

(2) 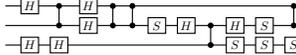

(12) 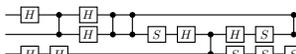

(16) 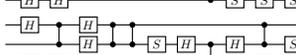

(2) 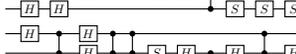

(14) 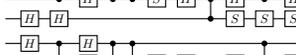

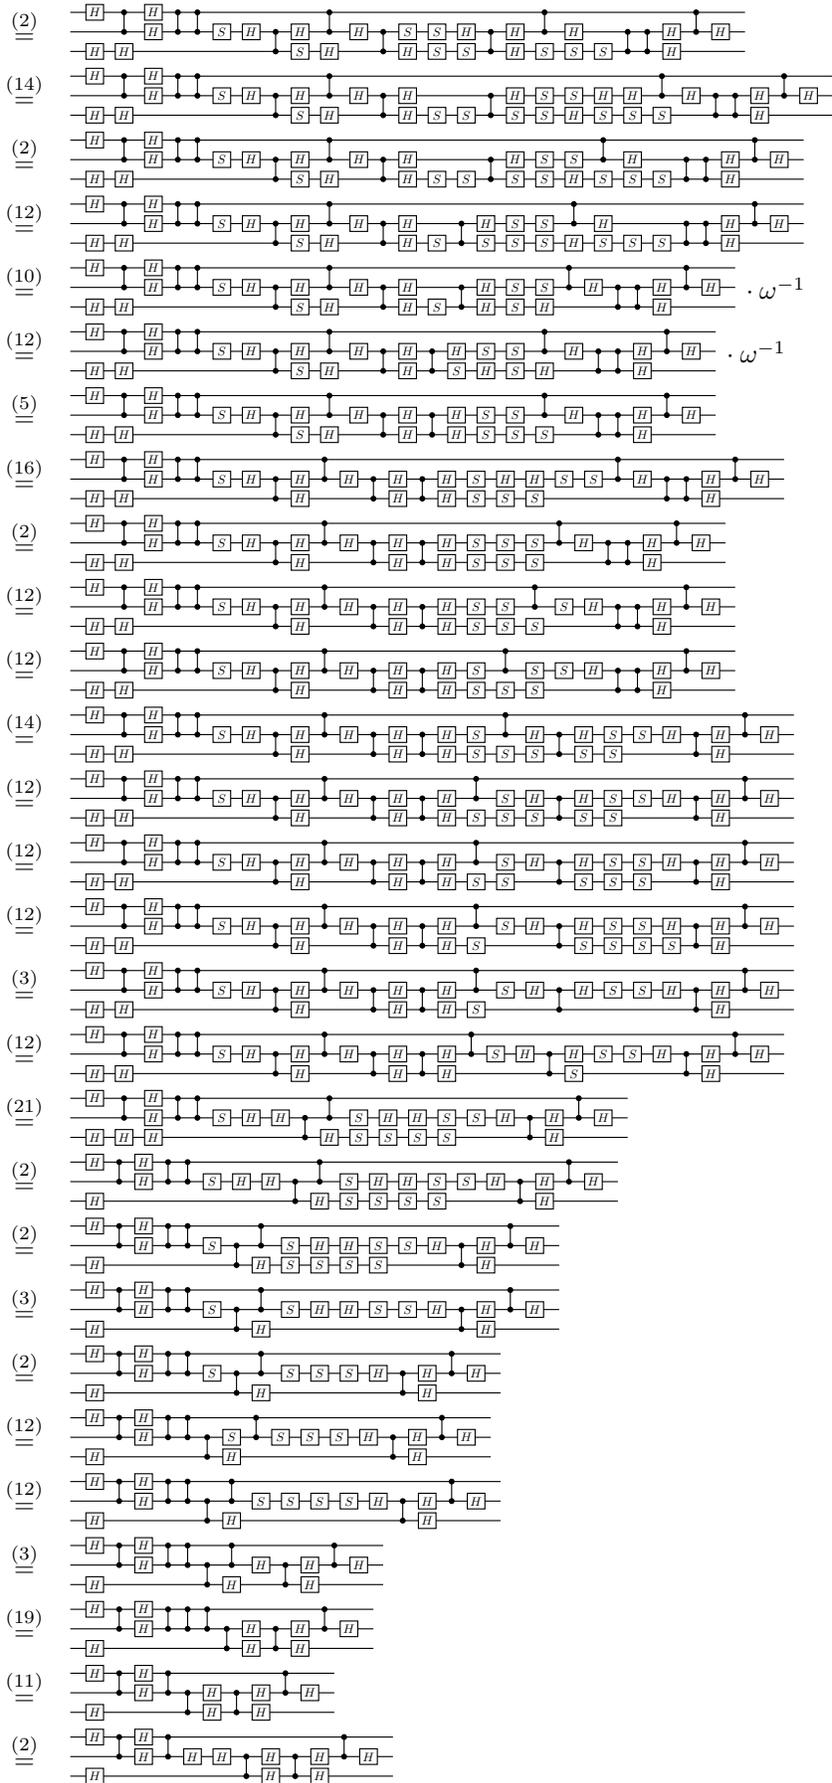

(def)

### 3.91 Equation

**Proof:**

(def)

(2)

(11)

(19)

(3)

(12)

(3)

(12)

(12)

(3)

(2)

(3)

(2)

(14)

(7)  $\cdot \omega^{-2}$

(13)  $\cdot \omega^{-1}$

(12)  $\cdot \omega^{-1}$

(2)  $\cdot \omega^{-1}$

(15)

(11)

(19)

(10)  $\cdot \omega$

(4)

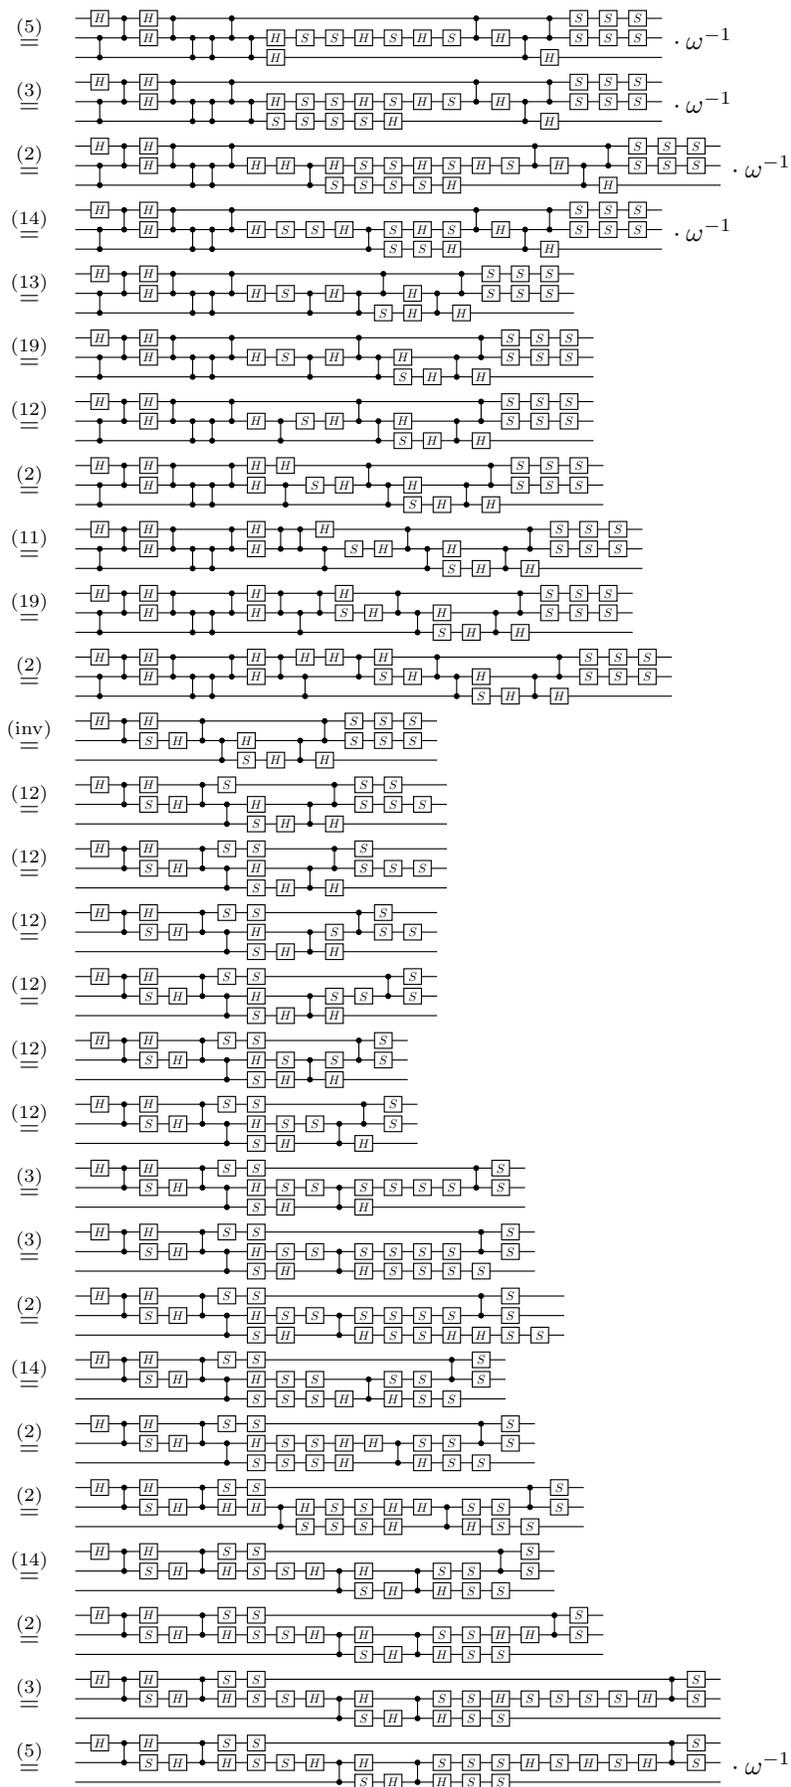

$$\begin{aligned}
& \underline{(2)} \quad \text{Diagram 1} \cdot \omega^{-1} \\
& \underline{(17)} \quad \text{Diagram 2} \cdot \omega^{-1} \\
& \underline{(12)} \quad \text{Diagram 3} \cdot \omega^{-1} \\
& \underline{(2)} \quad \text{Diagram 4} \cdot \omega^{-1} \\
& \underline{(3)} \quad \text{Diagram 5} \cdot \omega^{-1} \\
& \underline{(5)} \quad \text{Diagram 6} \cdot \omega^{-2} \\
& \underline{(17)} \quad \text{Diagram 7} \cdot \omega^{-2} \\
& \underline{(12)} \quad \text{Diagram 8} \cdot \omega^{-2} \\
& \underline{(2)} \quad \text{Diagram 9} \cdot \omega^{-2} \\
& \underline{(1)} \quad \text{Diagram 10} \cdot \omega^6 \\
& \underline{\text{(def)}} \quad \text{Diagram 11} \cdot \omega^6
\end{aligned}$$

### 3.92 Equation

$$\text{Diagram A} = \text{Diagram B} \cdot \omega^7$$

**Proof:**

$$\begin{aligned}
& \underline{\text{(def)}} \quad \text{Diagram 1} \\
& \underline{(2)} \quad \text{Diagram 2} \\
& \underline{(12)} \quad \text{Diagram 3} \\
& \underline{(17)} \quad \text{Diagram 4} \\
& \underline{(2)} \quad \text{Diagram 5} \\
& \underline{(11)} \quad \text{Diagram 6} \\
& \underline{(11)} \quad \text{Diagram 7} \\
& \underline{(19)} \quad \text{Diagram 8} \\
& \underline{(3)} \quad \text{Diagram 9} \\
& \underline{(12)} \quad \text{Diagram 10} \\
& \underline{(12)} \quad \text{Diagram 11} \\
& \underline{(12)} \quad \text{Diagram 12} \\
& \underline{(12)} \quad \text{Diagram 13}
\end{aligned}$$

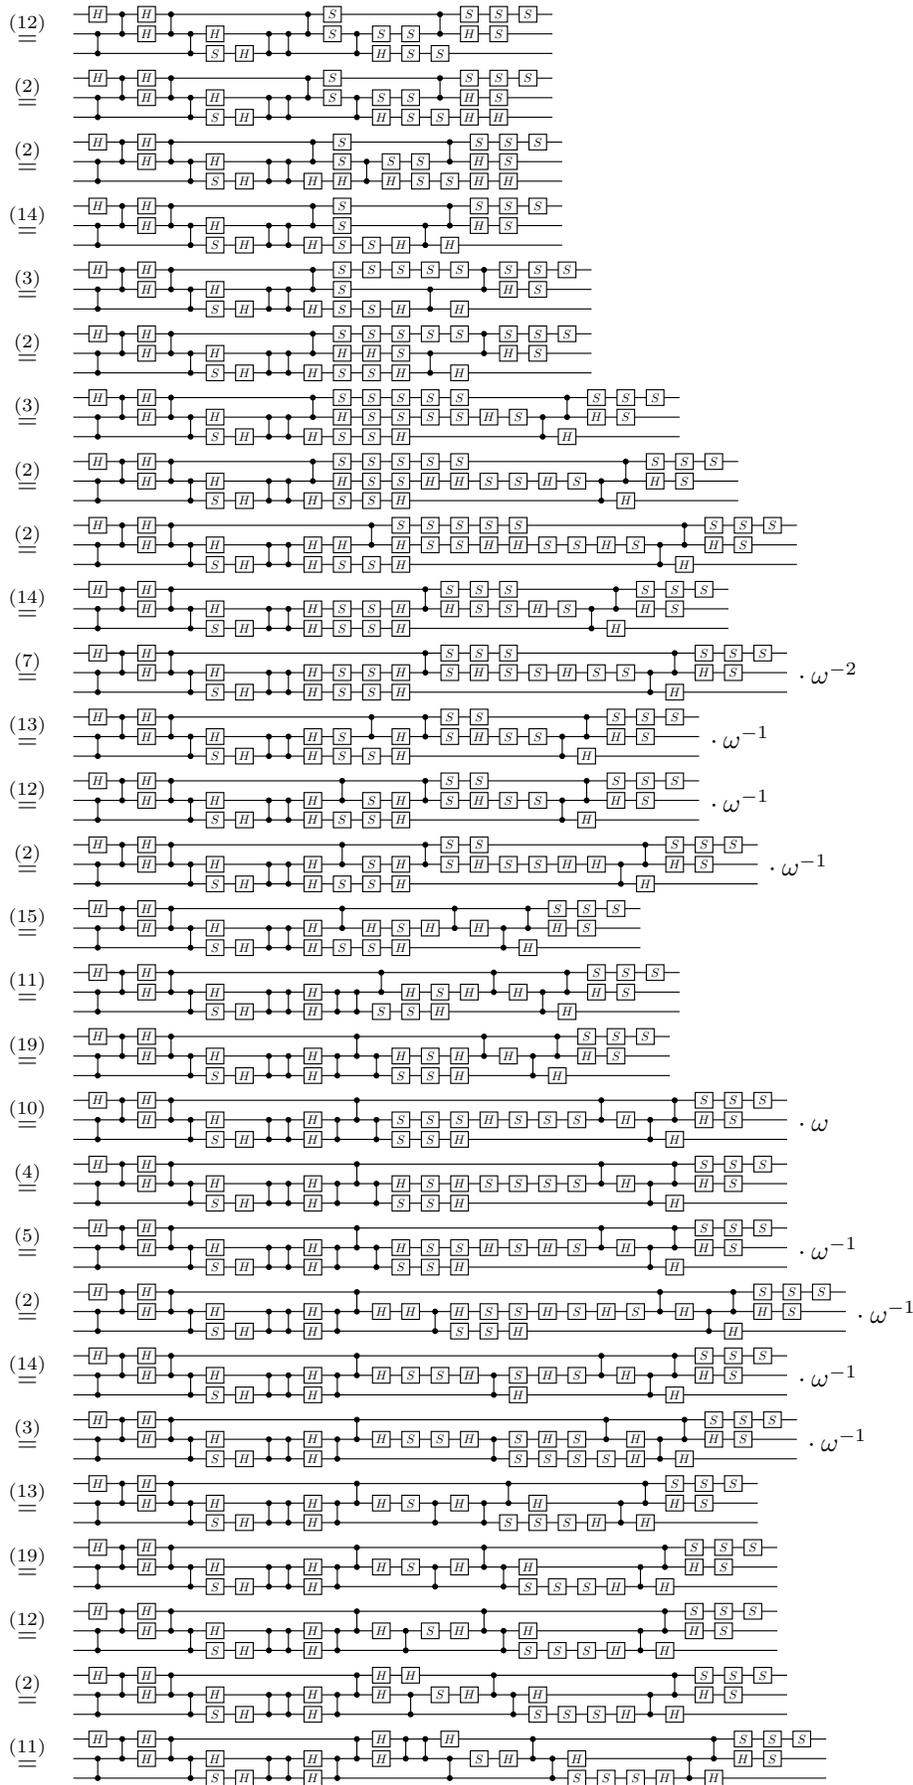





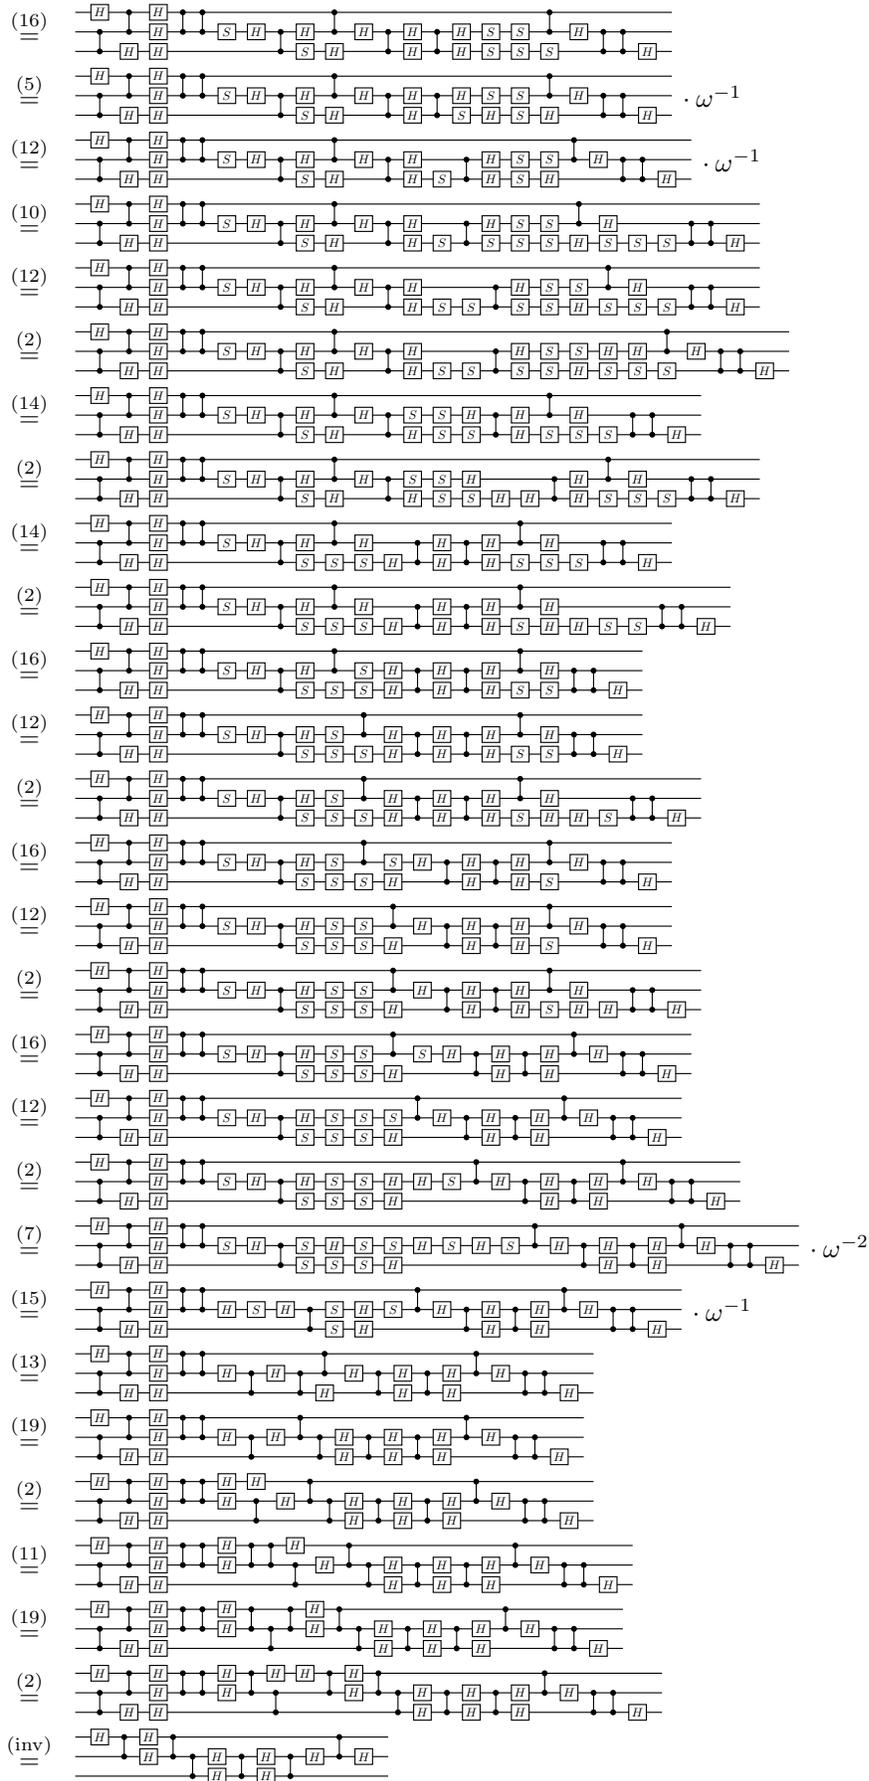

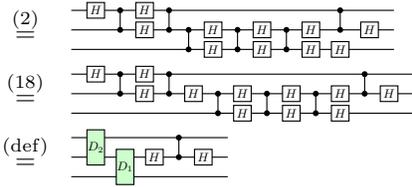

### 3.94 Equation

**Proof:**

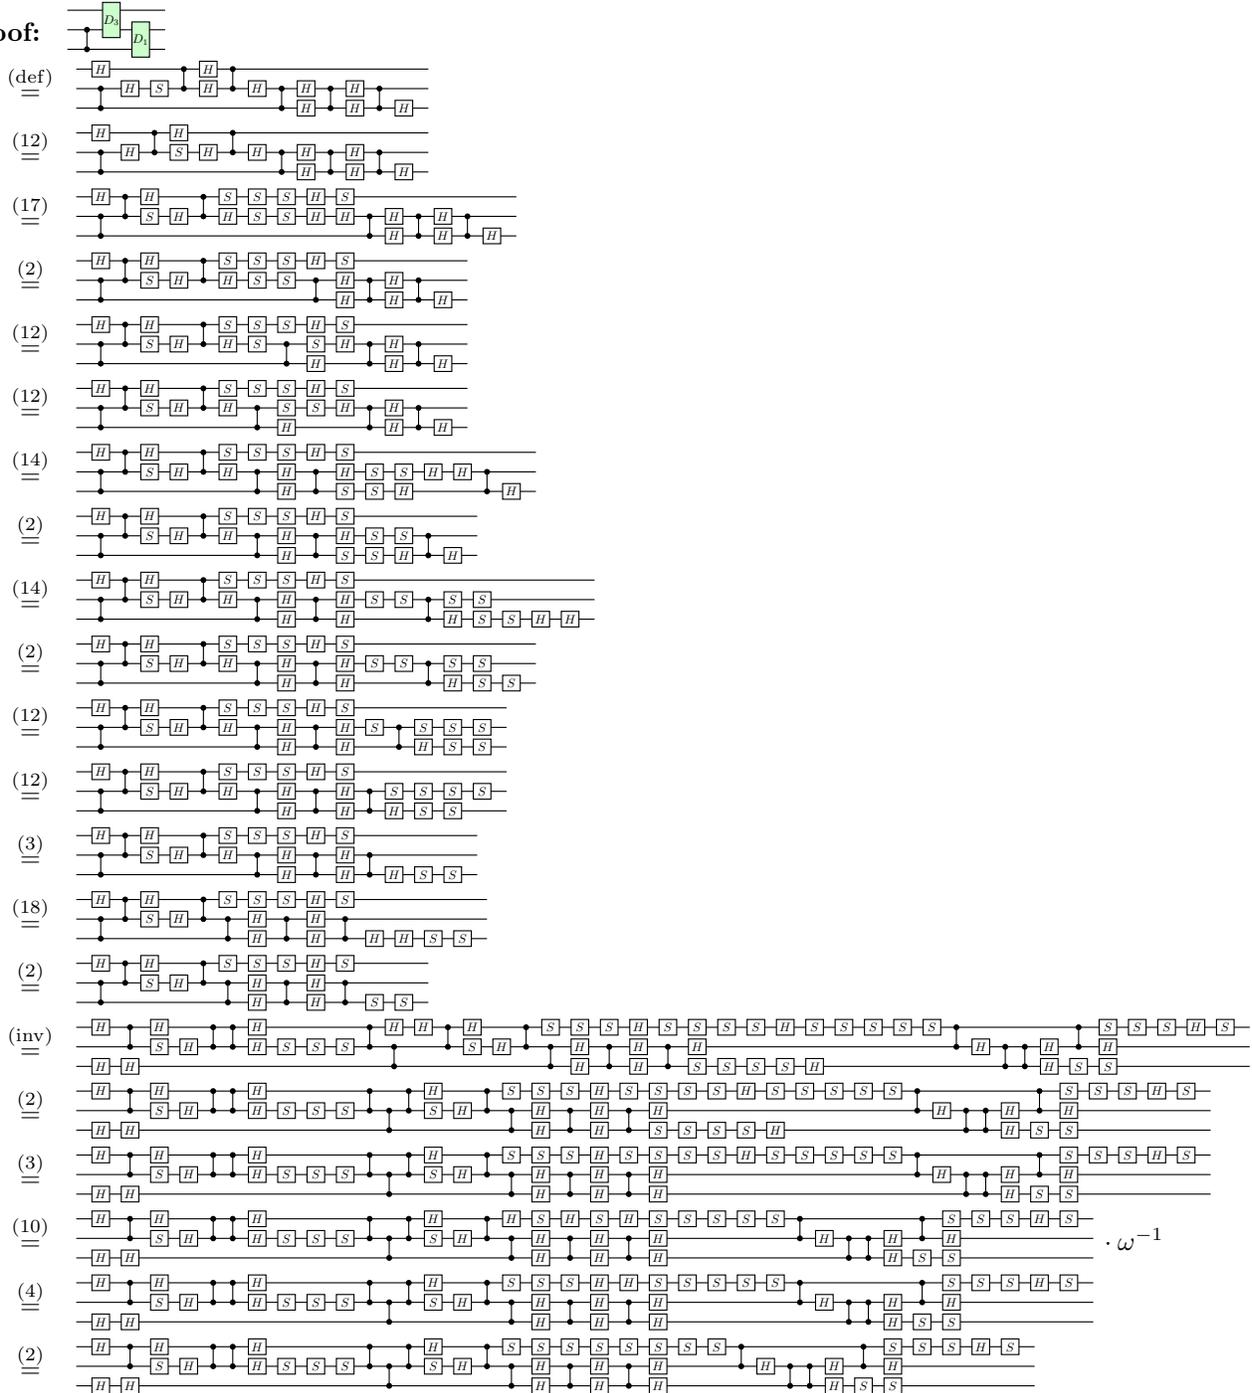

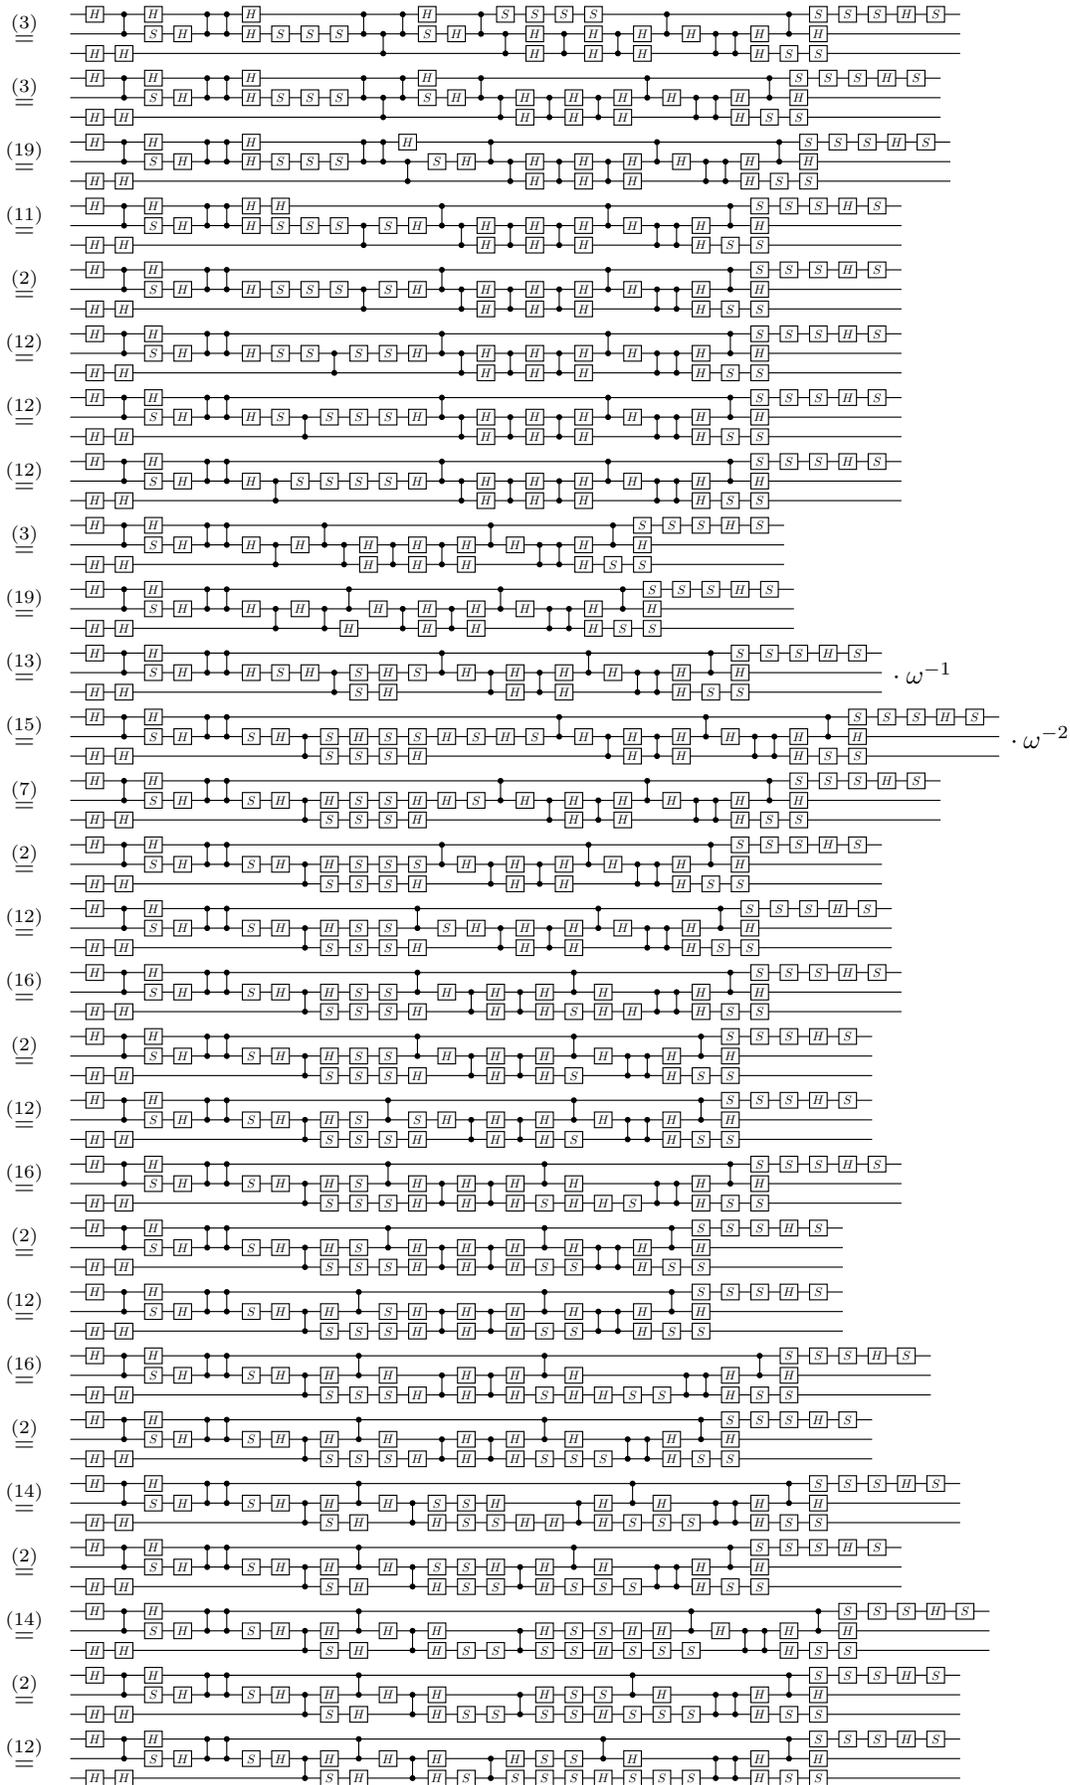

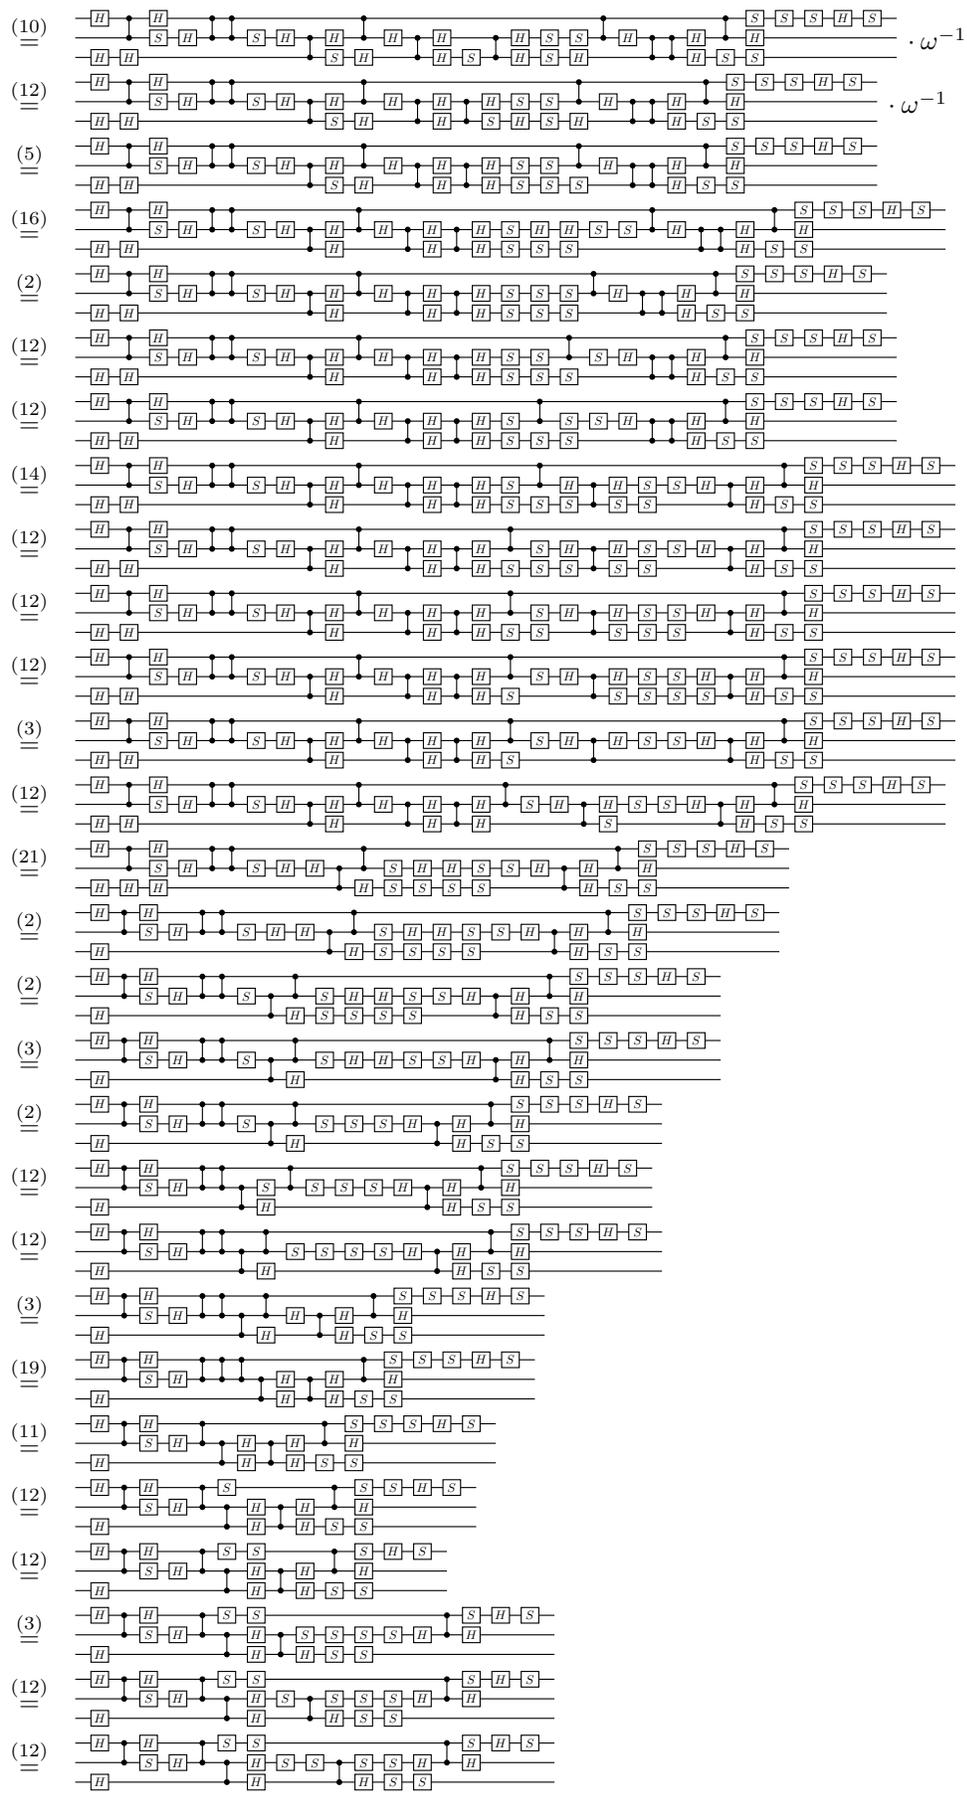

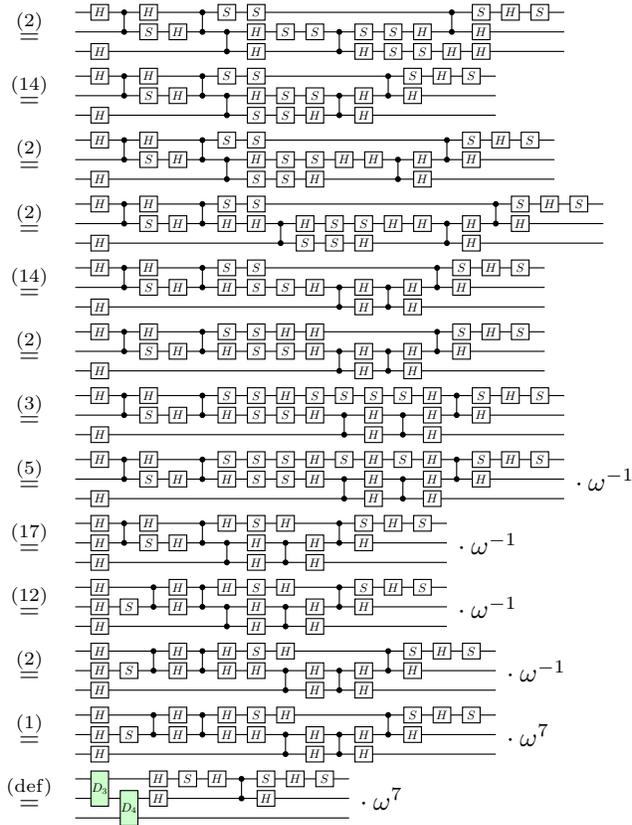

### 3.95 Equation

$$\begin{array}{c} \text{---} \\ \text{---} \end{array} \begin{array}{c} \boxed{D_3} \\ \boxed{D_2} \end{array} = \begin{array}{c} \text{---} \\ \text{---} \end{array} \begin{array}{c} \boxed{D_2} \\ \boxed{D_3} \\ \boxed{D_2} \end{array} \begin{array}{c} \boxed{H} \\ \boxed{S} \end{array} \begin{array}{c} \boxed{S} \\ \boxed{S} \end{array} \begin{array}{c} \boxed{H} \\ \boxed{S} \end{array} \begin{array}{c} \boxed{H} \\ \boxed{S} \end{array} \begin{array}{c} \boxed{H} \\ \boxed{S} \end{array} \begin{array}{c} \boxed{H} \\ \boxed{S} \end{array} \cdot \omega^7$$

**Proof:**

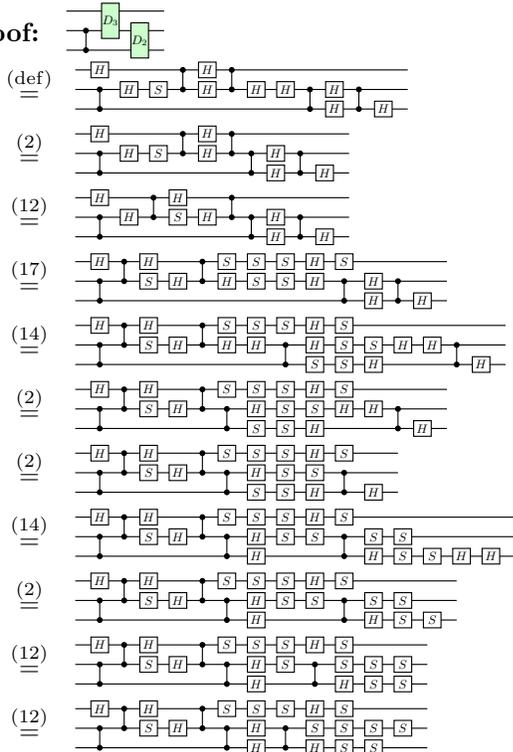



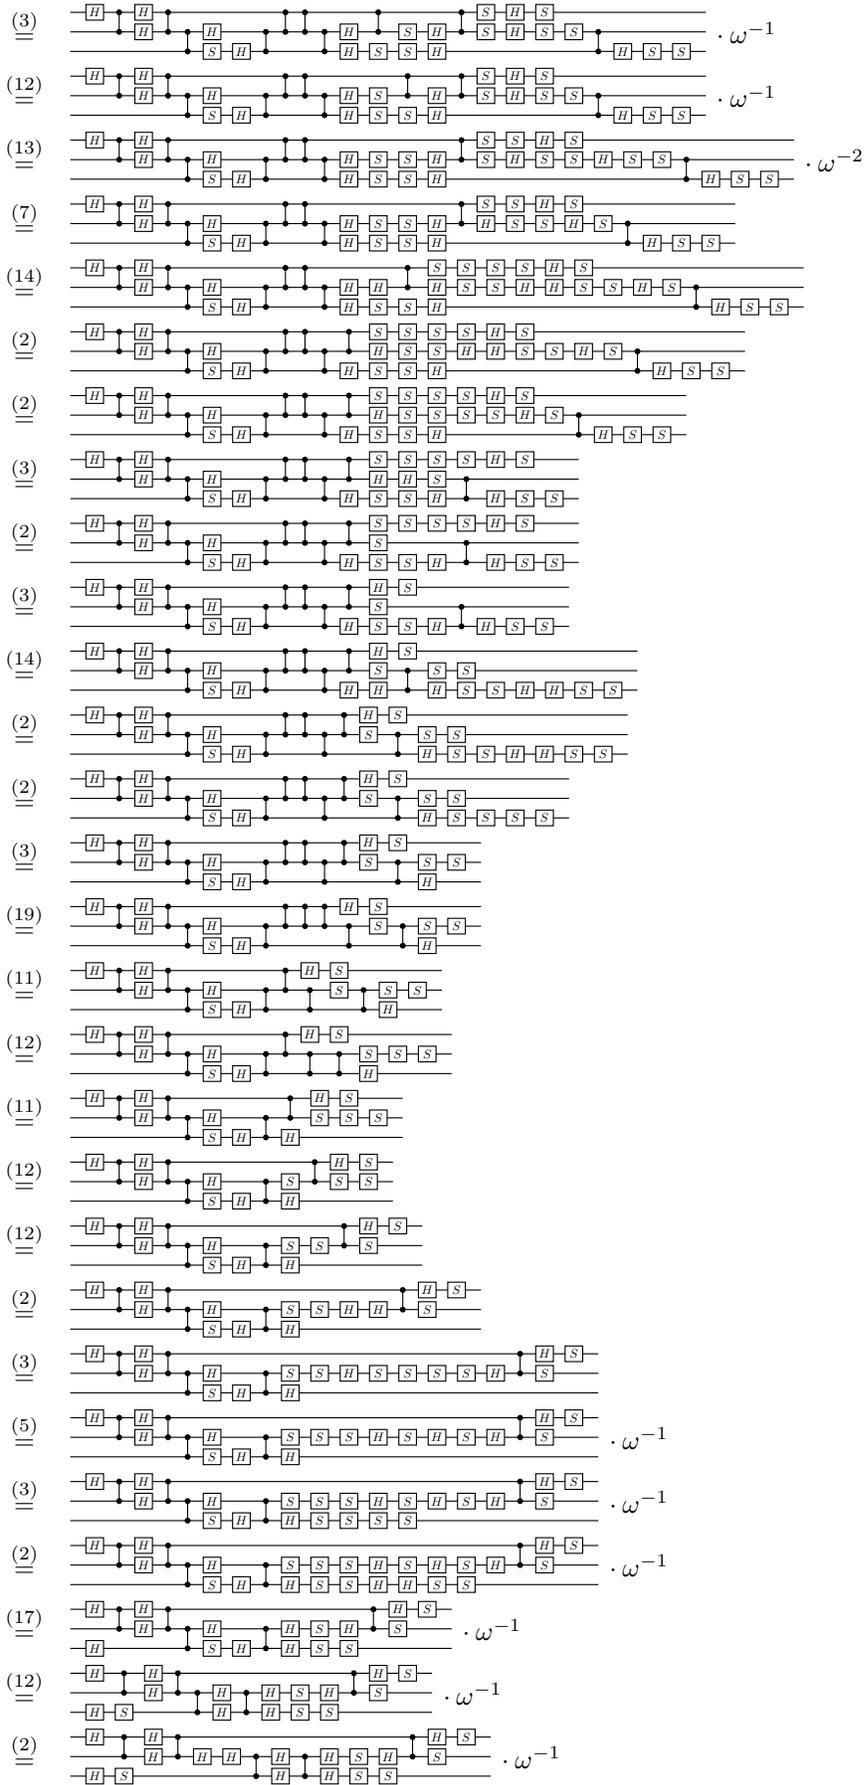



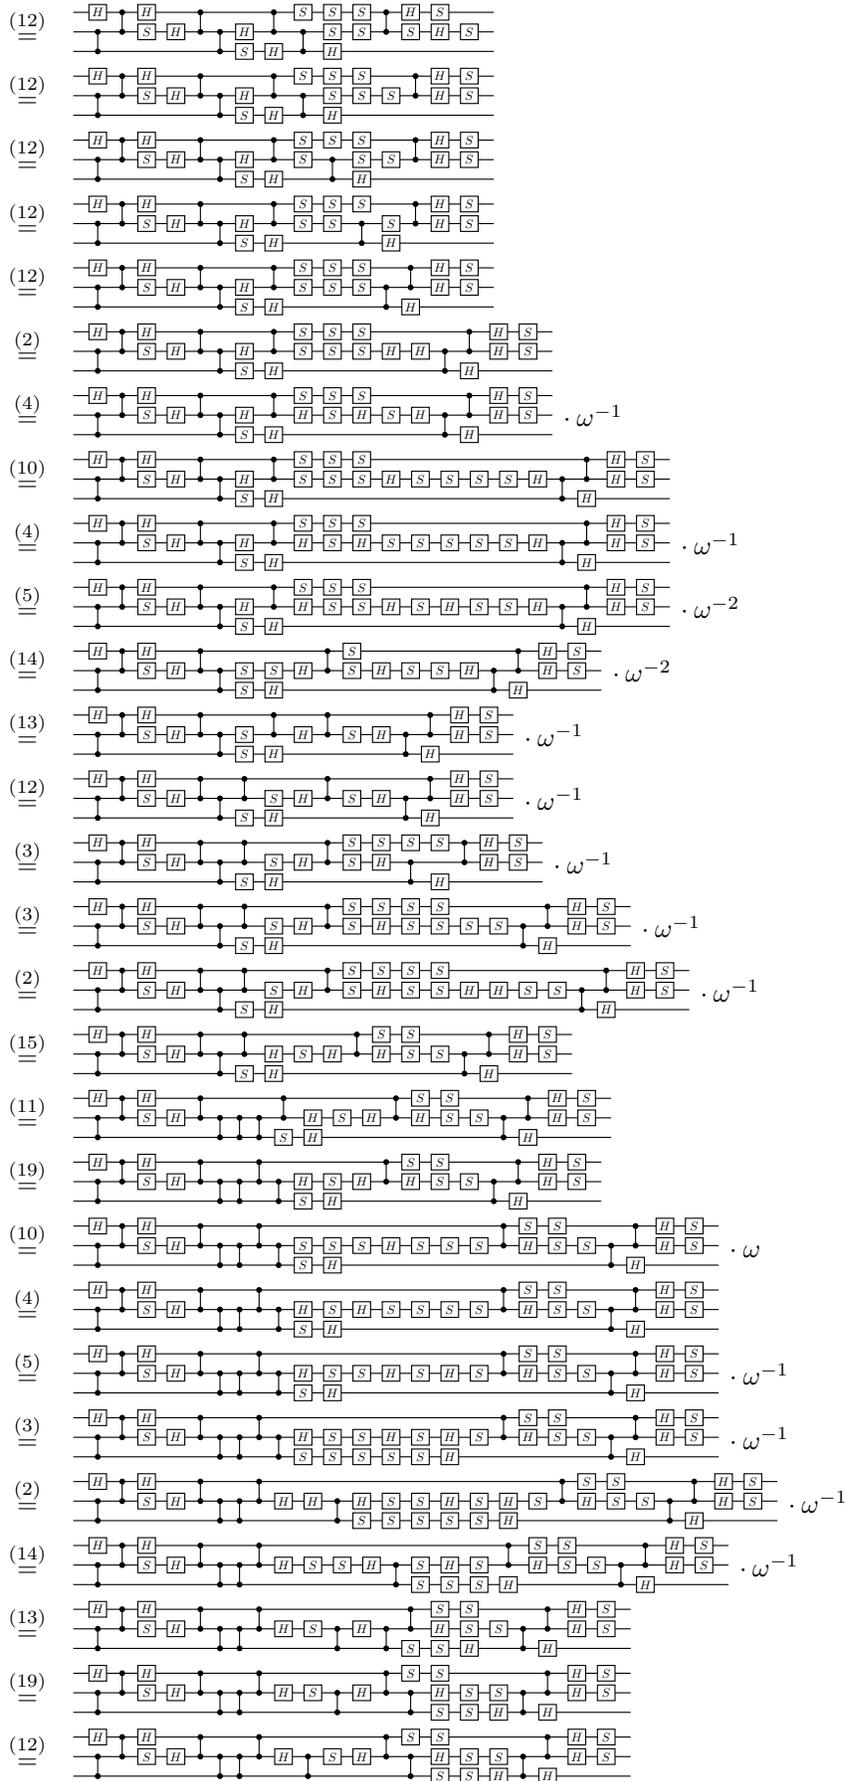

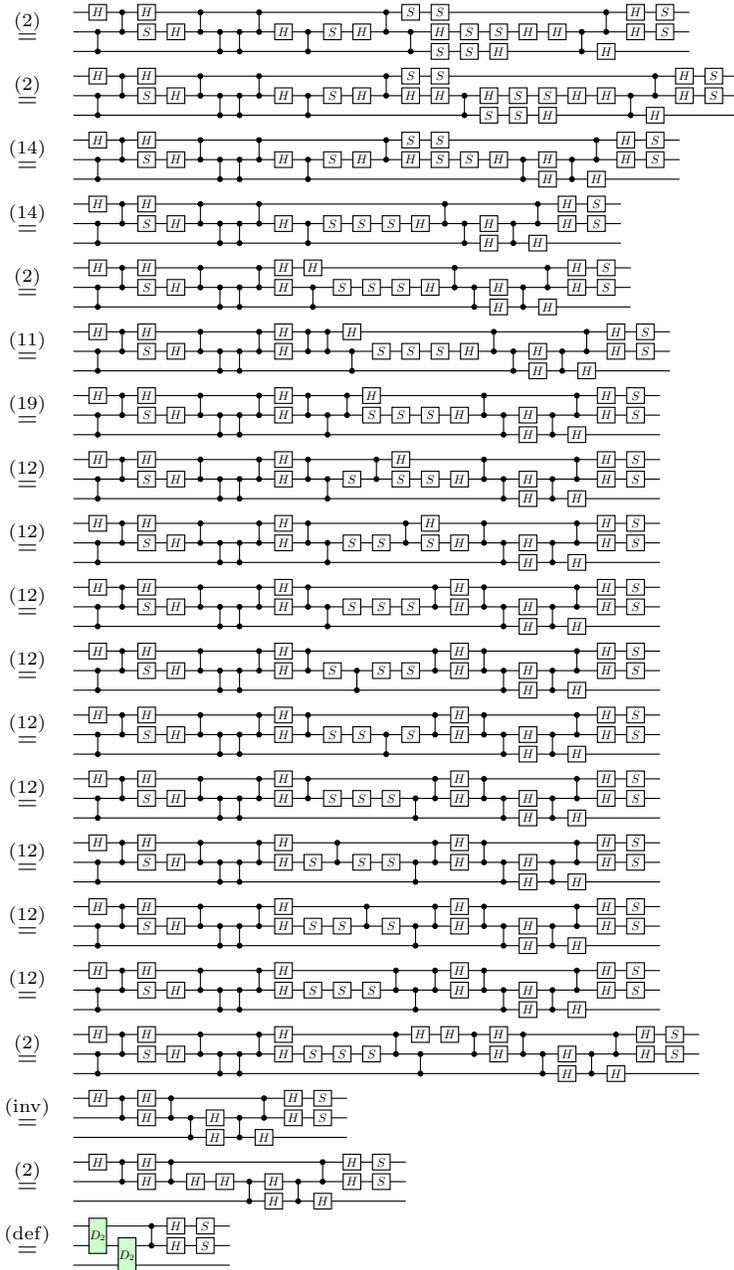

### 3.97 Equation

**Proof:**

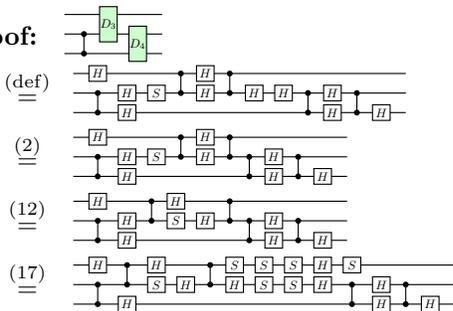

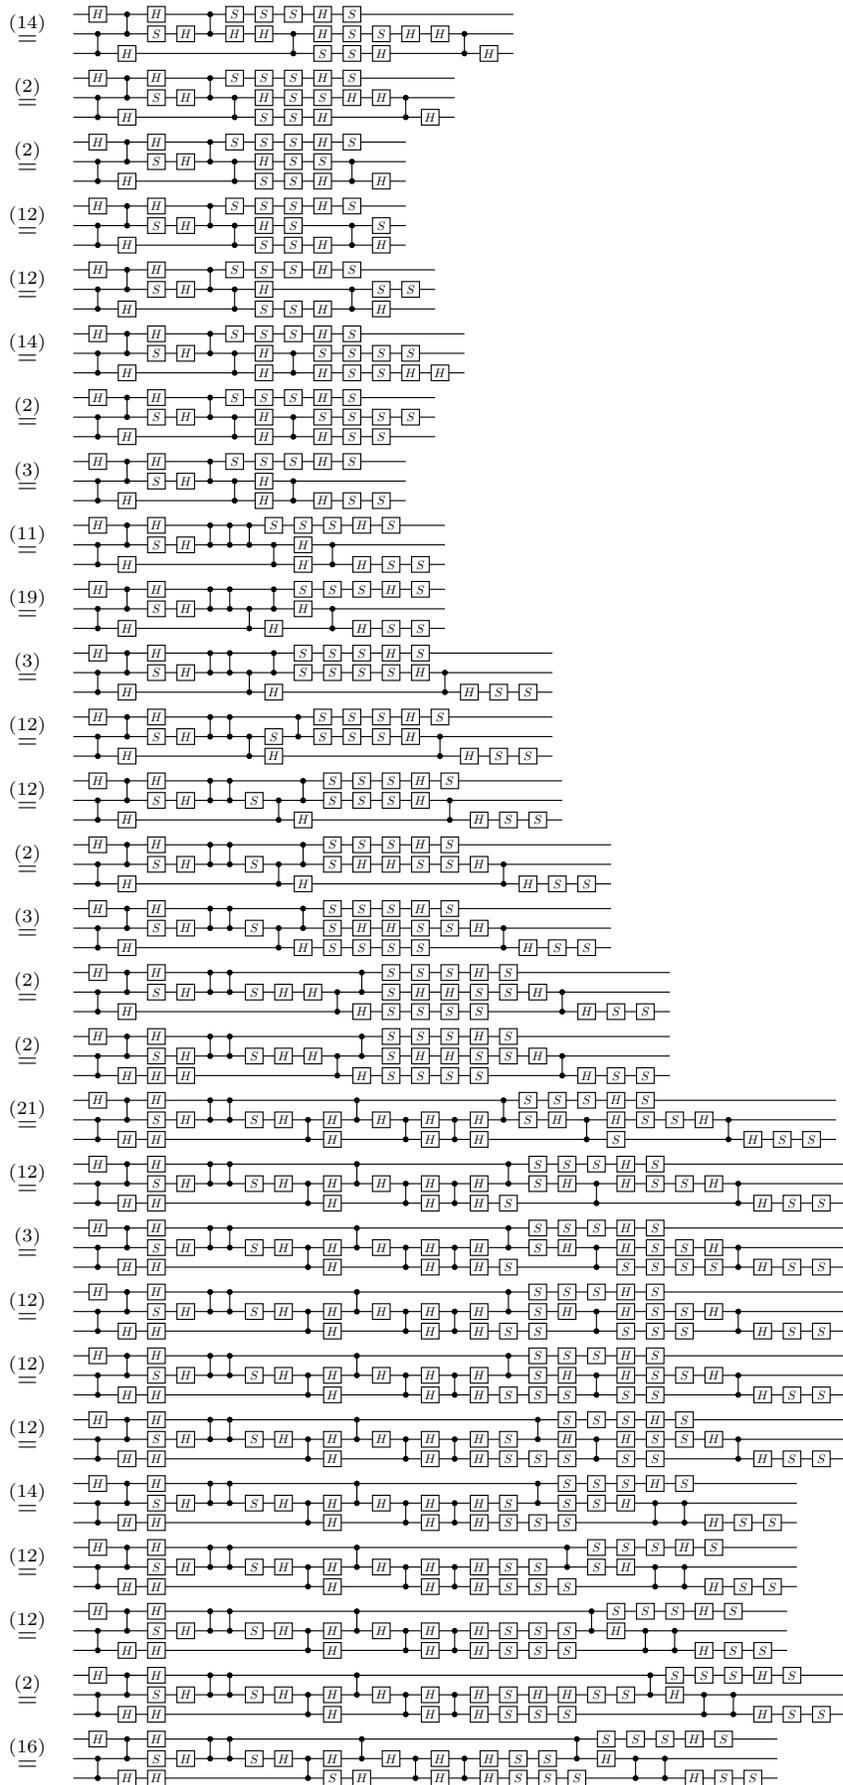

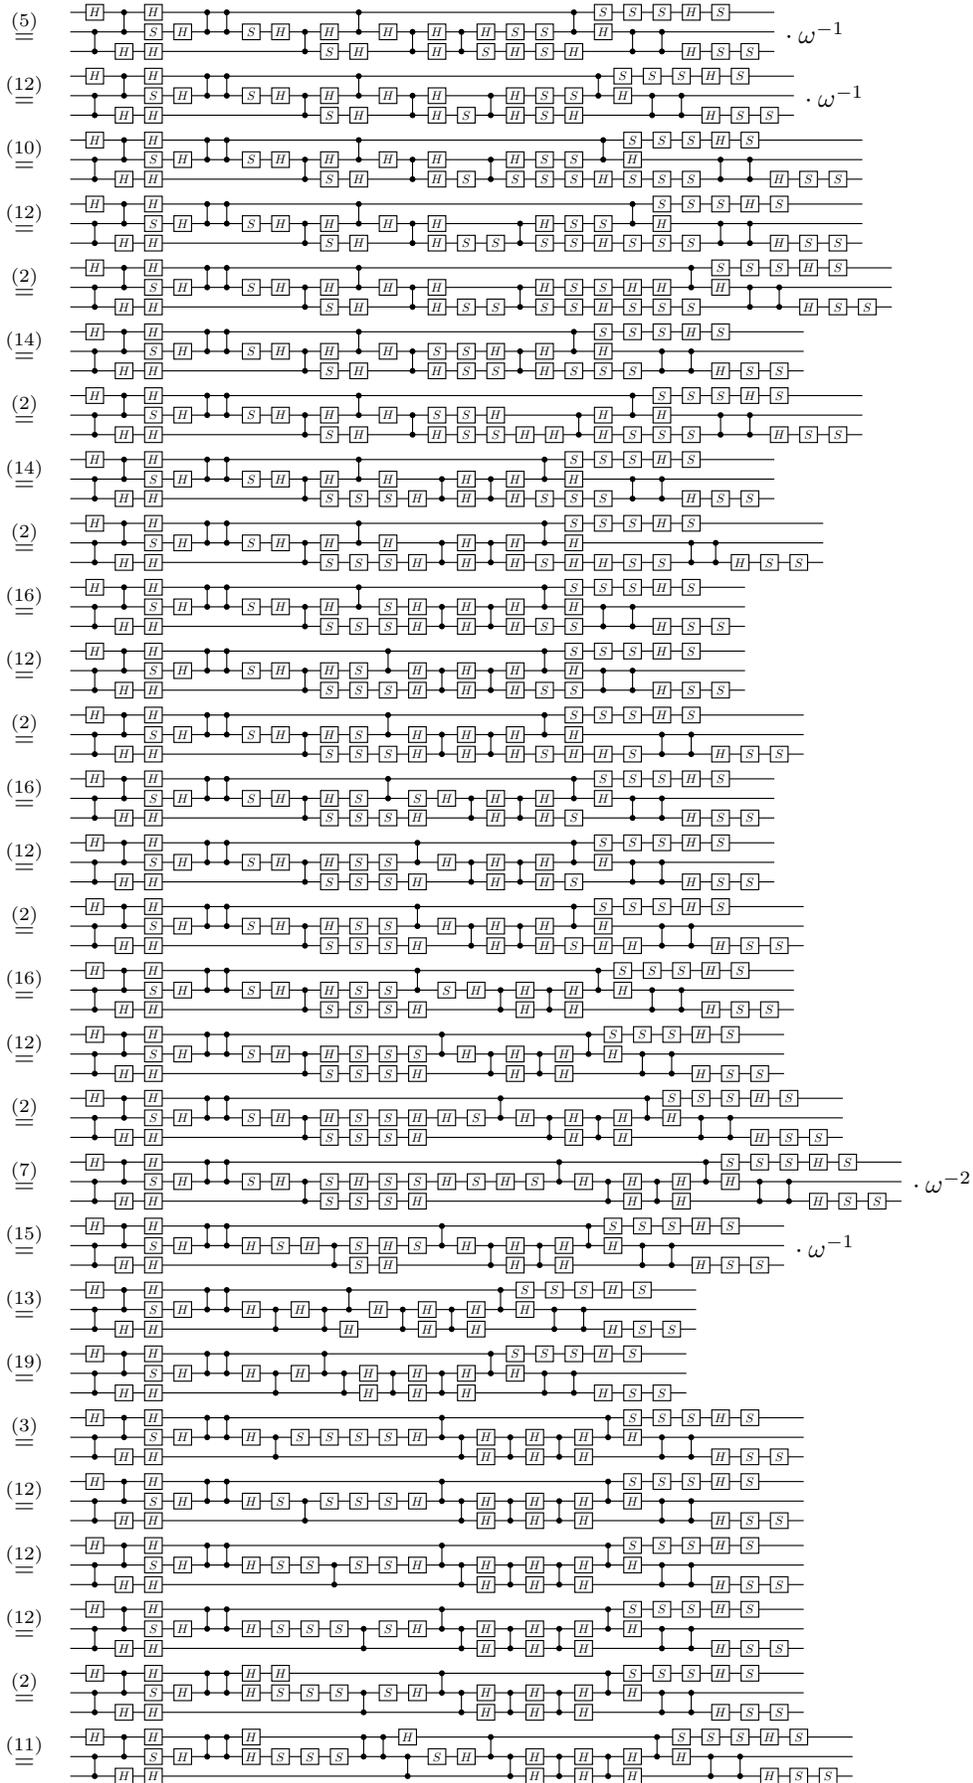





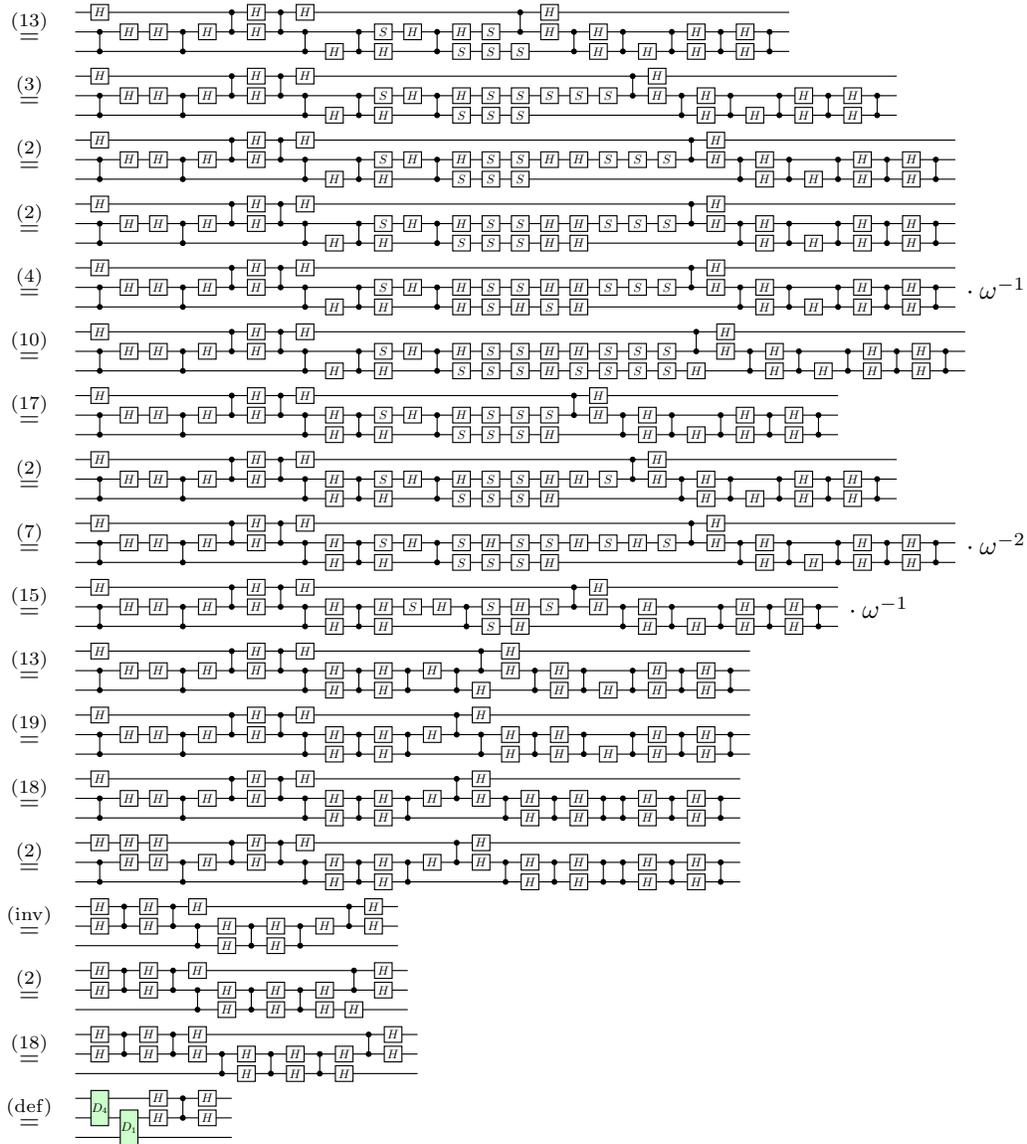

### 3.99 Equation

**Proof:**

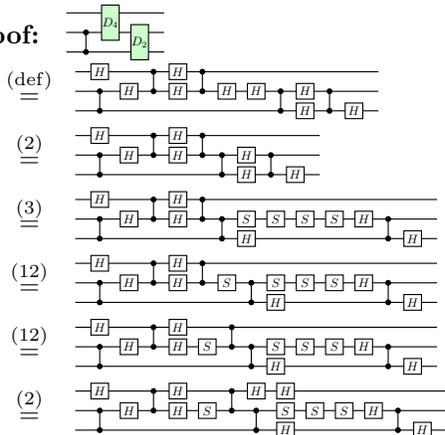

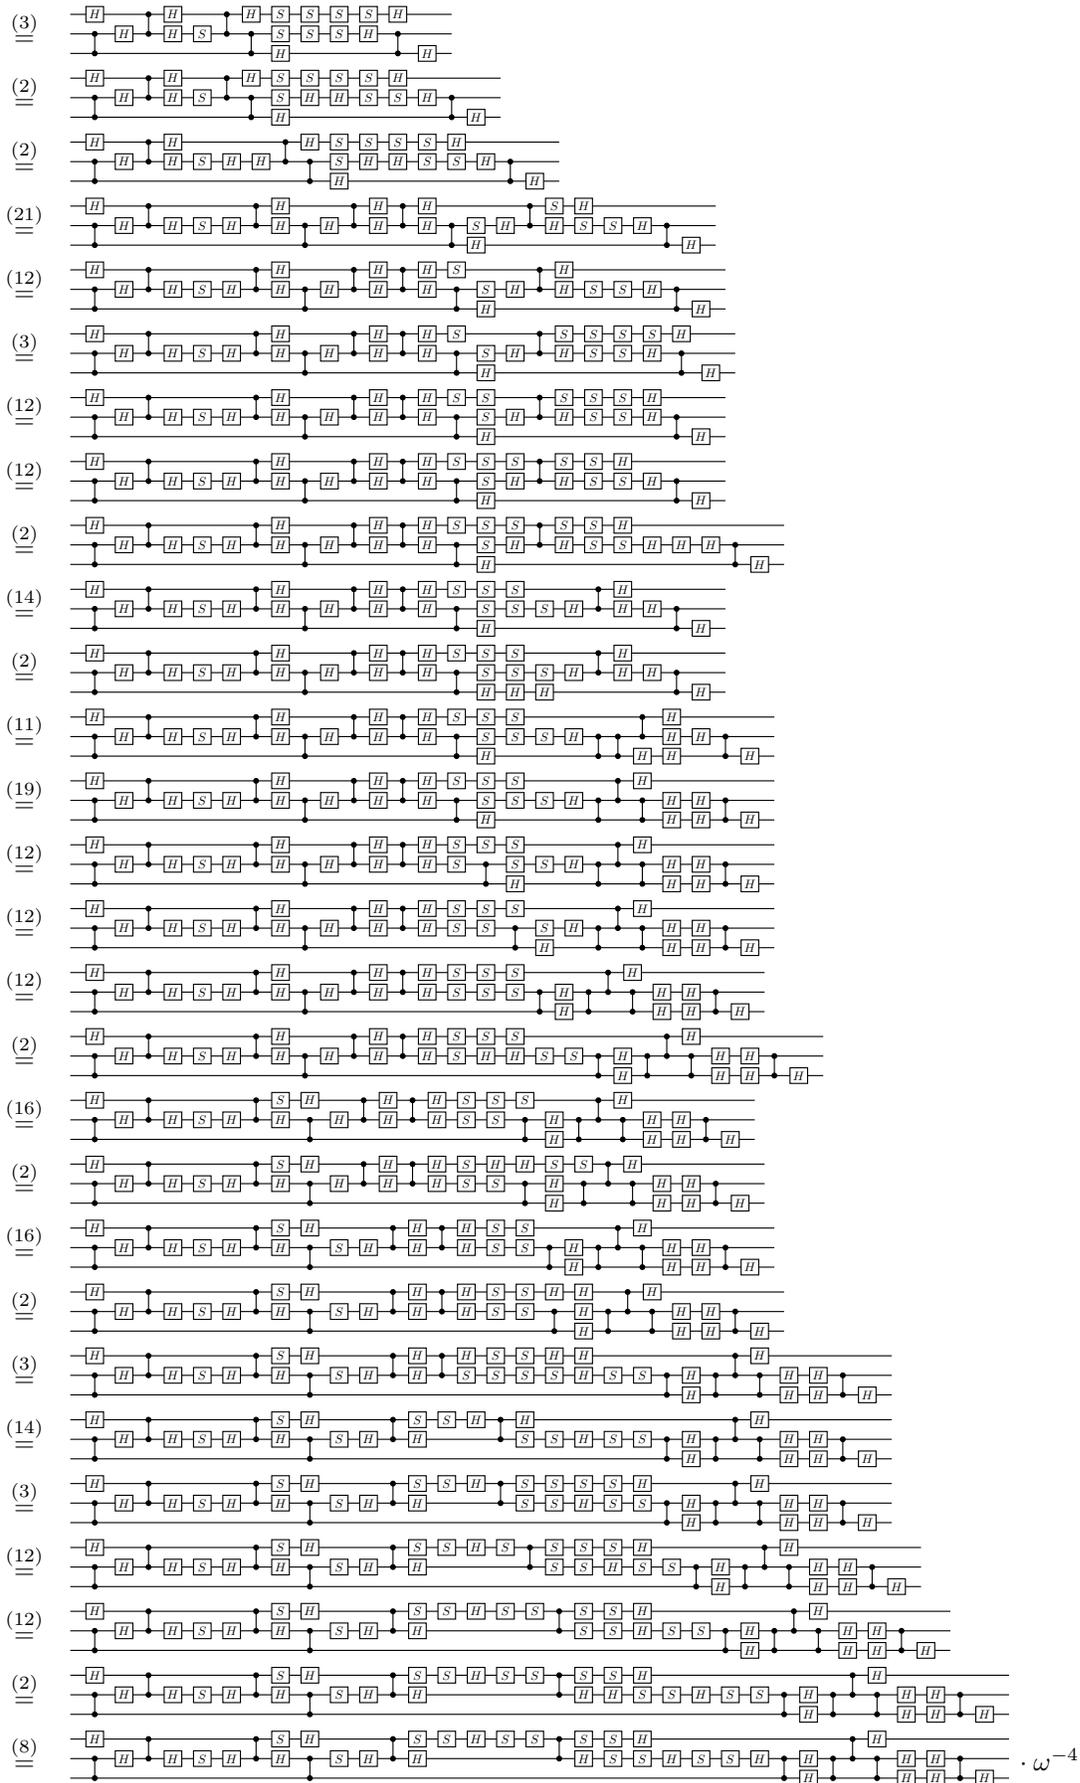



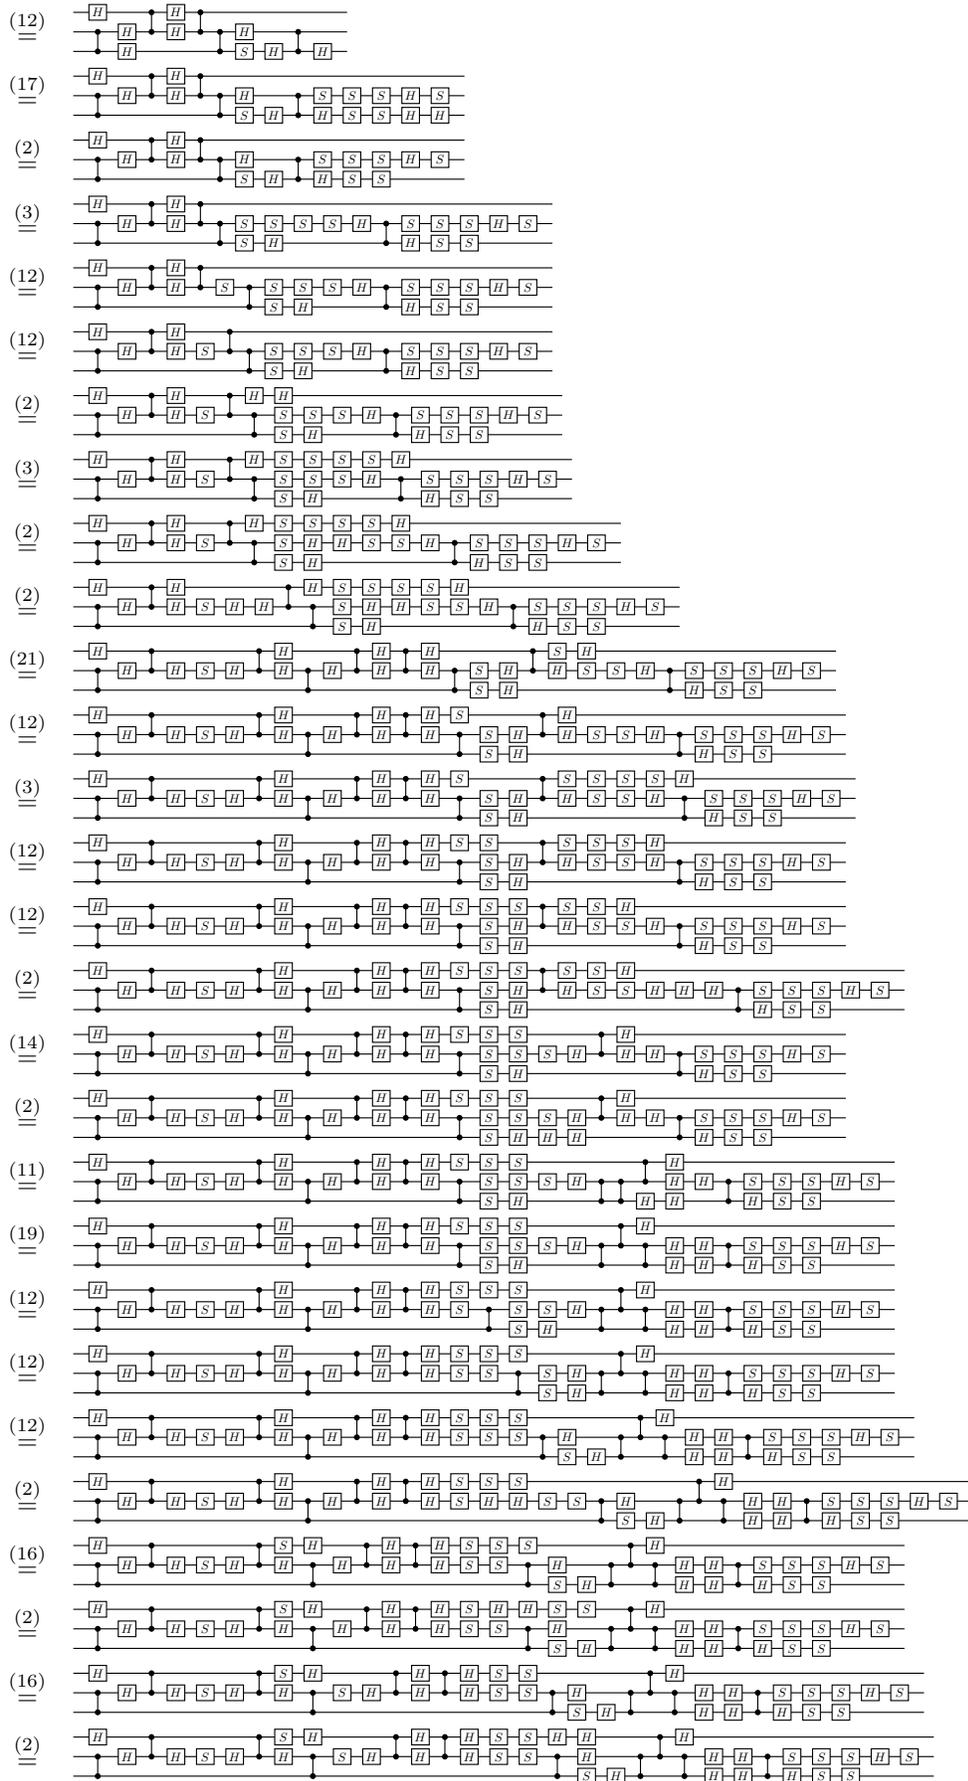



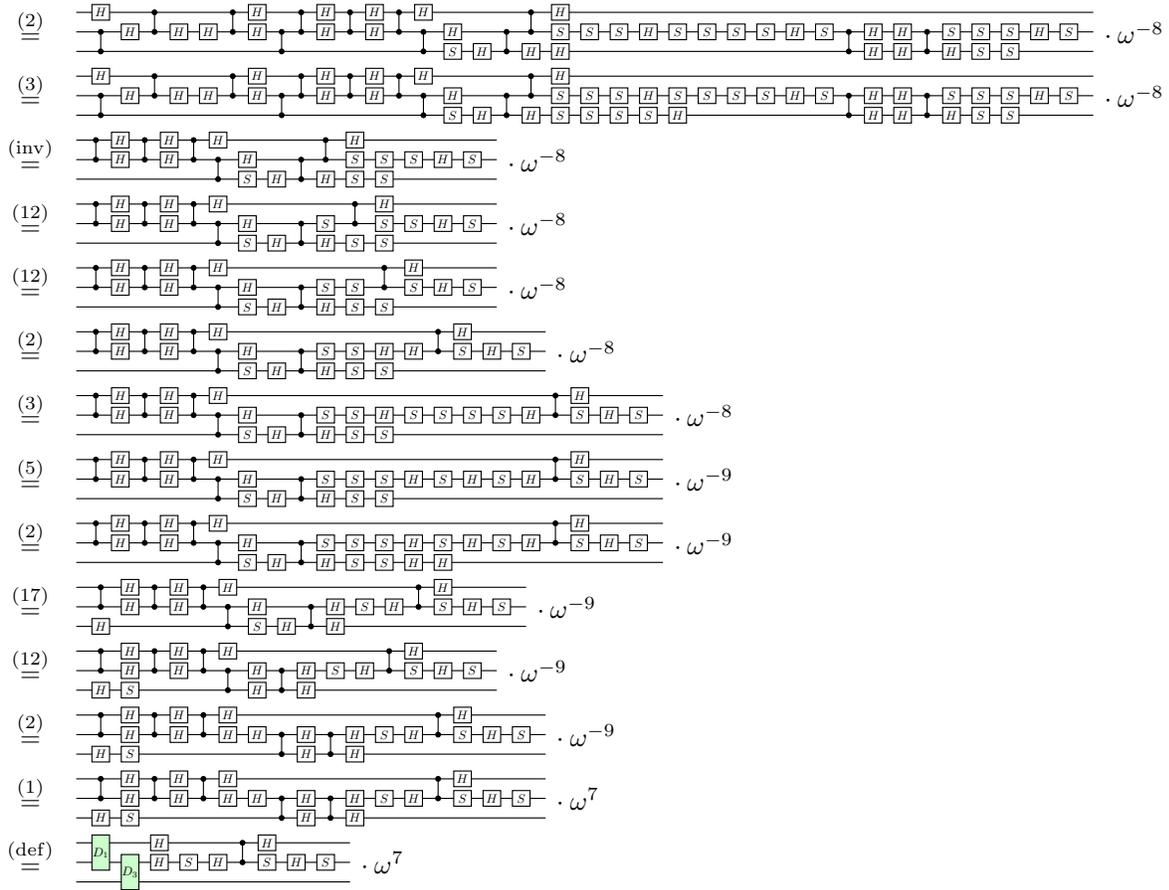

### 3.101 Equation

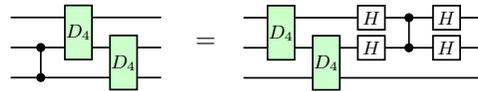

**Proof:**

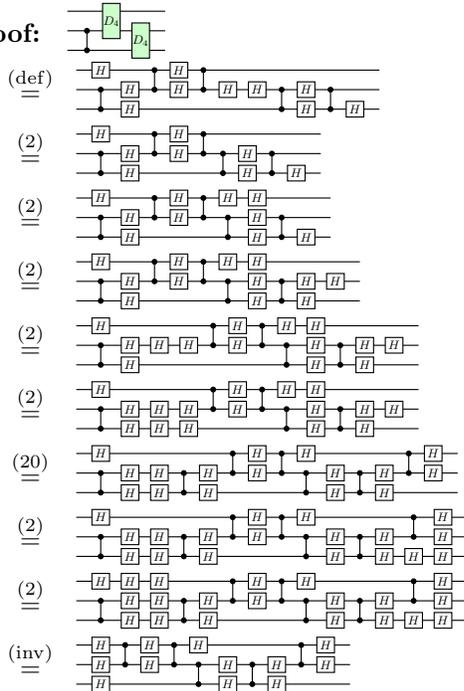

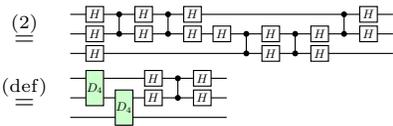

Supplement: Supplementary file 1 [file clifford-supplement.pdf]
